# Supplementary material for: On the classification of Kahler-Ricci solitons on Gorenstein del Pezzo surfaces
Source: arXiv:1705.02920 ancillary file (2018-03-10)
Supplement: Supplementary file 1 [file surfaces.pdf]

# surfaces

Hendrik Suess

05.05.2017

## 0.0.1 Gorenstein del Pezzo Surfaces

1. Degree 1,  $\text{Sing}=2D_4$
2. Degree 1,  $\text{Sing}=E_8$
3. Degree 1,  $\text{Sing}=E_7A_1$
4. Degree 1,  $\text{Sing}=E_6A_2$
5. Degree 2,  $\text{Sing}=2A_3A_1$
6. Degree 2,  $\text{Sing}=A_5A_2$
7. Degree 2,  $\text{Sing}=D_6A_1$
8. Degree 2,  $\text{Sing}=E_7$
9. Degree 2,  $\text{Sing}=E_6$
10. Degree 2,  $\text{Sing}=2A_3$
11. Degree 2,  $\text{Sing}=D_5A_1$
12. Degree 2,  $\text{Sing}=3A_1D_4$
13. Degree 3,  $\text{Sing}=A_5A_1$
14. Degree 3,  $\text{Sing}=E_6$
15. Degree 3,  $\text{Sing}=A_4A_1$
16. Degree 3,  $\text{Sing}=2A_2A_1$
17. Degree 3,  $\text{Sing}=D_5$
18. Degree 3,  $\text{Sing}=2A_2$
19. Degree 3,  $\text{Sing}=D_4$
20. Degree 3,  $\text{Sing}=A_32A_1$

- 
21. Degree 4, Sing= $D_5$
  22. Degree 4, Sing= $A_3A_1$
  23. Degree 4, Sing= $D_4$
  24. Degree 4, Sing= $A_4$
  25. Degree 4, Sing= $3A_1$
  26. Degree 4, Sing= $A_3$
  27. Degree 4, Sing= $2A_1$
  28. Degree 4, Sing= $A_2A_1$
  29. Degree 5, Sing= $A_4$
  30. Degree 5, Sing= $A_3$
  31. Degree 5, Sing= $A_2$
  32. Degree 5, Sing= $A_1$
  33. Degree 6, Sing= $A_2$
  34. Degree 6, Sing= $A_1$
- 

No. 2: Degree 1 / Singularity type  $E_8$ .

The combinatorial data is given by  $\square = [-1, 5]$  and  $\Phi_0(u) = \min\{\frac{u-4}{5}, 0\}$ ,  $\Phi_\infty(u) = \frac{u-2}{3}$ ,  $\Phi_1(u) = -\frac{u+1}{2}$

```
# We are working with interval arithmetic with precision of 26 bit
# this fixes the precision e.g. for evaluations of exponential \
  functions
```

```
RIF=RealIntervalField(26)
```

```
# The base polytope/interval
B=[-1,5]
```

```
# 3 PL functions on the interval
Phi1(u)=min_symbolic((u-4)/5,0)
Phi2(u)=1/3*u-2/3
Phi3(u)=-1/2*u-1/2
```

```
# the degree of \bar Phi
degPhi=Phi1+Phi2+Phi3+2
```

```
print "The combinatorial data"
show(B)
```

---

```
show(Phi1)
show(Phi2)
show(Phi3)
```

The combinatorial data

$$[-1, 5]$$

$$u \mapsto \min\left(\frac{1}{5}u - \frac{4}{5}, 0\right)$$

$$u \mapsto \frac{1}{3}u - \frac{2}{3}$$

$$u \mapsto -\frac{1}{2}u - \frac{1}{2}$$

Step (i) obtain a closed form for  $F_{X,\xi}(1)$

For this we have to analytically solve the integral  $\int_{\square} u \deg \bar{\Phi}(u) e^{\xi u} du$ .

```
# The integral can be solved symbolically:
```

```
F(xi)=integral(degPhi(u)*u*exp(xi*u),u,*B)
```

```
show(F(xi))
```

$$\frac{(5\xi - 2)e^{(5\xi)}}{6\xi^3} - \frac{(12(2\xi - 1)e^{(5\xi)} + \xi + 2)e^{(-\xi)}}{30\xi^3}$$

Step (ii) find an estimate for the soliton candidate vector field  $\xi$

```
# Solve numerically
```

```
sol=find_root(F, -10, 10)
```

```
print "Numerical solution:", sol
```

```
# Choose upper and lower bound and
```

```
# hope that the exact solution lies in between
```

```
xi_1=sol-0.0000001
```

```
xi_2=xi_1+0.0000002
```

```
#define a real value xi0 between xi_1 and xi_2
```

```
# representing the exact solution
```

```
xi0=RIF(xi_1, xi_2)
```

```
# Check whether Intermediate value theorem guarantees a zero between
```

```
# xi_1 and xi_2, i.e evaluate F at xi_1 and xi_2 using interval \
arithmetic
```

```
if RIF(F(xi_1)) < 0 and RIF(F(xi_2)) > 0:
```

```
    print "Interval containing solution:", xi0.str(style='\
brackets')
```

Numerical solution: -1.9976195991

Interval containing solution: [-1.99761972 .. -1.99761947]

Step (iii) & (iv) obtain closed forms for  $DF_{\xi}(X_{y,0,1})$  and plug in the estimate for  $\xi$

For every choice of  $y \in \mathbb{P}^1$  we have to symbolically solve the integrals  $\int_{\square} e^{u\xi} \cdot \left( (1 + \Phi_y(u))^2 - (1 + \sum_{z \neq y} \Phi_z(u)) \right)$

which up to scaling with a positive constant coincide with  $DF_\xi(\mathcal{X}_{y,0,1})$ . Then we plug in the estimate for  $\xi$  into the resulting expression.

```
#check for positivity of the DF invariant for our vector field xi
print("Stability test for test configurations:")

#storage for DF values (as intervals)
IDF={}

DF1(xi)=integral(exp(xi*u)*((Phi1+1)(u)^2-(Phi3+Phi2+1)(u)^2)/2,u\
, -1,B[1])
IDF[1]=RIF(DF1(xi0)) # evaluate DF1 at xi0 using interval arithmetic
show(DF1(xi) >= IDF[1].lower())

DF2(xi)=integral(exp(xi*u)*((Phi2+1)(u)^2-(Phi1+Phi3+1)(u)^2)/2,u\
, -1,B[1])
IDF[2]=RIF(DF2(xi0))
show(DF2(xi) >= IDF[2].lower())

DF3(xi)=integral(exp(xi*u)*((Phi3+1)(u)^2-(Phi1+Phi2+1)(u)^2)/2,u\
, -1,B[1])
IDF[3]=RIF(DF3(xi0))
show(DF3(xi) >= IDF[3].lower())

DF4(xi)=integral(exp(xi*u)*((1)^2-(Phi3+Phi2+Phi1+1)(u)^2)/2,u, -1,B\
[1])
IDF[4]=RIF(DF4(xi0))
show(DF4(xi) >= IDF[4].lower())

if all([DF > 0 for DF in IDF.values()]):
    print("Surface is stable!")
else:
    if any([DF <= 0 for DF in IDF.values()]):
        print("Surface is not stable!")

    # print upper bound for destabilising DF value
    if IDF[1] <= 0: show(DF1(xi) <= IDF[1].upper())
    if IDF[2] <= 0: show(DF2(xi) <= IDF[2].upper())
    if IDF[3] <= 0: show(DF3(xi) <= IDF[3].upper())
    if IDF[4] <= 0: show(DF4(xi) <= IDF[4].upper())
    else:
        print("Cannot determine stability")
        # Note, that "not a > 0" does not imply "a <= 0" for \
intervals
```

Stability test for test configurations:

$$\frac{(6\xi - 1)e^{(5\xi)}}{36\xi^3} - \frac{(36(5\xi - 1)e^{(5\xi)} + 11)e^{(-\xi)}}{900\xi^3} \geq 0.01128570$$

---


$$\frac{(12\xi - 5)e^{(5\xi)}}{36\xi^3} - \frac{(18(15\xi - 8)e^{(5\xi)} + 19)e^{(-\xi)}}{900\xi^3} \geq 0.01949453$$

$$- \frac{(12\xi - 5)e^{(5\xi)}}{36\xi^3} + \frac{(12(25\xi - 13)e^{(5\xi)} + 30\xi + 31)e^{(-\xi)}}{900\xi^3} \geq 0.02975460$$

$$\frac{(6\xi - 1)e^{(5\xi)}}{36\xi^3} - \frac{(6(25\xi - 4)e^{(5\xi)} - 30\xi - 1)e^{(-\xi)}}{900\xi^3} \geq 0.06053484$$

Surface is stable!

---

No. 3: Degree 1 / Singularity type  $E_7A_1$ .

The combinatorial data is given by  $\square = [-1, 3]$  and  $\Phi_0(u) = \min\{\frac{u-2}{3}, 0\}$ ,  $\Phi_\infty(u) = \frac{u-3}{4}$ ,  $\Phi_1(u) = \frac{-u-1}{2}$

```
# We are working with interval arithmetic with precision of 26 bit
# this fixes the precision e.g. for evaluations of exponential \
  functions
```

```
RIF=RealIntervalField(26)
```

```
# The base polytope/interval
B=[-1,3]
```

```
# 3 PL functions on the interval
```

```
Phi1(u)=min_symbolic((u-2)/3,0)
```

```
Phi2(u)=1/4*u-3/4
```

```
Phi3(u)=-1/2*u-1/2
```

```
# the degree of \bar Phi
```

```
degPhi=Phi1+Phi2+Phi3+2
```

```
print "The combinatorial data"
```

```
show(B)
```

```
show(Phi1)
```

```
show(Phi2)
```

```
show(Phi3)
```

The combinatorial data

$[-1, 3]$

$u \mapsto \min\left(\frac{1}{3}u - \frac{2}{3}, 0\right)$

$u \mapsto \frac{1}{4}u - \frac{3}{4}$

$u \mapsto -\frac{1}{2}u - \frac{1}{2}$

Step (i) obtain a closed form for  $F_{X,\xi}(1)$

For this we have to analytically solve the integral  $\int_{\square} u \deg \bar{\Phi}(u) e^{\xi u} du$ .

```
# The integral can be solved symbolically:
```

```
F(xi)=integral(degPhi(u)*u*exp(xi*u),u,-1,B[1])
```

---

```
show(F(xi))

$$\frac{(3\xi - 2)e^{(3\xi)}}{4\xi^3} - \frac{(8(\xi - 1)e^{(3\xi)} + \xi + 2)e^{(-\xi)}}{12\xi^3}$$

```

Step (ii) find an estimate for the soliton candidate vector field  $\xi$

```
# Solve numerically
sol=find_root(F,-10,10)
print "Numerical solution:",sol

# Choose upper and lower bound and
# hope that the exact solution lies in between
xi_1=sol-0.0000001
xi_2=xi_1+0.0000002

#define a real value xi0 between xi_1 and xi_2
# representing the exact solution
xi0=RIF(xi_1,xi_2)

# Check whether Intermediate value theorem guarantees a zero between
# xi_1 and xi_2, i.e evaluate F at xi_1 and xi_2 using interval \
  arithmetic
if RIF(F(xi_1)) < 0 and RIF(F(xi_2)) > 0:
    print "Interval containing solution:", xi0.str(style='\
brackets')
```

Numerical solution: -1.9402428939

Interval containing solution: [-1.94024301 .. -1.94024276]

Step (iii) & (iv) obtain closed forms for  $DF_\xi(X_{y,0,1})$  and plug in the estimate for  $\xi$

For every choice of  $y \in \mathbb{P}^1$  we have to symbolically solve the integrals  $\int_{\square} e^{u\xi} \cdot \left( (1 + \Phi_y(u))^2 - (1 + \sum_{z \neq y} \Phi_z(u)) \right)$ , which up to scaling with a positive constant coincide with  $DF_\xi(\mathcal{X}_{y,0,1})$ . Then we plug in the estimate for  $\xi$  into the resulting expression.

```
#check for positivity of the DF invariant for our vector field xi
print("Stability test for test configurations:")

#storage for DF values (as intervals)
IDF={}

DF1(xi)=integral(exp(xi*u)*((Phi1+1)(u)^2-(Phi3+Phi2+1)(u)^2)/2,u\
, -1,B[1])
IDF[1]=RIF(DF1(xi0)) # evaluate DF1 at xi0 using interval arithmetic
show(DF1(xi) >= IDF[1].lower())

DF2(xi)=integral(exp(xi*u)*((Phi2+1)(u)^2-(Phi1+Phi3+1)(u)^2)/2,u\
, -1,B[1])
IDF[2]=RIF(DF2(xi0))
```

---

```

show(DF2(xi) >= IDF[2].lower())

DF3(xi)=integral(exp(xi*u)*((Phi3+1)(u)^2-(Phi1+Phi2+1)(u)^2)/2,u\
, -1 ,B[1])
IDF[3]=RIF(DF3(xi0))
show(DF3(xi) >= IDF[3].lower())

DF4(xi)=integral(exp(xi*u)*((1)^2-(Phi3+Phi2+Phi1+1)(u)^2)/2,u, -1 ,B\
[1])
IDF[4]=RIF(DF4(xi0))
show(DF4(xi) >= IDF[4].lower())

if all([DF > 0 for DF in IDF.values()]):
    print("Surface is stable!")
else:
    if any([DF <= 0 for DF in IDF.values()]):
        print("Surface is not stable!")

    # print upper bound for destablising DF value
    if IDF[1] <= 0: show(DF1(xi) <= IDF[1].upper())
    if IDF[2] <= 0: show(DF2(xi) <= IDF[2].upper())
    if IDF[3] <= 0: show(DF3(xi) <= IDF[3].upper())
    if IDF[4] <= 0: show(DF4(xi) <= IDF[4].upper())
    else:
        print("Cannot determine stability")
        # Note, that "not a > 0" does not imply "a <= 0" for \
intervals

```

Stability test for test configurations:

$$\begin{aligned}
& \frac{(4\xi - 1)e^{(3\xi)}}{16\xi^3} - \frac{(16(3\xi - 1)e^{(3\xi)} + 7)e^{(-\xi)}}{144\xi^3} \geq 0.04440443 \\
& \frac{(4\xi - 3)e^{(3\xi)}}{16\xi^3} - \frac{(8(3\xi - 4)e^{(3\xi)} + 5)e^{(-\xi)}}{144\xi^3} \geq 0.03181965 \\
& -\frac{(4\xi - 3)e^{(3\xi)}}{16\xi^3} + \frac{(4(9\xi - 10)e^{(3\xi)} + 12\xi + 13)e^{(-\xi)}}{144\xi^3} \geq 0.06993168 \\
& \frac{(4\xi - 1)e^{(3\xi)}}{16\xi^3} - \frac{(4(9\xi - 2)e^{(3\xi)} - 12\xi - 1)e^{(-\xi)}}{144\xi^3} \geq 0.1461557
\end{aligned}$$

Surface is stable!

---

No. 4: Degree 2 / Singularity type  $E_6A_2$ .

The combinatorial data is given by  $\square = [-1, 2]$  and  $\Phi_0(u) = \min\{\frac{u-1}{2}, 0\}$ ,  $\Phi_\infty(u) = \frac{u-2}{3}$ ,  $\Phi_1(u) = \frac{-2u-2}{3}$

```

# We are working with interval arithmetic with precision of 26 bit
# this fixes the precision e.g. for evaluations of exponential \
functions

```

```

RIF=RealIntervalField(26)

```

---

```
# The base polytope/interval
B=[-1,2]

# 3 PL functions on the interval
Phi1(u)=min_symbolic((u-1)/2,0)
Phi2(u)=1/3*u-2/3
Phi3(u)=-2/3*u-2/3
```

```
# the degree of \bar Phi
degPhi=Phi1+Phi2+Phi3+2
```

```
print "The combinatorial data"
show(B)
show(Phi1)
show(Phi2)
show(Phi3)
```

The combinatorial data

$$[-1, 2]$$

$$u \mapsto \min\left(\frac{1}{2}u - \frac{1}{2}, 0\right)$$

$$u \mapsto \frac{1}{3}u - \frac{2}{3}$$

$$u \mapsto -\frac{2}{3}u - \frac{2}{3}$$

Step (i) obtain a closed form for  $F_{X,\xi}(1)$

For this we have to analytically solve the integral  $\int_{\square} u \deg \bar{\Phi}(u) e^{\xi u} du$ .

```
# The integral can be solved symbolically:
F(xi)=integral(degPhi(u)*u*exp(xi*u),u,-1,B[1])
show(F(xi))
```

$$\frac{2(\xi-1)e^{(2\xi)}}{3\xi^3} - \frac{(3(\xi-2)e^{(2\xi)} + \xi + 2)e^{(-\xi)}}{6\xi^3}$$

Step (ii) find an estimate for the soliton candidate vector field  $\xi$

```
# Solve numerically
sol=find_root(F,-10,10)
print "Numerical solution:",sol

# Choose upper and lower bound and
# hope that the exact solution lies in between
xi_1=sol-0.0000001
xi_2=xi_1+0.0000002

#define a real value xi0 between xi_1 and xi_2
# representing the exact solution
```



---

```
xi0=RIF(xi_1,xi_2)
```

```
# Check whether Intermediate value theorem guarantees a zero between
# xi_1 and xi_2, i.e evaluate F at xi_1 and xi_2 using interval \
    arithmetic
if RIF(F(xi_1)) < 0 and RIF(F(xi_2)) > 0:
    print "Interval containing solution:", xi0.str(style='\
brackets')
```

Numerical solution: -1.69131741884

Interval containing solution: [-1.69131753 .. -1.69131729]

Step (iii) & (iv) obtain closed forms for  $DF_\xi(X_{y,0,1})$  and plug in the estimate for  $\xi$

For every choice of  $y \in \mathbb{P}^1$  we have to symbolically solve the integrals  $\int_{\square} e^{u\xi} \cdot ((1 + \Phi_y(u))^2 - (1 + \sum_{z \neq y} \Phi_z(u)))$  which up to scaling with a positive constant coincide with  $DF_\xi(\mathcal{X}_{y,0,1})$ . Then we plug in the estimate for  $\xi$  into the resulting expression.

```
#check for positivity of the DF invariant for our vector field xi
print("Stability test for test configurations:")

#storage for DF values (as intervals)
IDF={}

DF1(xi)=integral(exp(xi*u)*((Phi1+1)(u)^2-(Phi3+Phi2+1)(u)^2)/2,u\
    ,-1,B[1])
IDF[1]=RIF(DF1(xi0)) # evaluate DF1 at xi0 using interval arithmetic
show(DF1(xi) >= IDF[1].lower())

DF2(xi)=integral(exp(xi*u)*((Phi2+1)(u)^2-(Phi1+Phi3+1)(u)^2)/2,u\
    ,-1,B[1])
IDF[2]=RIF(DF2(xi0))
show(DF2(xi) >= IDF[2].lower())

DF3(xi)=integral(exp(xi*u)*((Phi3+1)(u)^2-(Phi1+Phi2+1)(u)^2)/2,u\
    ,-1,B[1])
IDF[3]=RIF(DF3(xi0))
show(DF3(xi) >= IDF[3].lower())

DF4(xi)=integral(exp(xi*u)*((1)^2-(Phi3+Phi2+Phi1+1)(u)^2)/2,u,-1,B\
    [1])
IDF[4]=RIF(DF4(xi0))
show(DF4(xi) >= IDF[4].lower())

if all([DF > 0 for DF in IDF.values()]):
    print("Surface is stable!")
else:
    if any([DF <= 0 for DF in IDF.values()]):
        print("Surface is not stable!")
```

---

```

# print upper bound for destablising DF value
if IDF[1] <= 0: show(DF1(xi) <= IDF[1].upper())
if IDF[2] <= 0: show(DF2(xi) <= IDF[2].upper())
if IDF[3] <= 0: show(DF3(xi) <= IDF[3].upper())
if IDF[4] <= 0: show(DF4(xi) <= IDF[4].upper())
else:
    print("Cannot determine stability")
    # Note, that "not a > 0" does not imply "a <= 0" for \
intervals

```

Stability test for test configurations:

$$\begin{aligned}
& \frac{(3\xi - 1)e^{(2\xi)}}{9\xi^3} - \frac{(9(2\xi - 1)e^{(2\xi)} + 5)e^{(-\xi)}}{36\xi^3} \geq 0.1187884 \\
& \frac{(\xi - 1)e^{(2\xi)}}{3\xi^3} - \frac{((2\xi - 5)e^{(2\xi)} + 1)e^{(-\xi)}}{12\xi^3} \geq 0.07315991 \\
& -\frac{(\xi - 1)e^{(2\xi)}}{3\xi^3} + \frac{((4\xi - 7)e^{(2\xi)} + 2\xi + 3)e^{(-\xi)}}{12\xi^3} \geq 0.07315988 \\
& \frac{(3\xi - 1)e^{(2\xi)}}{9\xi^3} - \frac{(3(4\xi - 1)e^{(2\xi)} - 6\xi - 1)e^{(-\xi)}}{36\xi^3} \geq 0.2651082
\end{aligned}$$

Surface is stable!

---

No. 6: Degree 2 / Singularity type  $A_5A_2$ .

The combinatorial data is given by  $\square = [-1, 2]$  and  $\Phi_0(u) = \min\{-u, 0\}$ ,  $\Phi_\infty(u) = \frac{u-2}{3}$ ,  $\Phi_1(u) = \frac{u-2}{3}$

```

# We are working with interval arithmetic with precision of 26 bit
# this fixes the precision e.g. for evaluations of exponential \
functions

```

```
RIF=RealIntervalField(26)
```

```

# The base polytope/interval
B=[-1,2]

```

```
# 3 PL functions on the interval
```

```
Phi1(u)=min_symbolic(-u,0)
```

```
Phi2(u)=1/3*u-2/3
```

```
Phi3(u)=1/3*u-2/3
```

```
# the degree of \bar Phi
```

```
degPhi=Phi1+Phi2+Phi3+2
```

```
print "The combinatorial data"
```

```
show(B)
```

```
show(Phi1)
```

```
show(Phi2)
```

```
show(Phi3)
```

---

The combinatorial data

$$\begin{aligned} &[-1, 2] \\ &u \mapsto \min(-u, 0) \\ &u \mapsto \frac{1}{3}u - \frac{2}{3} \\ &u \mapsto \frac{1}{3}u - \frac{2}{3} \end{aligned}$$

Step (i) obtain a closed form for  $F_{X,\xi}(1)$

For this we have to analytically solve the integral  $\int_{\square} u \deg \bar{\Phi}(u) e^{\xi u} du$ .

# The integral can be solved symbolically:

```
F(xi)=integral(degPhi(u)*u*exp(xi*u),u,-1,B[1])
show(F(xi))
```

$$-\frac{2(\xi+2)e^{(-\xi)}}{3\xi^3} + \frac{2((\xi-1)e^{(2\xi)}+3)}{3\xi^3}$$

Step (ii) find an estimate for the soliton candidate vector field  $\xi$

# Solve numerically

```
sol=find_root(F,-10,10)
print "Numerical solution:",sol
```

# Choose upper and lower bound and

# hope that the exact solution lies in between

```
xi_1=sol-0.0000001
xi_2=xi_1+0.0000002
```

#define a real value xi0 between xi\_1 and xi\_2

# representing the exact solution

```
xi0=RIF(xi_1,xi_2)
```

# Check whether Intermediate value theorem guarantees a zero between  
# xi\_1 and xi\_2, i.e evaluate F at xi\_1 and xi\_2 using interval \

```
arithmetic
if RIF(F(xi_1)) < 0 and RIF(F(xi_2)) > 0:
```

```
    print "Interval containing solution:", xi0.str(style='\
brackets')
```

Numerical solution: -0.97052220918

Interval containing solution: [-0.970522315 .. -0.970522105]

Step (iii) & (iv) obtain closed forms for  $DF_{\xi}(X_{y,0,1})$  and plug in the estimate for  $\xi$

For every choice of  $y \in \mathbb{P}^1$  we have to symbolically solve the integrals  $\int_{\square} e^{u\xi} \cdot ((1 + \Phi_y(u))^2 - (1 + \sum_{z \neq y} \Phi_z(u)))$  which up to scaling with a positive constant coincide with  $DF_{\xi}(\mathcal{X}_{y,0,1})$ . Then we plug in the estimate for  $\xi$  into the resulting expression.

#check for positivity of the DF invariant for our vector field xi

```
print("Stability test for test configurations:")
```

---

```

#storage for DF values (as intervals)
IDF={}

DF1(xi)=integral(exp(xi*u)*((Phi1+1)(u)^2-(Phi3+Phi2+1)(u)^2)/2,u\
, -1,B[1])
IDF[1]=RIF(DF1(xi0)) # evaluate DF1 at xi0 using interval arithmetic
show(DF1(xi) >= IDF[1].lower())

DF2(xi)=integral(exp(xi*u)*((Phi2+1)(u)^2-(Phi1+Phi3+1)(u)^2)/2,u\
, -1,B[1])
IDF[2]=RIF(DF2(xi0))
show(DF2(xi) >= IDF[2].lower())

DF3(xi)=integral(exp(xi*u)*((Phi3+1)(u)^2-(Phi1+Phi2+1)(u)^2)/2,u\
, -1,B[1])
IDF[3]=RIF(DF3(xi0))
show(DF3(xi) >= IDF[3].lower())

DF4(xi)=integral(exp(xi*u)*((1)^2-(Phi3+Phi2+Phi1+1)(u)^2)/2,u, -1,B\
[1])
IDF[4]=RIF(DF4(xi0))
show(DF4(xi) >= IDF[4].lower())

if all([DF > 0 for DF in IDF.values()]):
    print("Surface is stable!")
else:
    if any([DF <= 0 for DF in IDF.values()]):
        print("Surface is not stable!")

    # print upper bound for destabilising DF value
    if IDF[1] <= 0: show(DF1(xi) <= IDF[1].upper())
    if IDF[2] <= 0: show(DF2(xi) <= IDF[2].upper())
    if IDF[3] <= 0: show(DF3(xi) <= IDF[3].upper())
    if IDF[4] <= 0: show(DF4(xi) <= IDF[4].upper())
    else:
        print("Cannot determine stability")
        # Note, that "not a > 0" does not imply "a <= 0" for \
intervals

```

Stability test for test configurations:

$$\frac{2(3\xi+2)e^{(-\xi)}}{9\xi^3} - \frac{(3\xi-5)e^{(2\xi)}+9\xi+9}{9\xi^3} \geq 0.4790611$$

$$\frac{(\xi-1)e^{(2\xi)}+\xi+1}{3\xi^3} \geq 0.09239867$$

$$\frac{(\xi-1)e^{(2\xi)}+\xi+1}{3\xi^3} \geq 0.09239867$$

---


$$\frac{2(3\xi+2)e^{(-\xi)}}{9\xi^3} + \frac{(3\xi-1)e^{(2\xi)} - 3\xi - 3}{9\xi^3} \geq 0.6638587$$

Surface is stable!

---

No. 7: Degree 2 / Singularity type  $D_6A_1$ .

The combinatorial data is given by  $\square = [-1, 3]$  and  $\Phi_0(u) = \min\{\frac{u-1}{2}, 0\}$ ,  $\Phi_\infty(u) = \frac{u-3}{4}$ ,  $\Phi_1(u) = \frac{-u-1}{2}$

```
# We are working with interval arithmetic with precision of 26 bit
# this fixes the precision e.g. for evaluations of exponential \
  functions
```

```
RIF=RealIntervalField(26)
```

```
# The base polytope/interval
B=[-1,3]
```

```
# 3 PL functions on the interval
```

```
Phi1(u)=min_symbolic((u-1)/2,0)
```

```
Phi2(u)=1/4*u-3/4
```

```
Phi3(u)=-1/2*u-1/2
```

```
# the degree of \bar Phi
```

```
degPhi=Phi1+Phi2+Phi3+2
```

```
print "The combinatorial data"
```

```
show(B)
```

```
show(Phi1)
```

```
show(Phi2)
```

```
show(Phi3)
```

The combinatorial data

$[-1, 3]$

$u \mapsto \min\left(\frac{1}{2}u - \frac{1}{2}, 0\right)$

$u \mapsto \frac{1}{4}u - \frac{3}{4}$

$u \mapsto -\frac{1}{2}u - \frac{1}{2}$

Step (i) obtain a closed form for  $F_{X,\xi}(1)$

For this we have to analytically solve the integral  $\int_{\square} u \deg \bar{\Phi}(u) e^{\xi u} du$ .

```
# The integral can be solved symbolically:
```

```
F(xi)=integral(degPhi(u)*u*exp(xi*u),u,-1,B[1])
```

```
show(F(xi))
```

$$\frac{(3\xi-2)e^{(3\xi)}}{4\xi^3} - \frac{(2(\xi-2)e^{(2\xi)} + \xi + 2)e^{(-\xi)}}{4\xi^3}$$

Step (ii) find an estimate for the soliton candidate vector field  $\xi$

---

```

# Solve numerically
sol=find_root(F,-10,10)
print "Numerical solution:",sol

# Choose upper and lower bound and
# hope that the exact solution lies in between
xi_1=sol-0.0000001
xi_2=xi_1+0.0000002

#define a real value xi0 between xi_1 and xi_2
# representing the exact solution
xi0=RIF(xi_1,xi_2)

# Check whether Intermediate value theorem guarantees a zero between
# xi_1 and xi_2, i.e evaluate F at xi_1 and xi_2 using interval \
  arithmetic
if RIF(F(xi_1)) < 0 and RIF(F(xi_2)) > 0:
    print "Interval containing solution:", xi0.str(style='\
brackets')

Numerical solution: -1.79675598472
Interval containing solution: [-1.79675609 .. -1.79675588]

```

Step (iii) & (iv) obtain closed forms for  $DF_\xi(X_{y,0,1})$  and plug in the estimate for  $\xi$

For every choice of  $y \in \mathbb{P}^1$  we have to symbolically solve the integrals  $\int_{\square} e^{u\xi} \cdot \left( (1 + \Phi_y(u))^2 - (1 + \sum_{z \neq y} \Phi_z(u)) \right)$  which up to scaling with a positive constant coincide with  $DF_\xi(\mathcal{X}_{y,0,1})$ . Then we plug in the estimate for  $\xi$  into the resulting expression.

```

#check for positivity of the DF invariant for our vector field xi
print("Stability test for test configurations:")

#storage for DF values (as intervals)
IDF={}

DF1(xi)=integral(exp(xi*u)*((Phi1+1)(u)^2-(Phi3+Phi2+1)(u)^2)/2,u\
, -1,B[1])
IDF[1]=RIF(DF1(xi0)) # evaluate DF1 at xi0 using interval arithmetic
show(DF1(xi) >= IDF[1].lower())

DF2(xi)=integral(exp(xi*u)*((Phi2+1)(u)^2-(Phi1+Phi3+1)(u)^2)/2,u\
, -1,B[1])
IDF[2]=RIF(DF2(xi0))
show(DF2(xi) >= IDF[2].lower())

DF3(xi)=integral(exp(xi*u)*((Phi3+1)(u)^2-(Phi1+Phi2+1)(u)^2)/2,u\
, -1,B[1])
IDF[3]=RIF(DF3(xi0))
show(DF3(xi) >= IDF[3].lower())

```

---

```

DF4(xi)=integral(exp(xi*u)*((1)^2-(Phi3+Phi2+Phi1+1)(u)^2)/2,u,-1,B\
[1])
IDF[4]=RIF(DF4(xi0))
show(DF4(xi) >= IDF[4].lower())

if all([DF > 0 for DF in IDF.values()]):
    print("Surface is stable!")
else:
    if any([DF <= 0 for DF in IDF.values()]):
        print("Surface is not stable!")

    # print upper bound for destabilising DF value
    if IDF[1] <= 0: show(DF1(xi) <= IDF[1].upper())
    if IDF[2] <= 0: show(DF2(xi) <= IDF[2].upper())
    if IDF[3] <= 0: show(DF3(xi) <= IDF[3].upper())
    if IDF[4] <= 0: show(DF4(xi) <= IDF[4].upper())
    else:
        print("Cannot determine stability")
        # Note, that "not a > 0" does not imply "a <= 0" for \
intervals

```

Stability test for test configurations:

$$\begin{aligned}
& \frac{(4\xi-1)e^{(3\xi)}}{16\xi^3} - \frac{(4(2\xi-1)e^{(2\xi)}+3)e^{(-\xi)}}{16\xi^3} \geq 0.1624897 \\
& \frac{(4\xi-3)e^{(3\xi)}}{16\xi^3} + \frac{(4e^{(2\xi)}-1)e^{(-\xi)}}{16\xi^3} \geq 0.05832627 \\
& -\frac{(4\xi-3)e^{(3\xi)}}{16\xi^3} + \frac{(4(\xi-2)e^{(2\xi)}+4\xi+5)e^{(-\xi)}}{16\xi^3} \geq 0.1687342 \\
& \frac{(4\xi-1)e^{(3\xi)}}{16\xi^3} - \frac{(4\xi e^{(2\xi)}-4\xi-1)e^{(-\xi)}}{16\xi^3} \geq 0.3895503
\end{aligned}$$

Surface is stable!

---

No. 8: Degree 2 / Singularity type  $E_7$ .

The combinatorial data is given by  $\square = [-1, 5]$  and  $\Phi_0(u) = \min\{\frac{u-3}{4}, 0\}$ ,  $\Phi_\infty(u) = \frac{u-2}{3}$ ,  $\Phi_1(u) = \frac{-u-1}{2}$

```

# We are working with interval arithmetic with precision of 26 bit
# this fixes the precision e.g. for evaluations of exponential \
functions
RIF=RealIntervalField(26)

# The base polytope/interval
B=[-1,5]

# 3 PL functions on the interval
Phi1(u)=min_symbolic((u-3)/4,0)

```

---

```

Phi2(u)=1/3*(u-2)
Phi3(u)=1/2*(-u-1)

# the degree of \bar Phi
degPhi=Phi1+Phi2+Phi3+2

print "The combinatorial data"
show(B)
show(Phi1)
show(Phi2)
show(Phi3)

```

The combinatorial data

$$\begin{aligned}
 &[-1, 5] \\
 &u \mapsto \min\left(\frac{1}{4}u - \frac{3}{4}, 0\right) \\
 &u \mapsto \frac{1}{3}u - \frac{2}{3} \\
 &u \mapsto -\frac{1}{2}u - \frac{1}{2}
 \end{aligned}$$

Step (i) obtain a closed form for  $F_{X,\xi}(1)$

For this we have to analytically solve the integral  $\int_{\square} u \deg \bar{\Phi}(u) e^{\xi u} du$ .

```

# The integral can be solved symbolically:
F(xi)=integral(degPhi(u)*u*exp(xi*u),u,-1,B[1])
show(F(xi))

```

$$\frac{(5\xi - 2)e^{5\xi}}{6\xi^3} - \frac{(3(3\xi - 2)e^{4\xi} + \xi + 2)e^{-\xi}}{12\xi^3}$$

Step (ii) find an estimate for the soliton candidate vector field  $\xi$

```

# Solve numerically
sol=find_root(F,-10,10)
print "Numerical solution:",sol

# Choose upper and lower bound and
# hope that the exact solution lies in between
xi_1=sol-0.0000001
xi_2=xi_1+0.0000002

#define a real value xi0 between xi_1 and xi_2
# representing the exact solution
xi0=RIF(xi_1,xi_2)

# Check whether Intermediate value theorem guarantees a zero between
# xi_1 and xi_2, i.e evaluate F at xi_1 and xi_2 using interval \
arithmetic
if RIF(F(xi_1)) < 0 and RIF(F(xi_2)) > 0:

```



---

```

    print "Interval containing solution:", xi0.str(style='\
brackets')

```

Numerical solution: -1.99186220915

Interval containing solution: [-1.99186233 .. -1.99186208]

Step (iii) & (iv) obtain closed forms for  $DF_\xi(X_{y,0,1})$  and plug in the estimate for  $\xi$

For every choice of  $y \in \mathbb{P}^1$  we have to symbolically solve the integrals  $\int_{\square} e^{u\xi} \cdot ((1 + \Phi_y(u))^2 - (1 + \sum_{z \neq y} \Phi_z(u)))$  which up to scaling with a positive constant coincide with  $DF_\xi(\mathcal{X}_{y,0,1})$ . Then we plug in the estimate for  $\xi$  into the resulting expression.

```

#check for positivity of the DF invariant for our vector field xi
print("Stability test for test configurations:")

#storage for DF values (as intervals)
IDF={}

DF1(xi)=integral(exp(xi*u)*((Phi1+1)(u)^2-(Phi3+Phi2+1)(u)^2)/2,u\
, -1 ,B[1])
IDF[1]=RIF(DF1(xi0)) # evaluate DF1 at xi0 using interval arithmetic
show(DF1(xi) >= IDF[1].lower())

DF2(xi)=integral(exp(xi*u)*((Phi2+1)(u)^2-(Phi1+Phi3+1)(u)^2)/2,u\
, -1 ,B[1])
IDF[2]=RIF(DF2(xi0))
show(DF2(xi) >= IDF[2].lower())

DF3(xi)=integral(exp(xi*u)*((Phi3+1)(u)^2-(Phi1+Phi2+1)(u)^2)/2,u\
, -1 ,B[1])
IDF[3]=RIF(DF3(xi0))
show(DF3(xi) >= IDF[3].lower())

DF4(xi)=integral(exp(xi*u)*((1)^2-(Phi3+Phi2+Phi1+1)(u)^2)/2,u, -1 ,B\
[1])
IDF[4]=RIF(DF4(xi0))
show(DF4(xi) >= IDF[4].lower())

if all([DF > 0 for DF in IDF.values()]):
    print("Surface is stable!")
else:
    if any([DF <= 0 for DF in IDF.values()]):
        print("Surface is not stable!")

# print upper bound for destabilising DF value
if IDF[1] <= 0: show(DF1(xi) <= IDF[1].upper())
if IDF[2] <= 0: show(DF2(xi) <= IDF[2].upper())
if IDF[3] <= 0: show(DF3(xi) <= IDF[3].upper())
if IDF[4] <= 0: show(DF4(xi) <= IDF[4].upper())

```

---

```

else :
    print("Cannot determine stability")
    # Note, that "not a > 0" does not imply "a <= 0" for \
    intervals

```

Stability test for test configurations:

$$\begin{aligned}
& \frac{(6\xi - 1)e^{(5\xi)}}{36\xi^3} - \frac{(9(4\xi - 1)e^{(4\xi)} + 5)e^{(-\xi)}}{144\xi^3} \geq 0.03202411 \\
& \frac{(12\xi - 5)e^{(5\xi)}}{36\xi^3} - \frac{(9(4\xi - 3)e^{(4\xi)} + 7)e^{(-\xi)}}{144\xi^3} \geq 0.04486743 \\
& -\frac{(12\xi - 5)e^{(5\xi)}}{36\xi^3} + \frac{(3(16\xi - 11)e^{(4\xi)} + 12\xi + 13)e^{(-\xi)}}{144\xi^3} \geq 0.07049793 \\
& \frac{(6\xi - 1)e^{(5\xi)}}{36\xi^3} - \frac{(3(8\xi - 1)e^{(4\xi)} - 12\xi - 1)e^{(-\xi)}}{144\xi^3} \geq 0.1473894
\end{aligned}$$

Surface is stable!

---

No. 9: Degree 2 / Singularity type  $E_6$ .

The combinatorial data is given by  $\square = [-1, 3]$  and  $\Phi_0(u) = \min\{\frac{u-2}{3}, 0\}$ ,  $\Phi_\infty(u) = \min\{\frac{u-2}{3}, 0\}$ ,  $\Phi_1(u) = \frac{-u-1}{2}$

```

# We are working with interval arithmetic with precision of 26 bit
# this fixes the precision e.g. for evaluations of exponential \
  functions

```

```

RIF=RealIntervalField(26)

```

```

# The base polytope/interval
B=[-1,3]

```

```

# 3 PL functions on the interval

```

```

Phi1(u)=min_symbolic((u-2)/3,0)
Phi2(u)=min_symbolic((u-2)/3,0)
Phi3(u)=1/2*(-u-1)

```

```

# the degree of \bar Phi
degPhi=Phi1+Phi2+Phi3+2

```

```

print "The combinatorial data"
show(B)
show(Phi1)
show(Phi2)
show(Phi3)

```

The combinatorial data

$$\begin{aligned}
& [-1, 3] \\
& u \mapsto \min\left(\frac{1}{3}u - \frac{2}{3}, 0\right) \\
& u \mapsto \min\left(\frac{1}{3}u - \frac{2}{3}, 0\right)
\end{aligned}$$

$$u \mapsto -\frac{1}{2}u - \frac{1}{2}$$

Step (i) obtain a closed form for  $F_{X,\xi}(1)$

For this we have to analytically solve the integral  $\int_{\square} u \deg \bar{\Phi}(u) e^{\xi u} du$ .

# The integral can be solved symbolically:

```
F(xi)=integral(degPhi(u)*u*exp(xi*u),u,-1,B[1])
show(F(xi))
```

$$\frac{(3\xi - 2)e^{(3\xi)}}{2\xi^3} - \frac{(8(\xi - 1)e^{(3\xi)} + \xi + 2)e^{(-\xi)}}{6\xi^3}$$

Step (ii) find an estimate for the soliton candidate vector field  $\xi$

# Solve numerically

```
sol=find_root(F,-10,10)
print "Numerical solution:",sol
```

# Choose upper and lower bound and

# hope that the exact solution lies in between

```
xi_1=sol-0.0000001
xi_2=xi_1+0.0000002
```

#define a real value xi0 between xi\_1 and xi\_2

# representing the exact solution

```
xi0=RIF(xi_1,xi_2)
```

# Check whether Intermediate value theorem guarantees a zero between  
# xi\_1 and xi\_2, i.e evaluate F at xi\_1 and xi\_2 using interval \

```
arithmetic
if RIF(F(xi_1)) < 0 and RIF(F(xi_2)) > 0:
    print "Interval containing solution:", xi0.str(style='\
brackets')
```

Numerical solution: -1.9402428939

Interval containing solution: [-1.94024301 .. -1.94024276]

Step (iii) & (iv) obtain closed forms for  $DF_{\xi}(X_{y,0,1})$  and plug in the estimate for  $\xi$

For every choice of  $y \in \mathbb{P}^1$  we have to symbolically solve the integrals  $\int_{\square} e^{u\xi} \cdot ((1 + \Phi_y(u))^2 - (1 + \sum_{z \neq y} \Phi_z(u)))$  which up to scaling with a positive constant coincide with  $DF_{\xi}(\mathcal{X}_{y,0,1})$ . Then we plug in the estimate for  $\xi$  into the resulting expression.

```
#check for positivity of the DF invariant for our vector field xi
print("Stability test for test configurations:")
```

#storage for DF values (as intervals)

```
IDF={}
```

```
DF1(xi)=integral(exp(xi*u)*((Phi1+1)(u)^2-(Phi3+Phi2+1)(u)^2)/2,u\
```

---

```

    , -1, B[1])
IDF[1]=RIF(DF1(xi0)) # evaluate DF1 at xi0 using interval arithmetic
show(DF1(xi) >= IDF[1].lower())

DF2(xi)=integral(exp(xi*u)*((Phi2+1)(u)^2-(Phi1+Phi3+1)(u)^2)/2,u\
    , -1, B[1])
IDF[2]=RIF(DF2(xi0))
show(DF2(xi) >= IDF[2].lower())

DF3(xi)=integral(exp(xi*u)*((Phi3+1)(u)^2-(Phi1+Phi2+1)(u)^2)/2,u\
    , -1, B[1])
IDF[3]=RIF(DF3(xi0))
show(DF3(xi) >= IDF[3].lower())

DF4(xi)=integral(exp(xi*u)*((1)^2-(Phi3+Phi2+Phi1+1)(u)^2)/2,u, -1, B\
    [1])
IDF[4]=RIF(DF4(xi0))
show(DF4(xi) >= IDF[4].lower())

if all([DF > 0 for DF in IDF.values()]):
    print("Surface is stable!")
else:
    if any([DF <= 0 for DF in IDF.values()]):
        print("Surface is not stable!")

    # print upper bound for destabilising DF value
    if IDF[1] <= 0: show(DF1(xi) <= IDF[1].upper())
    if IDF[2] <= 0: show(DF2(xi) <= IDF[2].upper())
    if IDF[3] <= 0: show(DF3(xi) <= IDF[3].upper())
    if IDF[4] <= 0: show(DF4(xi) <= IDF[4].upper())
    else:
        print("Cannot determine stability")
        # Note, that "not a > 0" does not imply "a <= 0" for \
        intervals

```

Stability test for test configurations:

$$\begin{aligned}
& \frac{(2\xi - 1)e^{(3\xi)}}{4\xi^3} - \frac{(2(3\xi - 2)e^{(3\xi)} + 1)e^{(-\xi)}}{12\xi^3} \geq 0.07622408 \\
& \frac{(2\xi - 1)e^{(3\xi)}}{4\xi^3} - \frac{(2(3\xi - 2)e^{(3\xi)} + 1)e^{(-\xi)}}{12\xi^3} \geq 0.07622408 \\
& -\frac{(2\xi - 1)e^{(3\xi)}}{4\xi^3} + \frac{(8(3\xi - 2)e^{(3\xi)} + 6\xi + 7)e^{(-\xi)}}{36\xi^3} \geq 0.1272785 \\
& \frac{(2\xi - 1)e^{(3\xi)}}{4\xi^3} - \frac{(4(3\xi - 2)e^{(3\xi)} - 6\xi - 1)e^{(-\xi)}}{36\xi^3} \geq 0.2797267
\end{aligned}$$

Surface is stable!

---

No. 11: Degree 2 / Singularity type  $D_5A_1$ .

The combinatorial data is given by  $\square = [-1, 2]$  and  $\Phi_0(u) = \min\{\frac{u-1}{2}, 0\}$ ,  $\Phi_\infty(u) = \min\{\frac{u-1}{2}, 0\}$ ,  $\Phi_1(u) = \frac{-2u-2}{3}$

```
# We are working with interval arithmetic with precision of 26 bit
# this fixes the precision e.g. for evaluations of exponential \
  functions
```

```
RIF=RealIntervalField(26)
```

```
# The base polytope/interval
B=[-1,2]
```

```
# 3 PL functions on the interval
```

```
Phi1(u)=min_symbolic((u-1)/2,0)
```

```
Phi2(u)=min_symbolic((u-1)/2,0)
```

```
Phi3(u)=1/3*(-2*u-2)
```

```
# the degree of \bar Phi
```

```
degPhi=Phi1+Phi2+Phi3+2
```

```
print "The combinatorial data"
```

```
show(B)
```

```
show(Phi1)
```

```
show(Phi2)
```

```
show(Phi3)
```

The combinatorial data

$[-1, 2]$

$u \mapsto \min\left(\frac{1}{2}u - \frac{1}{2}, 0\right)$

$u \mapsto \min\left(\frac{1}{2}u - \frac{1}{2}, 0\right)$

$u \mapsto -\frac{2}{3}u - \frac{2}{3}$

Step (i) obtain a closed form for  $F_{X,\xi}(1)$

For this we have to analytically solve the integral  $\int_{\square} u \deg \bar{\Phi}(u) e^{\xi u} du$ .

```
# The integral can be solved symbolically:
```

```
F(xi)=integral(degPhi(u)*u*exp(xi*u),u,-1,B[1])
```

```
show(F(xi))
```

$$\frac{4(\xi - 1)e^{(2\xi)}}{3\xi^3} - \frac{(3(\xi - 2)e^{(2\xi)} + \xi + 2)e^{(-\xi)}}{3\xi^3}$$

Step (ii) find an estimate for the soliton candidate vector field  $\xi$

```
# Solve numerically
```

```
sol=find_root(F,-10,10)
```

```
print "Numerical solution:",sol
```

---

```

# Choose upper and lower bound and
# hope that the exact solution lies in between
xi_1=sol-0.00001
xi_2=xi_1+0.00002

#define a real value xi0 between xi_1 and xi_2
# representing the exact solution
xi0=RIF(xi_1,xi_2)

# Check whether Intermediate value theorem guarantees a zero between
# xi_1 and xi_2, i.e evaluate F at xi_1 and xi_2 using interval \
  arithmetic
if RIF(F(xi_1)) < 0 and RIF(F(xi_2)) > 0:
    print "Interval containing solution:", xi0.str(style='\
brackets')

```

Numerical solution: -1.69131741884

Interval containing solution: [-1.69132743 .. -1.69130739]

Step (iii) & (iv) obtain closed forms for  $DF_\xi(X_{y,0,1})$  and plug in the estimate for  $\xi$

For every choice of  $y \in \mathbb{P}^1$  we have to symbolically solve the integrals  $\int_{\square} e^{u\xi} \cdot \left( (1 + \Phi_y(u))^2 - (1 + \sum_{z \neq y} \Phi_z(u)) \right)$  which up to scaling with a positive constant coincide with  $DF_\xi(\mathcal{X}_{y,0,1})$ . Then we plug in the estimate for  $\xi$  into the resulting expression.

```

#check for positivity of the DF invariant for our vector field xi
print("Stability test for test configurations:")

#storage for DF values (as intervals)
IDF={}

DF1(xi)=integral(exp(xi*u)*((Phi1+1)(u)^2-(Phi3+Phi2+1)(u)^2)/2,u\
, -1,B[1])
IDF[1]=RIF(DF1(xi0)) # evaluate DF1 at xi0 using interval arithmetic
show(DF1(xi) >= IDF[1].lower())

DF2(xi)=integral(exp(xi*u)*((Phi2+1)(u)^2-(Phi1+Phi3+1)(u)^2)/2,u\
, -1,B[1])
IDF[2]=RIF(DF2(xi0))
show(DF2(xi) >= IDF[2].lower())

DF3(xi)=integral(exp(xi*u)*((Phi3+1)(u)^2-(Phi1+Phi2+1)(u)^2)/2,u\
, -1,B[1])
IDF[3]=RIF(DF3(xi0))
show(DF3(xi) >= IDF[3].lower())

DF4(xi)=integral(exp(xi*u)*((1)^2-(Phi3+Phi2+Phi1+1)(u)^2)/2,u, -1,B\
[1])
IDF[4]=RIF(DF4(xi0))

```

---

```

show(DF4(xi) >= IDF[4].lower())

if all([DF > 0 for DF in IDF.values()]):
    print("Surface is stable!")
else:
    if any([DF <= 0 for DF in IDF.values()]):
        print("Surface is not stable!")

        # print upper bound for destabilising DF value
        if IDF[1] <= 0: show(DF1(xi) <= IDF[1].upper())
        if IDF[2] <= 0: show(DF2(xi) <= IDF[2].upper())
        if IDF[3] <= 0: show(DF3(xi) <= IDF[3].upper())
        if IDF[4] <= 0: show(DF4(xi) <= IDF[4].upper())
    else:
        print("Cannot determine stability")
        # Note, that "not a > 0" does not imply "a <= 0" for \
intervals

```

Stability test for test configurations:

$$\begin{aligned}
& \frac{2(3\xi - 2)e^{(2\xi)}}{9\xi^3} - \frac{2(3(\xi - 1)e^{(2\xi)} + 1)e^{(-\xi)}}{9\xi^3} \geq 0.1919413 \\
& \frac{2(3\xi - 2)e^{(2\xi)}}{9\xi^3} - \frac{2(3(\xi - 1)e^{(2\xi)} + 1)e^{(-\xi)}}{9\xi^3} \geq 0.1919413 \\
& -\frac{2(3\xi - 2)e^{(2\xi)}}{9\xi^3} + \frac{(9(\xi - 1)e^{(2\xi)} + 3\xi + 5)e^{(-\xi)}}{9\xi^3} \geq 0.1006816 \\
& \frac{2(3\xi - 2)e^{(2\xi)}}{9\xi^3} - \frac{(3(\xi - 1)e^{(2\xi)} - 3\xi - 1)e^{(-\xi)}}{9\xi^3} \geq 0.4845700
\end{aligned}$$

Surface is stable!

---

No. 12: Degree 2 / Singularity type  $3A_1D_4$ .

The combinatorial data is given by  $\square = [-1, 1]$  and  $\Phi_0(u) = \frac{u-1}{2}$ ,  $\Phi_\infty(u) = \frac{u-1}{2}$ ,  $\Phi_1(u) = \frac{-u-1}{2}$

```

# We are working with interval arithmetic with precision of 26 bit
# this fixes the precision e.g. for evaluations of exponential \
functions

```

```

RIF=RealIntervalField(26)

```

```

# The base polytope/interval
B=[-1,3]

```

```

# 3 PL functions on the interval
Phi1(u)=1/2*(u-1)
Phi2(u)=1/2*(u-1)
Phi3(u)=1/2*(-u-1)

```

```

# the degree of \bar Phi

```

---

```
degPhi=Phi1+Phi2+Phi3+2

print "The combinatorial data"
show(B)
show(Phi1)
show(Phi2)
show(Phi3)
```

The combinatorial data

$$[-1, 3]$$

$$u \mapsto \frac{1}{2}u - \frac{1}{2}$$

$$u \mapsto \frac{1}{2}u - \frac{1}{2}$$

$$u \mapsto -\frac{1}{2}u - \frac{1}{2}$$

Step (i) obtain a closed form for  $F_{X,\xi}(1)$

For this we have to analytically solve the integral  $\int_{\square} u \deg \bar{\Phi}(u) e^{\xi u} du$ .

```
# The integral can be solved symbolically:
F(xi)=integral(degPhi(u)*u*exp(xi*u),u,-1,B[1])
show(F(xi))
```

$$\frac{(12\xi^2 - 7\xi + 2)e^{(3\xi)}}{2\xi^3} - \frac{(\xi + 2)e^{(-\xi)}}{2\xi^3}$$

Step (ii) find an estimate for the soliton candidate vector field  $\xi$

```
# Solve numerically
sol=find_root(F,-10,10)
print "Numerical solution:",sol

# Choose upper and lower bound and
# hope that the exact solution lies in between
xi_1=sol-0.0000001
xi_2=xi_1+0.0000002

#define a real value xi0 between xi_1 and xi_2
# representing the exact solution
xi0=RIF(xi_1,xi_2)

# Check whether Intermediate value theorem guarantees a zero between
# xi_1 and xi_2, i.e evaluate F at xi_1 and xi_2 using interval \
arithmetic
if RIF(F(xi_1)) < 0 and RIF(F(xi_2)) > 0:
    print "Interval containing solution:", xi0.str(style='\
brackets')
```

Numerical solution: -1.97691850478

Interval containing solution: [-1.97691861 .. -1.97691839]



Step (iii) & (iv) obtain closed forms for  $DF_\xi(X_{y,0,1})$  and plug in the estimate for  $\xi$

For every choice of  $y \in \mathbb{P}^1$  we have to symbolically solve the integrals  $\int_{\square} e^{u\xi} \cdot ((1 + \Phi_y(u))^2 - (1 + \sum_{z \neq y} \Phi_z(u)))$  which up to scaling with a positive constant coincide with  $DF_\xi(\mathcal{X}_{y,0,1})$ . Then we plug in the estimate for  $\xi$  into the resulting expression.

```
#check for positivity of the DF invariant for our vector field xi
print("Stability test for test configurations:")

#storage for DF values (as intervals)
IDF={}

DF1(xi)=integral(exp(xi*u)*((Phi1+1)(u)^2-(Phi3+Phi2+1)(u)^2)/2,u\
, -1,B[1])
IDF[1]=RIF(DF1(xi0)) # evaluate DF1 at xi0 using interval arithmetic
show(DF1(xi) >= IDF[1].lower())

DF2(xi)=integral(exp(xi*u)*((Phi2+1)(u)^2-(Phi1+Phi3+1)(u)^2)/2,u\
, -1,B[1])
IDF[2]=RIF(DF2(xi0))
show(DF2(xi) >= IDF[2].lower())

DF3(xi)=integral(exp(xi*u)*((Phi3+1)(u)^2-(Phi1+Phi2+1)(u)^2)/2,u\
, -1,B[1])
IDF[3]=RIF(DF3(xi0))
show(DF3(xi) >= IDF[3].lower())

DF4(xi)=integral(exp(xi*u)*((1)^2-(Phi3+Phi2+Phi1+1)(u)^2)/2,u,-1,B\
[1])
IDF[4]=RIF(DF4(xi0))
show(DF4(xi) >= IDF[4].lower())

if all([DF > 0 for DF in IDF.values()]):
    print("Surface is stable!")
else:
    if any([DF <= 0 for DF in IDF.values()]):
        print("Surface is not stable!")

        # print upper bound for destabilising DF value
        if IDF[1] <= 0: show(DF1(xi) <= IDF[1].upper())
        if IDF[2] <= 0: show(DF2(xi) <= IDF[2].upper())
        if IDF[3] <= 0: show(DF3(xi) <= IDF[3].upper())
        if IDF[4] <= 0: show(DF4(xi) <= IDF[4].upper())
    else:
        print("Cannot determine stability")
        # Note, that "not a > 0" does not imply "a <= 0" for \
intervals
```

Stability test for test configurations:

---


$$\frac{(8\xi^2 - 4\xi + 1)e^{(3\xi)}}{4\xi^3} - \frac{e^{(-\xi)}}{4\xi^3} \geq 0.2301820$$

$$\frac{(8\xi^2 - 4\xi + 1)e^{(3\xi)}}{4\xi^3} - \frac{e^{(-\xi)}}{4\xi^3} \geq 0.2301820$$

$$-\frac{(16\xi^2 - 10\xi + 3)e^{(3\xi)}}{4\xi^3} + \frac{(2\xi + 3)e^{(-\xi)}}{4\xi^3} \geq 0.2301820$$

$$\frac{(2\xi - 1)e^{(3\xi)}}{4\xi^3} + \frac{(2\xi + 1)e^{(-\xi)}}{4\xi^3} \geq 0.6905461$$

Surface is stable!

---

No. 13: Degree 3 / Singularity type  $A_5A_1$ .

The combinatorial data is given by  $\square = [-1, 3]$  and  $\Phi_0(u) = \min\{-u, 0\}$ ,  $\Phi_\infty(u) = \frac{u-3}{4}$ ,  $\Phi_1(u) = \frac{u-1}{2}$

```
# We are working with interval arithmetic with precision of 16 bit
# this fixes the precision e.g. for evaluations of exponential \
  functions
```

```
RIF=RealIntervalField(11)
```

```
# The base polytope/interval
B=[ -1 ,3]
```

```
# 3 PL functions on the interval
Phi1(u)=min_symbolic(-u,0)
Phi2(u)=1/4*u-3/4
Phi3(u)=1/2*u-1/2
```

```
# the degree of \bar Phi
degPhi=Phi1+Phi2+Phi3+2
```

```
print "The combinatorial data"
show(B)
show(Phi1)
show(Phi2)
show(Phi3)
```

The combinatorial data

```
[-1, 3]
u ↦ min(-u, 0)
u ↦ 1/4 u - 3/4
u ↦ 1/2 u - 1/2
```

Step (i) obtain a closed form for  $F_{X,\xi}(1)$

For this we have to analytically solve the integral  $\int_{\square} u \deg \bar{\Phi}(u) e^{\xi u} du$ .

```
# The integral can be solved symbolically:
```

---

```
F(xi)=integral(degPhi(u)*u*exp(xi*u),u,-1,B[1])
```

```
show(F(xi))
```

$$-\frac{3(\xi+2)e^{(-\xi)}}{4\xi^3} + \frac{(3\xi-2)e^{(3\xi)}+8}{4\xi^3}$$

Step (ii) find an estimate for the soliton candidate vector field  $\xi$

```
# Solve numerically
```

```
sol=find_root(F,-10,10)
```

```
print "Numerical solution:",sol
```

```
# Choose upper and lower bound and
```

```
# hope that the exact solution lies in between
```

```
xi_1=sol-0.001
```

```
xi_2=sol+0.001
```

```
xi_1=-1.247
```

```
xi_2=-1.246
```

```
#define a real value xi0 between xi_1 and xi_2
```

```
# representing the exact solution
```

```
xi0=RIF(xi_1,xi_2)
```

```
# Check whether Intermediate value theorem guarantees a zero between
# xi_1 and xi_2, i.e evaluate F at xi_1 and xi_2 using interval \
arithmetic
```

```
if RIF(F(xi_1)) < 0 and RIF(F(xi_2)) > 0:
```

```
    print "Interval containing solution:", xi0.str(style='brackets')
```

```
Numerical solution: -1.24607304295
```

```
Interval containing solution: [-1.2471 .. -1.2451]
```

Step (iii) & (iv) obtain closed forms for  $DF_\xi(X_{y,0,1})$  and plug in the estimate for  $\xi$

For every choice of  $y \in \mathbb{P}^1$  we have to symbolically solve the integrals  $\int_{\square} e^{u\xi} \cdot ((1 + \Phi_y(u))^2 - (1 + \sum_{z \neq y} \Phi_z(u)))$  which up to scaling with a positive constant coincide with  $DF_\xi(\mathcal{X}_{y,0,1})$ . Then we plug in the estimate for  $\xi$  into the resulting expression.

```
#check for positivity of the DF invariant for our vector field xi
```

```
print("Stability test for test configurations:")
```

```
#storage for DF values (as intervals)
```

```
IDF={}
```

```
DF1(xi)=integral(exp(xi*u)*((Phi1+1)(u)^2-(Phi3+Phi2+1)(u)^2)/2,u\
,-1,B[1])
```

```
IDF[1]=RIF(DF1(xi0)) # evaluate DF1 at xi0 using interval arithmetic
```

```
show(DF1(xi) >= IDF[1].lower())
```

---

```

DF2(xi)=integral(exp(xi*u)*((Phi2+1)(u)^2-(Phi1+Phi3+1)(u)^2)/2,u\
, -1,B[1])
IDF[2]=RIF(DF2(xi0))
show(DF2(xi) >= IDF[2].lower())

DF3(xi)=integral(exp(xi*u)*((Phi3+1)(u)^2-(Phi1+Phi2+1)(u)^2)/2,u\
, -1,B[1])
IDF[3]=RIF(DF3(xi0))
show(DF3(xi) >= IDF[3].lower())

DF4(xi)=integral(exp(xi*u)*((1)^2-(Phi3+Phi2+Phi1+1)(u)^2)/2,u, -1,B\
[1])
IDF[4]=RIF(DF4(xi0))
show(DF4(xi) >= IDF[4].lower())

if all([DF > 0 for DF in IDF.values()]):
    print("Surface is stable!")
else:
    if any([DF <= 0 for DF in IDF.values()]):
        print("Surface is not stable!")

    # print upper bound for destabilising DF value
    if IDF[1] <= 0: show(DF1(xi) <= IDF[1].upper())
    if IDF[2] <= 0: show(DF2(xi) <= IDF[2].upper())
    if IDF[3] <= 0: show(DF3(xi) <= IDF[3].upper())
    if IDF[4] <= 0: show(DF4(xi) <= IDF[4].upper())
    else:
        print("Cannot determine stability")
        # Note, that "not a > 0" does not imply "a <= 0" for \
intervals

```

Stability test for test configurations:

$$\frac{3(4\xi+3)e^{(-\xi)}}{16\xi^3} - \frac{(8\xi-7)e^{(3\xi)}+16\xi+16}{16\xi^3} \geq 0.521$$

$$\frac{(4\xi-3)e^{(3\xi)}+8\xi}{16\xi^3} + \frac{3e^{(-\xi)}}{16\xi^3} \geq (-0.0120)$$

$$\frac{(8\xi-5)e^{(3\xi)}+4\xi+8}{16\xi^3} - \frac{3e^{(-\xi)}}{16\xi^3} \geq 0.248$$

$$\frac{3(4\xi+3)e^{(-\xi)}}{16\xi^3} + \frac{(4\xi-1)e^{(3\xi)}-4\xi-8}{16\xi^3} \geq 0.764$$

Surface is not stable!

$$\frac{(4\xi-3)e^{(3\xi)}+8\xi}{16\xi^3} + \frac{3e^{(-\xi)}}{16\xi^3} \leq (-0.00537)$$

---

No. 14: Degree 3 / Singularity type  $E_6$ .

The combinatorial data is given by  $\square = [-1, 5]$  and  $\Phi_0(u) = \min\{\frac{u-1}{3}, 0\}$ ,  $\Phi_\infty(u) = \frac{u-2}{3}$ ,  $\Phi_1(u) = \frac{-u-1}{2}$

---

```
# We are working with interval arithmetic with precision of 26 bit
# this fixes the precision e.g. for evaluations of exponential \
    functions
```

```
RIF=RealIntervalField(26)
```

```
# The base polytope/interval
B=[-1,3]
```

```
# 3 PL functions on the interval
```

```
Phi1(u)=min_symbolic((u-2)/3,0)
```

```
Phi2(u)=(u-2)/3
```

```
Phi3(u)=(-u-1)/2
```

```
# the degree of \bar Phi
```

```
degPhi=Phi1+Phi2+Phi3+2
```

```
print "The combinatorial data"
```

```
show(B)
```

```
show(Phi1)
```

```
show(Phi2)
```

```
show(Phi3)
```

The combinatorial data

$[-1, 3]$

$u \mapsto \min\left(\frac{1}{3}u - \frac{2}{3}, 0\right)$

$u \mapsto \frac{1}{3}u - \frac{2}{3}$

$u \mapsto -\frac{1}{2}u - \frac{1}{2}$

Step (i) obtain a closed form for  $F_{X,\xi}(1)$

For this we have to analytically solve the integral  $\int_{\square} u \deg \bar{\Phi}(u) e^{\xi u} du$ .

```
# The integral can be solved symbolically:
```

```
F(xi)=integral(degPhi(u)*u*exp(xi*u),u,-1,B[1])
```

```
show(F(xi))
```

$$\frac{(6\xi^2 + \xi - 2)e^{(3\xi)}}{6\xi^3} - \frac{(4(\xi - 1)e^{(3\xi)} + \xi + 2)e^{(-\xi)}}{6\xi^3}$$

Step (ii) find an estimate for the soliton candidate vector field  $\xi$

```
# Solve numerically
```

```
sol=find_root(F,-10,10)
```

```
print "Numerical solution:",sol
```

```
# Choose upper and lower bound and
```

```
# hope that the exact solution lies in between
```

```
xi_1=sol-0.0000001
```

---

```
xi_2=xi_1+0.0000002
```

```
#define a real value xi0 between xi_1 and xi_2
```

```
# representing the exact solution
```

```
xi0=RIF(xi_1,xi_2)
```

```
# Check whether Intermediate value theorem guarantees a zero beween  
# xi_1 and xi_2, i.e evaluate F at xi_1 and xi_2 using interval \
```

```
arithmetic
```

```
if RIF(F(xi_1)) < 0 and RIF(F(xi_2)) > 0:
```

```
    print "Interval containing solution:", xi0.str(style='\
```

```
brackets')
```

```
Numerical solution: -1.95932042376
```

```
Interval containing solution: [-1.95932055 .. -1.95932030]
```

Step (iii) & (iv) obtain closed forms for  $DF_\xi(X_{y,0,1})$  and plug in the estimate for  $\xi$

For every choice of  $y \in \mathbb{P}^1$  we have to symbolically solve the integrals  $\int_{\square} e^{u\xi} \cdot ((1 + \Phi_y(u))^2 - (1 + \sum_{z \neq y} \Phi_z(u)))$  which up to scaling with a positive constant coincide with  $DF_\xi(\mathcal{X}_{y,0,1})$ . Then we plug in the estimate for  $\xi$  into the resulting expression.

```
#check for positivity of the DF invariant for our vector field xi
```

```
print("Stability test for test configurations:")
```

```
#storage for DF values (as intervals)
```

```
IDF={}
```

```
DF1(xi)=integral(exp(xi*u)*((Phi1+1)(u)^2-(Phi3+Phi2+1)(u)^2)/2,u\
```

```
, -1,B[1])
```

```
IDF[1]=RIF(DF1(xi0)) # evaluate DF1 at xi0 using interval arithmetic
```

```
show(DF1(xi) >= IDF[1].lower())
```

```
DF2(xi)=integral(exp(xi*u)*((Phi2+1)(u)^2-(Phi1+Phi3+1)(u)^2)/2,u\
```

```
, -1,B[1])
```

```
IDF[2]=RIF(DF2(xi0))
```

```
show(DF2(xi) >= IDF[2].lower())
```

```
DF3(xi)=integral(exp(xi*u)*((Phi3+1)(u)^2-(Phi1+Phi2+1)(u)^2)/2,u\
```

```
, -1,B[1])
```

```
IDF[3]=RIF(DF3(xi0))
```

```
show(DF3(xi) >= IDF[3].lower())
```

```
DF4(xi)=integral(exp(xi*u)*((1)^2-(Phi3+Phi2+Phi1+1)(u)^2)/2,u, -1,B\
```

```
[1])
```

```
IDF[4]=RIF(DF4(xi0))
```

```
show(DF4(xi) >= IDF[4].lower())
```

```
if all([DF > 0 for DF in IDF.values()]):
```

---

```

    print("Surface is stable!")
else:
    if any([DF <= 0 for DF in IDF.values()]):
        print("Surface is not stable!")

    # print upper bound for destabilising DF value
    if IDF[1] <= 0: show(DF1(xi) <= IDF[1].upper())
    if IDF[2] <= 0: show(DF2(xi) <= IDF[2].upper())
    if IDF[3] <= 0: show(DF3(xi) <= IDF[3].upper())
    if IDF[4] <= 0: show(DF4(xi) <= IDF[4].upper())
    else:
        print("Cannot determine stability")
        # Note, that "not a > 0" does not imply "a <= 0" for \
intervals

```

Stability test for test configurations:

$$\begin{aligned}
& \frac{(10\xi^2 + 4\xi - 1)e^{(3\xi)}}{36\xi^3} - \frac{(4(3\xi - 1)e^{(3\xi)} + 3)e^{(-\xi)}}{36\xi^3} \geq 0.07627603 \\
& \frac{(14\xi^2 + 2\xi - 5)e^{(3\xi)}}{36\xi^3} - \frac{(2(3\xi - 4)e^{(3\xi)} + 3)e^{(-\xi)}}{36\xi^3} \geq 0.07668713 \\
& -\frac{(14\xi^2 + 2\xi - 5)e^{(3\xi)}}{36\xi^3} + \frac{(12(\xi - 1)e^{(3\xi)} + 6\xi + 7)e^{(-\xi)}}{36\xi^3} \geq 0.1276748 \\
& \frac{(10\xi^2 + 4\xi - 1)e^{(3\xi)}}{36\xi^3} - \frac{(6\xi e^{(3\xi)} - 6\xi - 1)e^{(-\xi)}}{36\xi^3} \geq 0.2806380
\end{aligned}$$

Surface is stable!

---

No. 15: Degree 3 / Singularity type  $A_4A_1$ .

The combinatorial data is given by  $\square = [-1, 2]$  and  $\Phi_0(u) = \min\{\frac{u-1}{2}, 0\}$ ,  $\Phi_\infty(u) = \min\{-u, 0\}$ ,  $\Phi_1(u) = \frac{u-2}{3}$

```

# We are working with interval arithmetic with precision of 26 bit
# this fixes the precision e.g. for evaluations of exponential \
functions

```

```

RIF=RealIntervalField(26)

```

```

# The base polytope/interval
B=[-1,2]

```

```

# 3 PL functions on the interval
Phi1(u)=min_symbolic(1/2*u-1/2,0)
Phi2(u)=min_symbolic(0,-u)
Phi3(u)=1/3*u-2/3

```

```

# the degree of \bar Phi
degPhi=Phi1+Phi2+Phi3+2

```

```

print "The combinatorial data"

```

---

```

show(B)
show(Phi1)
show(Phi2)
show(Phi3)

```

The combinatorial data

$$\begin{aligned}
&[-1, 2] \\
&u \mapsto \min\left(\frac{1}{2}u - \frac{1}{2}, 0\right) \\
&u \mapsto \min(0, -u) \\
&u \mapsto \frac{1}{3}u - \frac{2}{3}
\end{aligned}$$

Step (i) obtain a closed form for  $F_{X,\xi}(1)$

For this we have to analytically solve the integral  $\int_{\square} u \deg \bar{\Phi}(u) e^{\xi u} du$ .

# The integral can be solved symbolically:

```

F(xi)=integral(degPhi(u)*u*exp(xi*u),u,-1,B[1])
show(F(xi))

```

$$-\frac{(3(\xi-2)e^{(2\xi)}+5\xi+10)e^{(-\xi)}}{6\xi^3} + \frac{2(2(\xi-1)e^{(2\xi)}+3)}{3\xi^3}$$

Step (ii) find an estimate for the soliton candidate vector field  $\xi$

# Solve numerically

```

sol=find_root(F,-10,10)
print "Numerical solution:",sol

```

```

# Choose upper and lower bound and
# hope that the exact solution lies in between
xi_1=sol-0.0000001
xi_2=xi_1+0.0000002

```

```

#define a real value xi0 between xi_1 and xi_2
# representing the exact solution
xi0=RIF(xi_1,xi_2)

```

```

# Check whether Intermediate value theorem guarantees a zero between
# xi_1 and xi_2, i.e evaluate F at xi_1 and xi_2 using interval \
  arithmetic
if RIF(F(xi_1)) < 0 and RIF(F(xi_2)) > 0:
    print "Interval containing solution:", xi0.str(style='\
brackets')

```

Numerical solution: -1.19618719651

Interval containing solution: [-1.19618732 .. -1.19618707]

Step (iii) & (iv) obtain closed forms for  $DF_{\xi}(X_{y,0,1})$  and plug in the estimate for  $\xi$

For every choice of  $y \in \mathbb{P}^1$  we have to symbolically solve the integrals  $\int_{\square} e^{u\xi} \cdot \left( (1 + \Phi_y(u))^2 - (1 + \sum_{z \neq y} \Phi_z(u)) \right)$ , which up to scaling with a positive constant coincide with  $DF_{\xi}(\mathcal{X}_{y,0,1})$ . Then we plug in the estimate



for  $\xi$  into the resulting expression.

```
#check for positivity of the DF invariant for our vector field xi
print("Stability test for test configurations:")

#storage for DF values (as intervals)
IDF={}

DF1(xi)=integral(exp(xi*u)*((Phi1+1)(u)^2-(Phi3+Phi2+1)(u)^2)/2,u\
, -1,B[1])
IDF[1]=RIF(DF1(xi0)) # evaluate DF1 at xi0 using interval arithmetic
show(DF1(xi) >= IDF[1].lower())

DF2(xi)=integral(exp(xi*u)*((Phi2+1)(u)^2-(Phi1+Phi3+1)(u)^2)/2,u\
, -1,B[1])
IDF[2]=RIF(DF2(xi0))
show(DF2(xi) >= IDF[2].lower())

DF3(xi)=integral(exp(xi*u)*((Phi3+1)(u)^2-(Phi1+Phi2+1)(u)^2)/2,u\
, -1,B[1])
IDF[3]=RIF(DF3(xi0))
show(DF3(xi) >= IDF[3].lower())

DF4(xi)=integral(exp(xi*u)*((1)^2-(Phi3+Phi2+Phi1+1)(u)^2)/2,u,-1,B\
[1])
IDF[4]=RIF(DF4(xi0))
show(DF4(xi) >= IDF[4].lower())

if all([DF > 0 for DF in IDF.values()]):
    print("Surface is stable!")
else:
    if any([DF <= 0 for DF in IDF.values()]):
        print("Surface is not stable!")

        # print upper bound for destabilising DF value
        if IDF[1] <= 0: show(DF1(xi) <= IDF[1].upper())
        if IDF[2] <= 0: show(DF2(xi) <= IDF[2].upper())
        if IDF[3] <= 0: show(DF3(xi) <= IDF[3].upper())
        if IDF[4] <= 0: show(DF4(xi) <= IDF[4].upper())
    else:
        print("Cannot determine stability")
        # Note, that "not a > 0" does not imply "a <= 0" for \
intervals
```

Stability test for test configurations:

$$-\frac{(9(2\xi-1)e^{(2\xi)}+5)e^{(-\xi)}}{36\xi^3} + \frac{2(3\xi-2)e^{(2\xi)}+3\xi+3}{9\xi^3} \geq 0.2231133$$

---


$$\frac{(3(4\xi - 7)e^{(2\xi)} + 30\xi + 25)e^{(-\xi)}}{36\xi^3} - \frac{2(3\xi - 4)e^{(2\xi)} + 9\xi + 9}{9\xi^3} \geq 0.5531086$$

$$\frac{(27\xi e^{(2\xi)} - 18(\xi + 2)e^\xi + 10)e^{(-\xi)}}{72\xi^3} + \frac{16(3\xi - 4)e^{(2\xi)} - 27(\xi - 2)e^\xi + 54\xi + 36}{72\xi^3} \geq 0.03862803$$

$$\frac{(3(5\xi - 8)e^{(2\xi)} - 18(\xi + 2)e^\xi + 60\xi + 50)e^{(-\xi)}}{72\xi^3} + \frac{16(3\xi - 2)e^{(2\xi)} - 27(\xi - 2)e^\xi + 6\xi - 12}{72\xi^3} \geq$$

0.8148505  
Surface is stable!

---

No. 17: Degree 3 / Singularity type  $D_5$ .

The combinatorial data is given by  $\square = [-1, 3]$  and  $\Phi_0(u) = \min\{\frac{u-2}{3}, 0\}$ ,  $\Phi_\infty(u) = \min\{\frac{u-1}{2}, 0\}$ ,  $\Phi_1(u) = \frac{-u-1}{2}$

```
# We are working with interval arithmetic with precision of 26 bit
# this fixes the precision e.g. for evaluations of exponential \
  functions
```

```
RIF=RealIntervalField(26)
```

```
# The base polytope/interval
B=[-1,3]
```

```
# 3 PL functions on the interval
```

```
Phi1(u)=min_symbolic((u-2)/3,0)
```

```
Phi2(u)=min_symbolic((u-1)/2,0)
```

```
Phi3(u)=(-u-1)/2
```

```
# the degree of \bar Phi
```

```
degPhi=Phi1+Phi2+Phi3+2
```

```
print "The combinatorial data"
```

```
show(B)
```

```
show(Phi1)
```

```
show(Phi2)
```

```
show(Phi3)
```

The combinatorial data

$[-1, 3]$

$u \mapsto \min\left(\frac{1}{3}u - \frac{2}{3}, 0\right)$

$u \mapsto \min\left(\frac{1}{2}u - \frac{1}{2}, 0\right)$

$u \mapsto -\frac{1}{2}u - \frac{1}{2}$

Step (i) obtain a closed form for  $F_{X,\xi}(1)$

For this we have to analytically solve the integral  $\int_{\square} u \deg \bar{\Phi}(u) e^{\xi u} du$ .

```
# The integral can be solved symbolically:
```

---

```
F(xi)=integral(degPhi(u)*u*exp(xi*u),u,-1,B[1])
show(F(xi))
```

$$\frac{(3\xi - 2)e^{(3\xi)}}{2\xi^3} - \frac{(4(\xi - 1)e^{(3\xi)} + 3(\xi - 2)e^{(2\xi)} + 2\xi + 4)e^{(-\xi)}}{6\xi^3}$$

Step (ii) find an estimate for the soliton candidate vector field  $\xi$

```
# Solve numerically
sol=find_root(F,-10,10)
print "Numerical solution:",sol

# Choose upper and lower bound and
# hope that the exact solution lies in between
xi_1=sol-0.0000001
xi_2=xi_1+0.0000002

#define a real value xi0 between xi_1 and xi_2
# representing the exact solution
xi0=RIF(xi_1,xi_2)

# Check whether Intermediate value theorem guarantees a zero between
# xi_1 and xi_2, i.e evaluate F at xi_1 and xi_2 using interval \
arithmetic
if RIF(F(xi_1)) < 0 and RIF(F(xi_2)) > 0:
    print "Interval containing solution:", xi0.str(style='\
brackets')
```

Numerical solution: -1.83879135601

Interval containing solution: [-1.83879146 .. -1.83879125]

Step (iii) & (iv) obtain closed forms for  $DF_\xi(X_{y,0,1})$  and plug in the estimate for  $\xi$

For every choice of  $y \in \mathbb{P}^1$  we have to symbolically solve the integrals  $\int_{\square} e^{u\xi} \cdot ((1 + \Phi_y(u))^2 - (1 + \sum_{z \neq y} \Phi_z(u)))$  which up to scaling with a positive constant coincide with  $DF_\xi(\mathcal{X}_{y,0,1})$ . Then we plug in the estimate for  $\xi$  into the resulting expression.

```
#check for positivity of the DF invariant for our vector field xi
print("Stability test for test configurations:")

#storage for DF values (as intervals)
IDF={}

DF1(xi)=integral(exp(xi*u)*((Phi1+1)(u)^2-(Phi3+Phi2+1)(u)^2)/2,u\
,-1,B[1])
IDF[1]=RIF(DF1(xi0)) # evaluate DF1 at xi0 using interval arithmetic
show(DF1(xi) >= IDF[1].lower())

DF2(xi)=integral(exp(xi*u)*((Phi2+1)(u)^2-(Phi1+Phi3+1)(u)^2)/2,u\
,-1,B[1])
```

---

```

IDF[2]=RIF(DF2(xi0))
show(DF2(xi) >= IDF[2].lower())

DF3(xi)=integral(exp(xi*u)*((Phi3+1)(u)^2-(Phi1+Phi2+1)(u)^2)/2,u\
,-1,B[1])
IDF[3]=RIF(DF3(xi0))
show(DF3(xi) >= IDF[3].lower())

DF4(xi)=integral(exp(xi*u)*((1)^2-(Phi3+Phi2+Phi1+1)(u)^2)/2,u,-1,B\
[1])
IDF[4]=RIF(DF4(xi0))
show(DF4(xi) >= IDF[4].lower())

if all([DF > 0 for DF in IDF.values()]):
    print("Surface is stable!")
else:
    if any([DF <= 0 for DF in IDF.values()]):
        print("Surface is not stable!")

        # print upper bound for destabilising DF value
        if IDF[1] <= 0: show(DF1(xi) <= IDF[1].upper())
        if IDF[2] <= 0: show(DF2(xi) <= IDF[2].upper())
        if IDF[3] <= 0: show(DF3(xi) <= IDF[3].upper())
        if IDF[4] <= 0: show(DF4(xi) <= IDF[4].upper())
    else:
        print("Cannot determine stability")
        # Note, that "not a > 0" does not imply "a <= 0" for \
        intervals

Stability test for test configurations:

$$\frac{(2\xi-1)e^{(3\xi)}}{4\xi^3} - \frac{(4(3\xi-1)e^{(3\xi)}-9e^{(2\xi)}+4)e^{(-\xi)}}{36\xi^3} \geq 0.1038101$$


$$\frac{(2\xi-1)e^{(3\xi)}}{4\xi^3} - \frac{(2(3\xi-4)e^{(3\xi)}+9(2\xi-1)e^{(2\xi)}+8)e^{(-\xi)}}{36\xi^3} \geq 0.1934829$$


$$\frac{((27\xi-14)e^{(3\xi)}+30(\xi-1)e^{(2\xi)}+24\xi+32)e^{(-\xi)}}{72\xi^3} - \frac{6(2\xi-1)e^{(3\xi)}+(\xi-2)e^{(2\xi)}+2(\xi+2)e^\xi}{24\xi^3} \geq 0.2032122$$


$$- \frac{((9\xi-10)e^{(3\xi)}+6(\xi-1)e^{(2\xi)}-24\xi-8)e^{(-\xi)}}{72\xi^3} + \frac{6(2\xi-1)e^{(3\xi)}-(\xi-2)e^{(2\xi)}-2(\xi+2)e^\xi}{24\xi^3} \geq 0.5005054$$

Surface is stable!

```

---

No. 19: Degree 3 / Singularity type  $D_4$ .

The combinatorial data is given by  $\square = [-1, 2]$  and  $\Phi_0(u) = \min\{-u, \frac{-u-1}{2}\}$ ,  $\Phi_\infty(u) = \min\{0, \frac{u-1}{2}\}$ ,  $\Phi_1(u) = \min\{0, \frac{u-1}{2}\}$

# We are working with interval arithmetic with precision of 26 bit  
# this fixes the precision e.g. for evaluations of exponential \

---

```

functions
RIF=RealIntervalField(26)

# The base polytope/interval
B=[-1,2]

# 3 PL functions on the interval
Phi1(u)=min_symbolic((-u-1)/2,-u)
Phi2(u)=min_symbolic((u-1)/2,0)
Phi3(u)=min_symbolic((u-1)/2,0)

# the degree of \bar Phi
degPhi=Phi1+Phi2+Phi3+2

print "The combinatorial data"
show(B)
show(Phi1)
show(Phi2)
show(Phi3)

```

The combinatorial data

$$\begin{aligned}
 &[-1, 2] \\
 &u \mapsto \min\left(-\frac{1}{2}u - \frac{1}{2}, -u\right) \\
 &u \mapsto \min\left(\frac{1}{2}u - \frac{1}{2}, 0\right) \\
 &u \mapsto \min\left(\frac{1}{2}u - \frac{1}{2}, 0\right)
 \end{aligned}$$

Step (i) obtain a closed form for  $F_{X,\xi}(1)$

For this we have to analytically solve the integral  $\int_{\square} u \deg \bar{\Phi}(u) e^{\xi u} du$ .

# The integral can be solved symbolically:

```

F(xi)=integral(degPhi(u)*u*exp(xi*u),u,-1,B[1])
show(F(xi))

```

$$-\frac{((2\xi^2 - \xi - 2)e^{(2\xi)} + \xi + 2)e^{(-\xi)}}{2\xi^3} + \frac{2(\xi - 1)e^{(2\xi)} + (\xi^2 - 2\xi + 2)e^{\xi}}{\xi^3}$$

Step (ii) find an estimate for the soliton candidate vector field  $\xi$

```

# Solve numerically
sol=find_root(F,-10,10)
print "Numerical solution:",sol

# Choose upper and lower bound and
# hope that the exact solution lies in between
xi_1=sol-0.0000001
xi_2=xi_1+0.0000002

```

---

```

# define a real value xi0 between xi_1 and xi_2
# representing the exact solution
xi0=RIF(xi_1,xi_2)

# Check whether Intermediate value theorem guarantees a zero between
# xi_1 and xi_2, i.e evaluate F at xi_1 and xi_2 using interval \
arithmetic
if RIF(F(xi_1)) < 0 and RIF(F(xi_2)) > 0:
    print "Interval containing solution:", xi0.str(style='\
brackets')

```

Numerical solution: -1.69131741884

Interval containing solution: [-1.69131753 .. -1.69131729]

Step (iii) & (iv) obtain closed forms for  $DF_\xi(X_{y,0,1})$  and plug in the estimate for  $\xi$

For every choice of  $y \in \mathbb{P}^1$  we have to symbolically solve the integrals  $\int_{\square} e^{u\xi} \cdot ((1 + \Phi_y(u))^2 - (1 + \sum_{z \neq y} \Phi_z(u)))$  which up to scaling with a positive constant coincide with  $DF_\xi(\mathcal{X}_{y,0,1})$ . Then we plug in the estimate for  $\xi$  into the resulting expression.

```

#check for positivity of the DF invariant for our vector field xi
print("Stability test for test configurations:")

#storage for DF values (as intervals)
IDF={}

DF1(xi)=integral(exp(xi*u)*((Phi1+1)(u)^2-(Phi3+Phi2+1)(u)^2)/2,u\
, -1,B[1])
IDF[1]=RIF(DF1(xi0)) # evaluate DF1 at xi0 using interval arithmetic
show(DF1(xi) >= IDF[1].lower())

DF2(xi)=integral(exp(xi*u)*((Phi2+1)(u)^2-(Phi1+Phi3+1)(u)^2)/2,u\
, -1,B[1])
IDF[2]=RIF(DF2(xi0))
show(DF2(xi) >= IDF[2].lower())

DF3(xi)=integral(exp(xi*u)*((Phi3+1)(u)^2-(Phi1+Phi2+1)(u)^2)/2,u\
, -1,B[1])
IDF[3]=RIF(DF3(xi0))
show(DF3(xi) >= IDF[3].lower())

DF4(xi)=integral(exp(xi*u)*((1)^2-(Phi3+Phi2+Phi1+1)(u)^2)/2,u,-1,B\
[1])
IDF[4]=RIF(DF4(xi0))
show(DF4(xi) >= IDF[4].lower())

if all([DF > 0 for DF in IDF.values()]):
    print("Surface is stable!")
else:

```

---

```

if any([DF <= 0 for DF in IDF.values()]):
    print("Surface is not stable!")

# print upper bound for destabilising DF value
if IDF[1] <= 0: show(DF1(xi) <= IDF[1].upper())
if IDF[2] <= 0: show(DF2(xi) <= IDF[2].upper())
if IDF[3] <= 0: show(DF3(xi) <= IDF[3].upper())
if IDF[4] <= 0: show(DF4(xi) <= IDF[4].upper())
else:
    print("Cannot determine stability")
    # Note, that "not a > 0" does not imply "a <= 0" for \
    intervals

```

Stability test for test configurations:

$$\begin{aligned}
& -\frac{((2\xi^2 - 4\xi + 3)e^{(2\xi)} - 2\xi - 3)e^{(-\xi)}}{4\xi^3} - \frac{2(\xi - 1)e^{(2\xi)} - (\xi^2 - 2)e^\xi}{2\xi^3} \geq 0.2194796 \\
& \frac{((2\xi^2 - 2\xi + 1)e^{(2\xi)} - 1)e^{(-\xi)}}{4\xi^3} + \frac{2(\xi - 1)e^{(2\xi)} - (\xi^2 - 2)e^\xi}{2\xi^3} \geq 0.2194797 \\
& \frac{((2\xi^2 - 2\xi + 1)e^{(2\xi)} - 1)e^{(-\xi)}}{4\xi^3} + \frac{2(\xi - 1)e^{(2\xi)} - (\xi^2 - 2)e^\xi}{2\xi^3} \geq 0.2194797 \\
& \frac{((2\xi^2 - 1)e^{(2\xi)} + 2\xi + 1)e^{(-\xi)}}{4\xi^3} + \frac{2(\xi - 1)e^{(2\xi)} - (\xi^2 - 2)e^\xi}{2\xi^3} \geq 0.6584392
\end{aligned}$$

Surface is stable!

---

No. 20: Degree 3 / Singularity type  $2A_1A_3$ .

The combinatorial data is given by  $\square = [-1, 1]$  and  $\Phi_0(u) = \min\{0, u\}$ ,  $\Phi_\infty(u) = \frac{u-1}{2}$ ,  $\Phi_1(u) = \frac{-u-1}{2}$

```

# We are working with interval arithmetic with precision of 26 bit
# this fixes the precision e.g. for evaluations of exponential \
  functions

```

```
RIF=RealIntervalField(26)
```

```

# The base polytope/interval
B=[-1,1]

```

```
# 3 PL functions on the interval
```

```
Phi1(u)=min_symbolic(0,u)
```

```
Phi2(u)=(u-1)/2
```

```
Phi3(u)=(-u-1)/2
```

```
# the degree of \bar Phi
```

```
degPhi=Phi1+Phi2+Phi3+2
```

```
print "The combinatorial data"
```

```
show(B)
```

```
show(Phi1)
```

---

```
show(Phi2)
```

```
show(Phi3)
```

The combinatorial data

$$[-1, 1]$$
$$u \mapsto \min(0, u)$$
$$u \mapsto \frac{1}{2}u - \frac{1}{2}$$
$$u \mapsto -\frac{1}{2}u - \frac{1}{2}$$

Step (i) obtain a closed form for  $F_{X,\xi}(1)$

For this we have to analytically solve the integral  $\int_{\square} u \deg \bar{\Phi}(u) e^{\xi u} du$ .

```
# The integral can be solved symbolically:
```

```
F(xi)=integral(degPhi(u)*u*exp(xi*u),u,-1,B[1])
```

```
show(F(xi))
```

$$\frac{(\xi - 1)e^{\xi}}{\xi^2} - \frac{(\xi - 2e^{\xi} + 2)e^{(-\xi)}}{\xi^3}$$

Step (ii) find an estimate for the soliton candidate vector field  $\xi$

```
# Solve numerically
```

```
sol=find_root(F,-10,10)
```

```
print "Numerical solution:",sol
```

```
# Choose upper and lower bound and
```

```
# hope that the exact solution lies in between
```

```
xi_1=sol-0.0000001
```

```
xi_2=xi_1+0.0000002
```

```
#define a real value xi0 between xi_1 and xi_2
```

```
# representing the exact solution
```

```
xi0=RIF(xi_1,xi_2)
```

```
# Check whether Intermediate value theorem guarantees a zero between
```

```
# xi_1 and xi_2, i.e evaluate F at xi_1 and xi_2 using interval \
```

```
arithmetic
```

```
if RIF(F(xi_1)) < 0 and RIF(F(xi_2)) > 0:
```

```
    print "Interval containing solution:", xi0.str(style='\
```

```
brackets')
```

Numerical solution: -0.944683075826

Interval containing solution: [-0.944683180 .. -0.944682970]

Step (iii) & (iv) obtain closed forms for  $DF_{\xi}(X_{y,0,1})$  and plug in the estimate for  $\xi$

For every choice of  $y \in \mathbb{P}^1$  we have to symbolically solve the integrals  $\int_{\square} e^{u\xi} \cdot \left( (1 + \Phi_y(u))^2 - (1 + \sum_{z \neq y} \Phi_z(u)) \right)$ , which up to scaling with a positive constant coincide with  $DF_{\xi}(\mathcal{X}_{y,0,1})$ . Then we plug in the estimate for  $\xi$  into the resulting expression.



---

```

#check for positivity of the DF invariant for our vector field xi
print("Stability test for test configurations:")

#storage for DF values (as intervals)
IDF={}

DF1(xi)=integral(exp(xi*u)*((Phi1+1)(u)^2-(Phi3+Phi2+1)(u)^2)/2,u\
, -1 ,B[1])
IDF[1]=RIF(DF1(xi0)) # evaluate DF1 at xi0 using interval arithmetic
show(DF1(xi) >= IDF[1].lower())

DF2(xi)=integral(exp(xi*u)*((Phi2+1)(u)^2-(Phi1+Phi3+1)(u)^2)/2,u\
, -1 ,B[1])
IDF[2]=RIF(DF2(xi0))
show(DF2(xi) >= IDF[2].lower())

DF3(xi)=integral(exp(xi*u)*((Phi3+1)(u)^2-(Phi1+Phi2+1)(u)^2)/2,u\
, -1 ,B[1])
IDF[3]=RIF(DF3(xi0))
show(DF3(xi) >= IDF[3].lower())

DF4(xi)=integral(exp(xi*u)*((1)^2-(Phi3+Phi2+Phi1+1)(u)^2)/2,u, -1 ,B\
[1])
IDF[4]=RIF(DF4(xi0))
show(DF4(xi) >= IDF[4].lower())

if all([DF > 0 for DF in IDF.values()]):
    print("Surface is stable!")
else:
    if any([DF <= 0 for DF in IDF.values()]):
        print("Surface is not stable!")

        # print upper bound for destabilising DF value
        if IDF[1] <= 0: show(DF1(xi) <= IDF[1].upper())
        if IDF[2] <= 0: show(DF2(xi) <= IDF[2].upper())
        if IDF[3] <= 0: show(DF3(xi) <= IDF[3].upper())
        if IDF[4] <= 0: show(DF4(xi) <= IDF[4].upper())
    else:
        print("Cannot determine stability")
        # Note, that "not a > 0" does not imply "a <= 0" for \
intervals

```

Stability test for test configurations:

$$\frac{e^\xi}{2\xi} - \frac{((\xi-1)e^\xi + 1)e^{(-\xi)}}{\xi^3} \geq 0.5383074$$

$$\frac{(\xi-1)e^\xi}{2\xi^2} + \frac{1}{2\xi^2} \geq 0.1366506$$

---


$$-\frac{(\xi-1)e^\xi}{2\xi^2} + \frac{((\xi-4)e^\xi + 2\xi + 4)e^{(-\xi)}}{2\xi^3} \geq 0.1366499$$

$$\frac{e^\xi}{2\xi} + \frac{(\xi - e^\xi + 1)e^{(-\xi)}}{\xi^3} \geq 0.8116092$$

Surface is stable!

---

No. 21: Degree 4 / Singularity type  $D_5$ .

The combinatorial data is given by  $\square = [-1, 5]$  and  $\Phi_0(u) = \min\{\frac{u-1}{2}, 0\}$ ,  $\Phi_\infty(u) = \frac{u-2}{3}$ ,  $\Phi_1(u) = \frac{-u-1}{2}$

```
# We are working with interval arithmetic with precision of 26 bit
# this fixes the precision e.g. for evaluations of exponential \
  functions
```

```
RIF=RealIntervalField(26)
```

```
# The base polytope/interval
B=[-1,5]
```

```
# 3 PL functions on the interval
```

```
Phi1(u)=min_symbolic((u-1)/2,0)
```

```
Phi2(u)=(u-2)/3
```

```
Phi3(u)=(-u-1)/2
```

```
# the degree of \bar Phi
```

```
degPhi=Phi1+Phi2+Phi3+2
```

```
print "The combinatorial data"
```

```
show(B)
```

```
show(Phi1)
```

```
show(Phi2)
```

```
show(Phi3)
```

The combinatorial data

$[-1, 5]$

$u \mapsto \min\left(\frac{1}{2}u - \frac{1}{2}, 0\right)$

$u \mapsto \frac{1}{3}u - \frac{2}{3}$

$u \mapsto -\frac{1}{2}u - \frac{1}{2}$

Step (i) obtain a closed form for  $F_{X,\xi}(1)$

For this we have to analytically solve the integral  $\int_{\square} u \deg \bar{\Phi}(u) e^{\xi u} du$ .

```
# The integral can be solved symbolically:
```

```
F(xi)=integral(degPhi(u)*u*exp(xi*u),u,-1,B[1])
```

```
show(F(xi))
```

$$\frac{(5\xi - 2)e^{(5\xi)}}{6\xi^3} - \frac{(3(\xi - 2)e^{(2\xi)} + 2\xi + 4)e^{(-\xi)}}{6\xi^3}$$

Step (ii) find an estimate for the soliton candidate vector field  $\xi$

```
# Solve numerically
sol=find_root(F,-10,10)
print "Numerical solution:",sol

# Choose upper and lower bound and
# hope that the exact solution lies in between
xi_1=sol-0.0000001
xi_2=xi_1+0.0000002

#define a real value xi0 between xi_1 and xi_2
# representing the exact solution
xi0=RIF(xi_1,xi_2)

# Check whether Intermediate value theorem guarantees a zero between
# xi_1 and xi_2, i.e evaluate F at xi_1 and xi_2 using interval \
arithmetic
if RIF(F(xi_1)) < 0 and RIF(F(xi_2)) > 0:
    print "Interval containing solution:", xi0.str(style='\
brackets')
```

Numerical solution: -1.85969017295

Interval containing solution: [-1.85969028 .. -1.85969007]

Step (iii) & (iv) obtain closed forms for  $DF_\xi(X_{y,0,1})$  and plug in the estimate for  $\xi$

For every choice of  $y \in \mathbb{P}^1$  we have to symbolically solve the integrals  $\int_{\square} e^{u\xi} \cdot ((1 + \Phi_y(u))^2 - (1 + \sum_{z \neq y} \Phi_z(u)))$  which up to scaling with a positive constant coincide with  $DF_\xi(\mathcal{X}_{y,0,1})$ . Then we plug in the estimate for  $\xi$  into the resulting expression.

```
#check for positivity of the DF invariant for our vector field xi
print("Stability test for test configurations:")

#storage for DF values (as intervals)
IDF={}

DF1(xi)=integral(exp(xi*u)*((Phi1+1)(u)^2-(Phi3+Phi2+1)(u)^2)/2,u\
, -1,B[1])
IDF[1]=RIF(DF1(xi0)) # evaluate DF1 at xi0 using interval arithmetic
show(DF1(xi) >= IDF[1].lower())

DF2(xi)=integral(exp(xi*u)*((Phi2+1)(u)^2-(Phi1+Phi3+1)(u)^2)/2,u\
, -1,B[1])
IDF[2]=RIF(DF2(xi0))
show(DF2(xi) >= IDF[2].lower())
```

---

```

DF3(xi)=integral(exp(xi*u)*((Phi3+1)(u)^2-(Phi1+Phi2+1)(u)^2)/2,u\
    ,-1,B[1])
IDF[3]=RIF(DF3(xi0))
show(DF3(xi) >= IDF[3].lower())

DF4(xi)=integral(exp(xi*u)*((1)^2-(Phi3+Phi2+Phi1+1)(u)^2)/2,u,-1,B\
    [1])
IDF[4]=RIF(DF4(xi0))
show(DF4(xi) >= IDF[4].lower())

if all([DF > 0 for DF in IDF.values()]):
    print("Surface is stable!")
else:
    if any([DF <= 0 for DF in IDF.values()]):
        print("Surface is not stable!")

        # print upper bound for destabilising DF value
        if IDF[1] <= 0: show(DF1(xi) <= IDF[1].upper())
        if IDF[2] <= 0: show(DF2(xi) <= IDF[2].upper())
        if IDF[3] <= 0: show(DF3(xi) <= IDF[3].upper())
        if IDF[4] <= 0: show(DF4(xi) <= IDF[4].upper())
    else:
        print("Cannot determine stability")
        # Note, that "not a > 0" does not imply "a <= 0" for \
        intervals

```

Stability test for test configurations:

$$\begin{aligned}
& \frac{(6\xi - 1)e^{(5\xi)}}{36\xi^3} - \frac{(9(2\xi - 1)e^{(2\xi)} + 8)e^{(-\xi)}}{36\xi^3} \geq 0.1933190 \\
& \frac{(12\xi - 5)e^{(5\xi)}}{36\xi^3} + \frac{(9e^{(2\xi)} - 4)e^{(-\xi)}}{36\xi^3} \geq 0.1048980 \\
& -\frac{(12\xi - 5)e^{(5\xi)}}{36\xi^3} + \frac{(3(4\xi - 7)e^{(2\xi)} + 12\xi + 16)e^{(-\xi)}}{36\xi^3} \geq 0.2043036 \\
& \frac{(6\xi - 1)e^{(5\xi)}}{36\xi^3} - \frac{(3(2\xi + 1)e^{(2\xi)} - 12\xi - 4)e^{(-\xi)}}{36\xi^3} \geq 0.5025207
\end{aligned}$$

Surface is stable!

---

No. 22: Degree 4 / Singularity type  $A_3A_1$ .

The combinatorial data is given by  $\square = [-1, 2]$  and  $\Phi_0(u) = \min\{0, u\}$ ,  $\Phi_\infty(u) = \min\{u, u\}$ ,  $\Phi_1(u) = \frac{-2u-2}{3}$

```

# We are working with interval arithmetic with precision of 26 bit
# this fixes the precision e.g. for evaluations of exponential \
    functions
RIF=RealIntervalField(26)

```

---

```
# The base polytope/interval
B=[-1,2]
```

```
# 3 PL functions on the interval
Phi1(u)=min_symbolic(0,u)
Phi2(u)=min_symbolic(0,u)
Phi3(u)=-2/3*u-2/3
```

```
# the degree of \bar Phi
degPhi=Phi1+Phi2+Phi3+2
```

```
print "The combinatorial data"
show(B)
show(Phi1)
show(Phi2)
show(Phi3)
```

The combinatorial data

```
[-1, 2]
u ↦ min(0, u)
u ↦ min(0, u)
u ↦ - $\frac{2}{3}u - \frac{2}{3}$ 
```

Step (i) obtain a closed form for  $F_{X,\xi}(1)$

For this we have to analytically solve the integral  $\int_{\square} u \deg \bar{\Phi}(u) e^{\xi u} du$ .

```
# The integral can be solved symbolically:
```

```
F(xi)=integral(degPhi(u)*u*exp(xi*u),u,-1,B[1])
show(F(xi))
```

$$\frac{4(\xi-1)e^{(2\xi)}}{3\xi^3} - \frac{4(\xi-3e^{\xi}+2)e^{(-\xi)}}{3\xi^3}$$

Step (ii) find an estimate for the soliton candidate vector field  $\xi$

```
# Solve numerically
```

```
sol=find_root(F,-10,10)
print "Numerical solution:",sol
```

```
# Choose upper and lower bound and
```

```
# hope that the exact solution lies in between
```

```
xi_1=sol-0.0000001
xi_2=xi_1+0.0000002
```

```
#define a real value xi0 between xi_1 and xi_2
```

```
# representing the exact solution
```

```
xi0=RIF(xi_1,xi_2)
```

```
# Check whether Intermediate value theorem guarantees a zero between
```

---

```
# xi_1 and xi_2, i.e evaluate F at xi_1 and xi_2 using interval \
arithmetic
if RIF(F(xi_1)) < 0 and RIF(F(xi_2)) > 0:
    print "Interval containing solution:", xi0.str(style='\
brackets')
```

Numerical solution: -0.97052220918

Interval containing solution: [-0.970522315 .. -0.970522105]

Step (iii) & (iv) obtain closed forms for  $DF_\xi(X_{y,0,1})$  and plug in the estimate for  $\xi$

For every choice of  $y \in \mathbb{P}^1$  we have to symbolically solve the integrals  $\int_{\square} e^{u\xi} \cdot ((1 + \Phi_y(u))^2 - (1 + \sum_{z \neq y} \Phi_z(u)))$  which up to scaling with a positive constant coincide with  $DF_\xi(\mathcal{X}_{y,0,1})$ . Then we plug in the estimate for  $\xi$  into the resulting expression.

```
#check for positivity of the DF invariant for our vector field xi
print("Stability test for test configurations:")
```

```
#storage for DF values (as intervals)
IDF={}
```

```
DF1(xi)=integral(exp(xi*u)*((Phi1+1)(u)^2-(Phi3+Phi2+1)(u)^2)/2,u\
, -1,B[1])
IDF[1]=RIF(DF1(xi0)) # evaluate DF1 at xi0 using interval arithmetic
show(DF1(xi) >= IDF[1].lower())
```

```
DF2(xi)=integral(exp(xi*u)*((Phi2+1)(u)^2-(Phi1+Phi3+1)(u)^2)/2,u\
, -1,B[1])
IDF[2]=RIF(DF2(xi0))
show(DF2(xi) >= IDF[2].lower())
```

```
DF3(xi)=integral(exp(xi*u)*((Phi3+1)(u)^2-(Phi1+Phi2+1)(u)^2)/2,u\
, -1,B[1])
IDF[3]=RIF(DF3(xi0))
show(DF3(xi) >= IDF[3].lower())
```

```
DF4(xi)=integral(exp(xi*u)*((1)^2-(Phi3+Phi2+Phi1+1)(u)^2)/2,u,-1,B\
[1])
IDF[4]=RIF(DF4(xi0))
show(DF4(xi) >= IDF[4].lower())
```

```
if all([DF > 0 for DF in IDF.values()]):
    print("Surface is stable!")
else:
    if any([DF <= 0 for DF in IDF.values()]):
        print("Surface is not stable!")
```

```
# print upper bound for destabilising DF value
if IDF[1] <= 0: show(DF1(xi) <= IDF[1].upper())
```

---

```

    if IDF[2] <= 0: show(DF2(xi) <= IDF[2].upper())
    if IDF[3] <= 0: show(DF3(xi) <= IDF[3].upper())
    if IDF[4] <= 0: show(DF4(xi) <= IDF[4].upper())
else:
    print("Cannot determine stability")
    # Note, that "not a > 0" does not imply "a <= 0" for \
intervals

```

Stability test for test configurations:

$$\frac{2(3\xi - 2)e^{(2\xi)}}{9\xi^3} - \frac{2(3(\xi - 2)e^\xi + 4)e^{(-\xi)}}{9\xi^3} \geq 0.5714598$$

$$\frac{2(3\xi - 2)e^{(2\xi)}}{9\xi^3} - \frac{2(3(\xi - 2)e^\xi + 4)e^{(-\xi)}}{9\xi^3} \geq 0.5714598$$

$$-\frac{2(3\xi - 2)e^{(2\xi)}}{9\xi^3} + \frac{2(9(\xi - 2)e^\xi + 6\xi + 16)e^{(-\xi)}}{9\xi^3} \geq (-0.2018673)$$

$$\frac{2(3\xi - 2)e^{(2\xi)}}{9\xi^3} + \frac{2(3(\xi - 2)e^\xi + 6\xi + 8)e^{(-\xi)}}{9\xi^3} \geq 0.9410544$$

Surface is not stable!

$$-\frac{2(3\xi - 2)e^{(2\xi)}}{9\xi^3} + \frac{2(9(\xi - 2)e^\xi + 6\xi + 16)e^{(-\xi)}}{9\xi^3} \leq (-0.2018636)$$

---

No. 23: Degree 4 / Singularity type  $D_4$ .

The combinatorial data is given by  $\square = [-1, 3]$  and  $\Phi_0(u) = \min\{\frac{u-1}{2}, 0\}$ ,  $\Phi_\infty(u) = \min\{\frac{u-1}{2}, 0\}$ ,  $\Phi_1(u) = \frac{-u-1}{2}$

```

# We are working with interval arithmetic with precision of 26 bit
# this fixes the precision e.g. for evaluations of exponential \
functions

```

```

RIF=RealIntervalField(26)

```

```

# The base polytope/interval

```

```

B=[-1,3]

```

```

# 3 PL functions on the interval

```

```

Phi1(u)=min_symbolic((u-1)/2,0)

```

```

Phi2(u)=min_symbolic((u-1)/2,0)

```

```

Phi3(u)=(-u-1)/2

```

```

# the degree of \bar Phi

```

```

degPhi=Phi1+Phi2+Phi3+2

```

```

print "The combinatorial data"

```

```

show(B)

```

```

show(Phi1)

```

```

show(Phi2)

```

```

show(Phi3)

```

The combinatorial data

```

[-1, 3]

```

$$u \mapsto \min\left(\frac{1}{2}u - \frac{1}{2}, 0\right)$$

$$u \mapsto \min\left(\frac{1}{2}u - \frac{1}{2}, 0\right)$$

$$u \mapsto -\frac{1}{2}u - \frac{1}{2}$$

Step (i) obtain a closed form for  $F_{X,\xi}(1)$

For this we have to analytically solve the integral  $\int_{\square} u \deg \bar{\Phi}(u) e^{\xi u} du$ .

# The integral can be solved symbolically:

```
F(xi)=integral(degPhi(u)*u*exp(xi*u),u,-1,B[1])
show(F(xi))
```

$$\frac{(3\xi - 2)e^{(3\xi)}}{2\xi^3} - \frac{(2(\xi - 2)e^{(2\xi)} + \xi + 2)e^{(-\xi)}}{2\xi^3}$$

Step (ii) find an estimate for the soliton candidate vector field  $\xi$

# Solve numerically

```
sol=find_root(F,-10,10)
print "Numerical solution:",sol
```

# Choose upper and lower bound and

# hope that the exact solution lies in between

```
xi_1=sol-0.0000001
xi_2=xi_1+0.0000002
```

#define a real value xi0 between xi\_1 and xi\_2

# representing the exact solution

```
xi0=RIF(xi_1,xi_2)
```

# Check whether Intermediate value theorem guarantees a zero between  
# xi\_1 and xi\_2, i.e evaluate F at xi\_1 and xi\_2 using interval \

```
arithmetic
if RIF(F(xi_1)) < 0 and RIF(F(xi_2)) > 0:
```

```
    print "Interval containing solution:", xi0.str(style='\
brackets')
```

Numerical solution: -1.79675598472

Interval containing solution: [-1.79675609 .. -1.79675588]

Step (iii) & (iv) obtain closed forms for  $DF_{\xi}(X_{y,0,1})$  and plug in the estimate for  $\xi$

For every choice of  $y \in \mathbb{P}^1$  we have to symbolically solve the integrals  $\int_{\square} e^{u\xi} \cdot ((1 + \Phi_y(u))^2 - (1 + \sum_{z \neq y} \Phi_z(u)))$  which up to scaling with a positive constant coincide with  $DF_{\xi}(\mathcal{X}_{y,0,1})$ . Then we plug in the estimate for  $\xi$  into the resulting expression.

```
#check for positivity of the DF invariant for our vector field xi
print("Stability test for test configurations:")
```



---

```

#storage for DF values (as intervals)
IDF={}

DF1(xi)=integral(exp(xi*u)*((Phi1+1)(u)^2-(Phi3+Phi2+1)(u)^2)/2,u\
,-1,B[1])
IDF[1]=RIF(DF1(xi0)) # evaluate DF1 at xi0 using interval arithmetic
show(DF1(xi) >= IDF[1].lower())

DF2(xi)=integral(exp(xi*u)*((Phi2+1)(u)^2-(Phi1+Phi3+1)(u)^2)/2,u\
,-1,B[1])
IDF[2]=RIF(DF2(xi0))
show(DF2(xi) >= IDF[2].lower())

DF3(xi)=integral(exp(xi*u)*((Phi3+1)(u)^2-(Phi1+Phi2+1)(u)^2)/2,u\
,-1,B[1])
IDF[3]=RIF(DF3(xi0))
show(DF3(xi) >= IDF[3].lower())

DF4(xi)=integral(exp(xi*u)*((1)^2-(Phi3+Phi2+Phi1+1)(u)^2)/2,u,-1,B\
[1])
IDF[4]=RIF(DF4(xi0))
show(DF4(xi) >= IDF[4].lower())

if all([DF > 0 for DF in IDF.values()]):
    print("Surface is stable!")
else:
    if any([DF <= 0 for DF in IDF.values()]):
        print("Surface is not stable!")

    # print upper bound for destabilising DF value
    if IDF[1] <= 0: show(DF1(xi) <= IDF[1].upper())
    if IDF[2] <= 0: show(DF2(xi) <= IDF[2].upper())
    if IDF[3] <= 0: show(DF3(xi) <= IDF[3].upper())
    if IDF[4] <= 0: show(DF4(xi) <= IDF[4].upper())
    else:
        print("Cannot determine stability")
        # Note, that "not a > 0" does not imply "a <= 0" for \
intervals

```

Stability test for test configurations:

$$\begin{aligned}
& \frac{(2\xi-1)e^{(3\xi)}}{4\xi^3} - \frac{(2(\xi-1)e^{(2\xi)}+1)e^{(-\xi)}}{4\xi^3} \geq 0.2208160 \\
& \frac{(2\xi-1)e^{(3\xi)}}{4\xi^3} - \frac{(2(\xi-1)e^{(2\xi)}+1)e^{(-\xi)}}{4\xi^3} \geq 0.2208160 \\
& -\frac{(2\xi-1)e^{(3\xi)}}{4\xi^3} + \frac{(4(\xi-1)e^{(2\xi)}+2\xi+3)e^{(-\xi)}}{4\xi^3} \geq 0.2333050 \\
& \frac{(2\xi-1)e^{(3\xi)}}{4\xi^3} + \frac{(2\xi+1)e^{(-\xi)}}{4\xi^3} \geq 0.6749371
\end{aligned}$$

---

Surface is stable!

---

No. 24: Degree 4 / Singularity type  $A_4$ .

The combinatorial data is given by  $\square = [-1, 3]$  and  $\Phi_0(u) = \min\{\frac{u-2}{3}, 0\}$ ,  $\Phi_\infty(u) = \min\{-u, 0\}$ ,  $\Phi_1(u) = \frac{-u-1}{2}$

```
# We are working with interval arithmetic with precision of 26 bit
# this fixes the precision e.g. for evaluations of exponential \
  functions
```

```
RIF=RealIntervalField(26)
```

```
# The base polytope/interval
B=[-1,3]
```

```
# 3 PL functions on the interval
Phi1(u)=min_symbolic(0,1/3*u-2/3)
Phi2(u)=min_symbolic(-u,0)
Phi3(u)=1/2*u-1/2
```

```
# the degree of \bar Phi
degPhi=Phi1+Phi2+Phi3+2
```

```
print "The combinatorial data"
show(B)
show(Phi1)
show(Phi2)
show(Phi3)
```

The combinatorial data

$$[-1, 3]$$

$$u \mapsto \min\left(0, \frac{1}{3}u - \frac{2}{3}\right)$$

$$u \mapsto \min(-u, 0)$$

$$u \mapsto \frac{1}{2}u - \frac{1}{2}$$

Step (i) obtain a closed form for  $F_{X,\xi}(1)$

For this we have to analytically solve the integral  $\int_{\square} u \deg \bar{\Phi}(u) e^{\xi u} du$ .

```
# The integral can be solved symbolically:
```

```
F(xi)=integral(degPhi(u)*u*exp(xi*u),u,-1,B[1])
show(F(xi))
```

$$-\frac{(4(\xi-1)e^{(3\xi)}+5\xi+10)e^{(-\xi)}}{6\xi^3} + \frac{(3\xi-2)e^{(3\xi)}+4}{2\xi^3}$$

Step (ii) find an estimate for the soliton candidate vector field  $\xi$

```
# Solve numerically
```

---

```

sol=find_root(F,-10,10)
print "Numerical solution:",sol

# Choose upper and lower bound and
# hope that the exact solution lies in between
xi_1=sol-0.0000001
xi_2=xi_1+0.0000002

#define a real value xi0 between xi_1 and xi_2
# representing the exact solution
xi0=RIF(xi_1,xi_2)

# Check whether Intermediate value theorem guarantees a zero between
# xi_1 and xi_2, i.e evaluate F at xi_1 and xi_2 using interval \
  arithmetic
if RIF(F(xi_1)) < 0 and RIF(F(xi_2)) > 0:
    print "Interval containing solution:", xi0.str(style='\
brackets')

```

Numerical solution: -1.38176017478

Interval containing solution: [-1.38176030 .. -1.38176006]

Step (iii) & (iv) obtain closed forms for  $DF_\xi(X_{y,0,1})$  and plug in the estimate for  $\xi$

For every choice of  $y \in \mathbb{P}^1$  we have to symbolically solve the integrals  $\int_{\square} e^{u\xi} \cdot ((1 + \Phi_y(u))^2 - (1 + \sum_{z \neq y} \Phi_z(u)))$ , which up to scaling with a positive constant coincide with  $DF_\xi(\mathcal{X}_{y,0,1})$ . Then we plug in the estimate for  $\xi$  into the resulting expression.

```

#check for positivity of the DF invariant for our vector field xi
print("Stability test for test configurations:")

#storage for DF values (as intervals)
IDF={}

DF1(xi)=integral(exp(xi*u)*((Phi1+1)(u)^2-(Phi3+Phi2+1)(u)^2)/2,u\
, -1,B[1])
IDF[1]=RIF(DF1(xi0)) # evaluate DF1 at xi0 using interval arithmetic
show(DF1(xi) >= IDF[1].lower())

DF2(xi)=integral(exp(xi*u)*((Phi2+1)(u)^2-(Phi1+Phi3+1)(u)^2)/2,u\
, -1,B[1])
IDF[2]=RIF(DF2(xi0))
show(DF2(xi) >= IDF[2].lower())

DF3(xi)=integral(exp(xi*u)*((Phi3+1)(u)^2-(Phi1+Phi2+1)(u)^2)/2,u\
, -1,B[1])
IDF[3]=RIF(DF3(xi0))
show(DF3(xi) >= IDF[3].lower())

```

---

```

DF4(xi)=integral(exp(xi*u)*((1)^2-(Phi3+Phi2+Phi1+1)(u)^2)/2,u,-1,B\
[1])
IDF[4]=RIF(DF4(xi0))
show(DF4(xi) >= IDF[4].lower())

```

```

if all([DF > 0 for DF in IDF.values()]):
    print("Surface is stable!")
else:
    if any([DF <= 0 for DF in IDF.values()]):
        print("Surface is not stable!")

        # print upper bound for destabilising DF value
        if IDF[1] <= 0: show(DF1(xi) <= IDF[1].upper())
        if IDF[2] <= 0: show(DF2(xi) <= IDF[2].upper())
        if IDF[3] <= 0: show(DF3(xi) <= IDF[3].upper())
        if IDF[4] <= 0: show(DF4(xi) <= IDF[4].upper())
    else:
        print("Cannot determine stability")
        # Note, that "not a > 0" does not imply "a <= 0" for \
        intervals

```

Stability test for test configurations:

$$\begin{aligned}
& -\frac{(4(3\xi-1)e^{(3\xi)}-5)e^{(-\xi)}}{36\xi^3} + \frac{(2\xi-1)e^{(3\xi)}+2\xi}{4\xi^3} \geq 0.04422930 \\
& \frac{(2(9\xi-8)e^{(3\xi)}+30\xi+25)e^{(-\xi)}}{36\xi^3} - \frac{(4\xi-3)e^{(3\xi)}+4\xi+4}{4\xi^3} \geq 0.5594457 \\
& \frac{(2(3\xi+1)e^{(3\xi)}-12(\xi+1)e^\xi-5)e^{(-\xi)}}{36\xi^3} + \frac{3(4\xi-3)e^{(3\xi)}-6(\xi-1)e^{(2\xi)}+8\xi+8}{12\xi^3} \geq 0.2463752 \\
& \frac{(2(6\xi-5)e^{(3\xi)}-12(\xi+1)e^\xi+30\xi+25)e^{(-\xi)}}{36\xi^3} + \frac{3(2\xi-1)e^{(3\xi)}-6(\xi-1)e^{(2\xi)}+2\xi-4}{12\xi^3} \geq
\end{aligned}$$

0.8500507

Surface is stable!

---

No. 26: Degree 4 / Singularity type  $A_3$ .

The combinatorial data is given by  $\square = [-1, 2]$  and  $\Phi_0(u) = \min\{-u, 0\}$ ,  $\Phi_\infty(u) = \min\{0, \frac{u-1}{2}\}$ ,  $\Phi_1(u) = \min\{0, \frac{u-1}{2}\}$

```

# We are working with interval arithmetic with precision of 26 bit
# this fixes the precision e.g. for evaluations of exponential \
  functions

```

```

RIF=RealIntervalField(26)

```

```

# The base polytope/interval
B=[-1,2]

```

```

# 3 PL functions on the interval
Phi1(u)=min_symbolic(-u,0)

```

---

```
Phi2(u)=min_symbolic((u-1)/2,0)
Phi3(u)=min_symbolic((u-1)/2,0)
```

```
# the degree of \bar Phi
degPhi=Phi1+Phi2+Phi3+2
```

```
print "The combinatorial data"
show(B)
show(Phi1)
show(Phi2)
show(Phi3)
```

The combinatorial data

$$[-1, 2]$$

$$u \mapsto \min(-u, 0)$$

$$u \mapsto \min\left(\frac{1}{2}u - \frac{1}{2}, 0\right)$$

$$u \mapsto \min\left(\frac{1}{2}u - \frac{1}{2}, 0\right)$$

Step (i) obtain a closed form for  $F_{X,\xi}(1)$

For this we have to analytically solve the integral  $\int_{\square} u \deg \bar{\Phi}(u) e^{\xi u} du$ .

```
# The integral can be solved symbolically:
```

```
F(xi)=integral(degPhi(u)*u*exp(xi*u),u,-1,B[1])
show(F(xi))
```

$$-\frac{((\xi-2)e^{(2\xi)}+\xi+2)e^{(-\xi)}}{\xi^3} + \frac{2((\xi-1)e^{(2\xi)}+1)}{\xi^3}$$

Step (ii) find an estimate for the soliton candidate vector field  $\xi$

```
# Solve numerically
```

```
sol=find_root(F,-10,10)
print "Numerical solution:",sol
```

```
# Choose upper and lower bound and
# hope that the exact solution lies in between
xi_1=sol-0.0000001
xi_2=xi_1+0.0000002
```

```
#define a real value xi0 between xi_1 and xi_2
# representing the exact solution
xi0=RIF(xi_1,xi_2)
```

```
# Check whether Intermediate value theorem guarantees a zero between
# xi_1 and xi_2, i.e evaluate F at xi_1 and xi_2 using interval \
arithmetic
if RIF(F(xi_1)) < 0 and RIF(F(xi_2)) > 0:
    print "Interval containing solution:", xi0.str(style='\
```

---

```
brackets ')
```

Numerical solution: -1.31047894021

Interval containing solution: [-1.31047905 .. -1.31047883]

Step (iii) & (iv) obtain closed forms for  $DF_\xi(X_{y,0,1})$  and plug in the estimate for  $\xi$

For every choice of  $y \in \mathbb{P}^1$  we have to symbolically solve the integrals  $\int_{\square} e^{u\xi} \cdot ((1 + \Phi_y(u))^2 - (1 + \sum_{z \neq y} \Phi_z(u)))$  which up to scaling with a positive constant coincide with  $DF_\xi(\mathcal{X}_{y,0,1})$ . Then we plug in the estimate for  $\xi$  into the resulting expression.

```
#check for positivity of the DF invariant for our vector field xi
print("Stability test for test configurations:")
```

```
#storage for DF values (as intervals)
IDF={}
```

```
DF1(xi)=integral(exp(xi*u)*((Phi1+1)(u)^2-(Phi3+Phi2+1)(u)^2)/2,u\
, -1,B[1])
```

```
IDF[1]=RIF(DF1(xi0)) # evaluate DF1 at xi0 using interval arithmetic
show(DF1(xi) >= IDF[1].lower())
```

```
DF2(xi)=integral(exp(xi*u)*((Phi2+1)(u)^2-(Phi1+Phi3+1)(u)^2)/2,u\
, -1,B[1])
```

```
IDF[2]=RIF(DF2(xi0))
show(DF2(xi) >= IDF[2].lower())
```

```
DF3(xi)=integral(exp(xi*u)*((Phi3+1)(u)^2-(Phi1+Phi2+1)(u)^2)/2,u\
, -1,B[1])
```

```
IDF[3]=RIF(DF3(xi0))
show(DF3(xi) >= IDF[3].lower())
```

```
DF4(xi)=integral(exp(xi*u)*((1)^2-(Phi3+Phi2+Phi1+1)(u)^2)/2,u,-1,B\
[1])
```

```
IDF[4]=RIF(DF4(xi0))
show(DF4(xi) >= IDF[4].lower())
```

```
if all([DF > 0 for DF in IDF.values()]):
    print("Surface is stable!")
```

```
else:
    if any([DF <= 0 for DF in IDF.values()]):
        print("Surface is not stable!")
```

```
# print upper bound for destabilising DF value
```

```
if IDF[1] <= 0: show(DF1(xi) <= IDF[1].upper())
```

```
if IDF[2] <= 0: show(DF2(xi) <= IDF[2].upper())
```

```
if IDF[3] <= 0: show(DF3(xi) <= IDF[3].upper())
```

```
if IDF[4] <= 0: show(DF4(xi) <= IDF[4].upper())
```

```
else:
```

---

```

print("Cannot determine stability")
# Note, that "not a > 0" does not imply "a <= 0" for \
intervals

```

Stability test for test configurations:

$$\frac{((\xi - 1)e^{(2\xi)} + \xi + 1)e^{(-\xi)}}{\xi^3} - \frac{(\xi - 1)e^{(2\xi)} + \xi + 1}{\xi^3} \geq 0.5757800$$

$$\frac{8(\xi - 1)e^{(2\xi)} - 3(\xi - 2)e^\xi + 6\xi + 4}{8\xi^3} - \frac{(\xi - 2)e^\xi + 2\xi + 4}{8\xi^3} \geq 0.1674627$$

$$\frac{8(\xi - 1)e^{(2\xi)} - 3(\xi - 2)e^\xi + 6\xi + 4}{8\xi^3} - \frac{(\xi - 2)e^\xi + 2\xi + 4}{8\xi^3} \geq 0.1674627$$

$$\frac{((3\xi - 2)e^{(2\xi)} - 2(\xi + 2)e^\xi + 4\xi + 4)e^{(-\xi)}}{4\xi^3} + \frac{4(\xi - 1)e^{(2\xi)} - 3(\xi - 2)e^\xi + 2\xi}{4\xi^3} \geq 0.9107058$$

Surface is stable!

---

No. 28: Degree 4 / Singularity type  $A_1A_2$ .

The combinatorial data is given by  $\square = [-1, 1]$  and  $\Phi_0(u) = \min\{0, u\}$ ,  $\Phi_\infty(u) = \min\{0, u\}$ ,  $\Phi_1(u) = \frac{-u-1}{2}$

```

# We are working with interval arithmetic with precision of 26 bit
# this fixes the precision e.g. for evaluations of exponential \
functions

```

```
RIF=RealIntervalField(26)
```

```

# The base polytope/interval
B=[-1,1]

```

```
# 3 PL functions on the interval
```

```
Phi1(u)=min_symbolic(0,u)
```

```
Phi2(u)=min_symbolic(0,u)
```

```
Phi3(u)=-1/2*u-1/2
```

```
# the degree of \bar Phi
```

```
degPhi=Phi1+Phi2+Phi3+2
```

```
print "The combinatorial data"
```

```
show(B)
```

```
show(Phi1)
```

```
show(Phi2)
```

```
show(Phi3)
```

The combinatorial data

$[-1, 1]$

$u \mapsto \min(0, u)$

$u \mapsto \min(0, u)$

$u \mapsto -\frac{1}{2}u - \frac{1}{2}$

Step (i) obtain a closed form for  $F_{X,\xi}(1)$

For this we have to analytically solve the integral  $\int_{\square} u \deg \bar{\Phi}(u) e^{\xi u} du$ .

```
# The integral can be solved symbolically:
F(xi)=integral(degPhi(u)*u*exp(xi*u),u,-1,B[1])
show(F(xi))
```

$$-\frac{(3\xi - 8e^{\xi} + 6)e^{(-\xi)}}{2\xi^3} + \frac{(2\xi^2 - \xi - 2)e^{\xi}}{2\xi^3}$$

Step (ii) find an estimate for the soliton candidate vector field  $\xi$

```
# Solve numerically
sol=find_root(F,-10,10)
print "Numerical solution:",sol

# Choose upper and lower bound and
# hope that the exact solution lies in between
xi_1=sol-0.0000001
xi_2=xi_1+0.0000002

#define a real value xi0 between xi_1 and xi_2
# representing the exact solution
xi0=RIF(xi_1,xi_2)

# Check whether Intermediate value theorem guarantees a zero between
# xi_1 and xi_2, i.e evaluate F at xi_1 and xi_2 using interval \
arithmetic
if RIF(F(xi_1)) < 0 and RIF(F(xi_2)) > 0:
    print "Interval containing solution:", xi0.str(style='\
brackets')
```

Numerical solution: -0.743738705959

Interval containing solution: [-0.743738816 .. -0.743738591]

Step (iii) & (iv) obtain closed forms for  $DF_{\xi}(X_{y,0,1})$  and plug in the estimate for  $\xi$

For every choice of  $y \in \mathbb{P}^1$  we have to symbolically solve the integrals  $\int_{\square} e^{u\xi} \cdot ((1 + \Phi_y(u))^2 - (1 + \sum_{z \neq y} \Phi_z(u)))$  which up to scaling with a positive constant coincide with  $DF_{\xi}(\mathcal{X}_{y,0,1})$ . Then we plug in the estimate for  $\xi$  into the resulting expression.

```
#check for positivity of the DF invariant for our vector field xi
print("Stability test for test configurations:")

#storage for DF values (as intervals)
IDF={}

DF1(xi)=integral(exp(xi*u)*((Phi1+1)(u)^2-(Phi3+Phi2+1)(u)^2)/2,u\
,-1,B[1])
IDF[1]=RIF(DF1(xi0)) # evaluate DF1 at xi0 using interval arithmetic
show(DF1(xi) >= IDF[1].lower())
```



---

```

DF2(xi)=integral(exp(xi*u)*((Phi2+1)(u)^2-(Phi1+Phi3+1)(u)^2)/2,u\
    ,-1,B[1])
IDF[2]=RIF(DF2(xi0))
show(DF2(xi) >= IDF[2].lower())

DF3(xi)=integral(exp(xi*u)*((Phi3+1)(u)^2-(Phi1+Phi2+1)(u)^2)/2,u\
    ,-1,B[1])
IDF[3]=RIF(DF3(xi0))
show(DF3(xi) >= IDF[3].lower())

DF4(xi)=integral(exp(xi*u)*((1)^2-(Phi3+Phi2+Phi1+1)(u)^2)/2,u,-1,B\
    [1])
IDF[4]=RIF(DF4(xi0))
show(DF4(xi) >= IDF[4].lower())

if all([DF > 0 for DF in IDF.values()]):
    print("Surface is stable!")
else:
    if any([DF <= 0 for DF in IDF.values()]):
        print("Surface is not stable!")

    # print upper bound for destabilising DF value
    if IDF[1] <= 0: show(DF1(xi) <= IDF[1].upper())
    if IDF[2] <= 0: show(DF2(xi) <= IDF[2].upper())
    if IDF[3] <= 0: show(DF3(xi) <= IDF[3].upper())
    if IDF[4] <= 0: show(DF4(xi) <= IDF[4].upper())
    else:
        print("Cannot determine stability")
        # Note, that "not a > 0" does not imply "a <= 0" for \
        intervals

```

Stability test for test configurations:

$$\begin{aligned}
& -\frac{(2(\xi-2)e^\xi+3)e^{(-\xi)}}{4\xi^3} + \frac{(2\xi^2-1)e^\xi}{4\xi^3} \geq 0.4699562 \\
& -\frac{(2(\xi-2)e^\xi+3)e^{(-\xi)}}{4\xi^3} + \frac{(2\xi^2-1)e^\xi}{4\xi^3} \geq 0.4699562 \\
& \frac{(8(\xi-2)e^\xi+6\xi+15)e^{(-\xi)}}{4\xi^3} - \frac{(2\xi^2-1)e^\xi}{4\xi^3} \geq (-0.1023106) \\
& \frac{(4(\xi-2)e^\xi+6\xi+9)e^{(-\xi)}}{4\xi^3} + \frac{(2\xi^2-1)e^\xi}{4\xi^3} \geq 0.8376046
\end{aligned}$$

Surface is not stable!

$$\frac{(8(\xi-2)e^\xi+6\xi+15)e^{(-\xi)}}{4\xi^3} - \frac{(2\xi^2-1)e^\xi}{4\xi^3} \leq (-0.1023037)$$

---

No. 29: Degree 5 / Singularity type  $A_4$ .

The combinatorial data is given by  $\square = [-1, 5]$  and  $\Phi_0(u) = \min\{-u, 0\}$ ,  $\Phi_\infty(u) = \frac{u-2}{3}$ ,  $\Phi_1(u) = \frac{u-1}{2}$

---

```
# We are working with interval arithmetic with precision of 26 bit
# this fixes the precision e.g. for evaluations of exponential \
    functions
```

```
RIF=RealIntervalField(26)
```

```
# The base polytope/interval
B=[-1,1]
```

```
# 3 PL functions on the interval
```

```
Phi1(u)=min_symbolic(0,-u)
```

```
Phi2(u)=1/3*u-2/3
```

```
Phi3(u)=1/2*u-1/2
```

```
# the degree of \bar Phi
```

```
degPhi=Phi1+Phi2+Phi3+2
```

```
print "The combinatorial data"
```

```
show(B)
```

```
show(Phi1)
```

```
show(Phi2)
```

```
show(Phi3)
```

The combinatorial data

$[-1, 1]$

$u \mapsto \min(0, -u)$

$u \mapsto \frac{1}{3}u - \frac{2}{3}$

$u \mapsto \frac{1}{2}u - \frac{1}{2}$

Step (i) obtain a closed form for  $F_{X,\xi}(1)$

For this we have to analytically solve the integral  $\int_{\square} u \deg \bar{\Phi}(u) e^{\xi u} du$ .

```
# The integral can be solved symbolically:
```

```
F(xi)=integral(degPhi(u)*u*exp(xi*u),u,-1,B[1])
```

```
show(F(xi))
```

$$-\frac{5(\xi+2)e^{(-\xi)}}{6\xi^3} + \frac{(4\xi^2-3\xi-2)e^{\xi}+12}{6\xi^3}$$

Step (ii) find an estimate for the soliton candidate vector field  $\xi$

```
# Solve numerically
```

```
sol=find_root(F,-10,10)
```

```
print "Numerical solution:",sol
```

```
# Choose upper and lower bound and
```

```
# hope that the exact solution lies in between
```

```
xi_1=sol-0.0000001
```

```
xi_2=xi_1+0.0000002
```

---

```

#define a real value xi0 between xi_1 and xi_2
# representing the exact solution
xi0=RIF(xi_1,xi_2)

# Check whether Intermediate value theorem guarantees a zero between
# xi_1 and xi_2, i.e evaluate F at xi_1 and xi_2 using interval \
  arithmetic
if RIF(F(xi_1)) < 0 and RIF(F(xi_2)) > 0:
    print "Interval containing solution:", xi0.str(style='\
brackets')

```

Numerical solution: -0.830799974476

Interval containing solution: [-0.830800087 .. -0.830799862]

Step (iii) & (iv) obtain closed forms for  $DF_\xi(X_{y,0,1})$  and plug in the estimate for  $\xi$

For every choice of  $y \in \mathbb{P}^1$  we have to symbolically solve the integrals  $\int_{\square} e^{u\xi} \cdot \left( (1 + \Phi_y(u))^2 - (1 + \sum_{z \neq y} \Phi_z(u)) \right)$  which up to scaling with a positive constant coincide with  $DF_\xi(\mathcal{X}_{y,0,1})$ . Then we plug in the estimate for  $\xi$  into the resulting expression.

```

#check for positivity of the DF invariant for our vector field xi
print("Stability test for test configurations:")

#storage for DF values (as intervals)
IDF={}

DF1(xi)=integral(exp(xi*u)*((Phi1+1)(u)^2-(Phi3+Phi2+1)(u)^2)/2,u\
, -1,B[1])
IDF[1]=RIF(DF1(xi0)) # evaluate DF1 at xi0 using interval arithmetic
show(DF1(xi) >= IDF[1].lower())

DF2(xi)=integral(exp(xi*u)*((Phi2+1)(u)^2-(Phi1+Phi3+1)(u)^2)/2,u\
, -1,B[1])
IDF[2]=RIF(DF2(xi0))
show(DF2(xi) >= IDF[2].lower())

DF3(xi)=integral(exp(xi*u)*((Phi3+1)(u)^2-(Phi1+Phi2+1)(u)^2)/2,u\
, -1,B[1])
IDF[3]=RIF(DF3(xi0))
show(DF3(xi) >= IDF[3].lower())

DF4(xi)=integral(exp(xi*u)*((1)^2-(Phi3+Phi2+Phi1+1)(u)^2)/2,u, -1,B\
[1])
IDF[4]=RIF(DF4(xi0))
show(DF4(xi) >= IDF[4].lower())

if all([DF > 0 for DF in IDF.values()]):
    print("Surface is stable!")

```

---

```

else:
    if any([DF <= 0 for DF in IDF.values()]):
        print("Surface is not stable!")

        # print upper bound for destabilising DF value
        if IDF[1] <= 0: show(DF1(xi) <= IDF[1].upper())
        if IDF[2] <= 0: show(DF2(xi) <= IDF[2].upper())
        if IDF[3] <= 0: show(DF3(xi) <= IDF[3].upper())
        if IDF[4] <= 0: show(DF4(xi) <= IDF[4].upper())
    else:
        print("Cannot determine stability")
        # Note, that "not a > 0" does not imply "a <= 0" for \
        intervals

```

Stability test for test configurations:

$$\frac{5(6\xi + 5)e^{(-\xi)}}{36\xi^3} - \frac{(8\xi^2 - 20\xi - 11)e^\xi + 36\xi + 36}{36\xi^3} \geq 0.5216795$$

$$\frac{(8\xi^2 - 8\xi - 5)e^\xi + 18\xi}{36\xi^3} + \frac{5e^{(-\xi)}}{36\xi^3} \geq 0.01721630$$

$$\frac{(16\xi^2 - 10\xi - 7)e^\xi + 12\xi + 12}{36\xi^3} - \frac{5e^{(-\xi)}}{36\xi^3} \geq 0.1968489$$

$$\frac{5(6\xi + 5)e^{(-\xi)}}{36\xi^3} + \frac{(16\xi^2 + 2\xi - 1)e^\xi - 6\xi - 24}{36\xi^3} \geq 0.7357463$$

Surface is stable!

---

No. 30: Degree 5 / Singularity type  $A_3$ .

The combinatorial data is given by  $\square = [-1, 3]$  and  $\Phi_0(u) = \min\{\frac{u-1}{2}, 0\}$ ,  $\Phi_\infty(u) = \min\{0, u\}$ ,  $\Phi_1(u) = \frac{-u-1}{2}$

```

# We are working with interval arithmetic with precision of 26 bit
# this fixes the precision e.g. for evaluations of exponential \
  functions
RIF=RealIntervalField(26)

```

```

# The base polytope/interval
B=[-1,3]

```

```

# 3 PL functions on the interval
Phi1(u)=min_symbolic(0,1/2*u-1/2)
Phi2(u)=min_symbolic(-u,0)
Phi3(u)=1/2*u-1/2

```

```

# the degree of \bar Phi
degPhi=Phi1+Phi2+Phi3+2

```

```

print "The combinatorial data"
show(B)

```

---

```
show(Phi1)
show(Phi2)
show(Phi3)
```

The combinatorial data

$$[-1, 3]$$

$$u \mapsto \min\left(0, \frac{1}{2}u - \frac{1}{2}\right)$$

$$u \mapsto \min(-u, 0)$$

$$u \mapsto \frac{1}{2}u - \frac{1}{2}$$

Step (i) obtain a closed form for  $F_{X,\xi}(1)$

For this we have to analytically solve the integral  $\int_{\square} u \deg \bar{\Phi}(u) e^{\xi u} du$ .

# The integral can be solved symbolically:

```
F(xi)=integral(degPhi(u)*u*exp(xi*u),u,-1,B[1])
show(F(xi))
```

$$-\frac{((\xi-2)e^{(2\xi)}+2\xi+4)e^{(-\xi)}}{2\xi^3} + \frac{(3\xi-2)e^{(3\xi)}+4}{2\xi^3}$$

Step (ii) find an estimate for the soliton candidate vector field  $\xi$

# Solve numerically

```
sol=find_root(F,-10,10)
print "Numerical solution:",sol
```

# Choose upper and lower bound and

# hope that the exact solution lies in between

```
xi_1=sol-0.0000001
xi_2=xi_1+0.0000002
```

#define a real value xi0 between xi\_1 and xi\_2

# representing the exact solution

```
xi0=RIF(xi_1,xi_2)
```

# Check whether Intermediate value theorem guarantees a zero between

# xi\_1 and xi\_2, i.e evaluate F at xi\_1 and xi\_2 using interval \ arithmetic

```
if RIF(F(xi_1)) < 0 and RIF(F(xi_2)) > 0:
    print "Interval containing solution:", xi0.str(style='\
brackets')
```

Numerical solution: -1.4388637356

Interval containing solution: [-1.43886385 .. -1.43886363]

Step (iii) & (iv) obtain closed forms for  $DF_{\xi}(X_{y,0,1})$  and plug in the estimate for  $\xi$

For every choice of  $y \in \mathbb{P}^1$  we have to symbolically solve the integrals  $\int_{\square} e^{u\xi} \cdot ((1 + \Phi_y(u))^2 - (1 + \sum_{z \neq y} \Phi_z(u)))$  which up to scaling with a positive constant coincide with  $DF_{\xi}(\mathcal{X}_{y,0,1})$ . Then we plug in the estimate for  $\xi$  into the resulting expression.

---

```

#check for positivity of the DF invariant for our vector field xi
print("Stability test for test configurations:")

#storage for DF values (as intervals)
IDF={}

DF1(xi)=integral(exp(xi*u)*((Phi1+1)(u)^2-(Phi3+Phi2+1)(u)^2)/2,u\
, -1 ,B[1])
IDF[1]=RIF(DF1(xi0)) # evaluate DF1 at xi0 using interval arithmetic
show(DF1(xi) >= IDF[1].lower())

DF2(xi)=integral(exp(xi*u)*((Phi2+1)(u)^2-(Phi1+Phi3+1)(u)^2)/2,u\
, -1 ,B[1])
IDF[2]=RIF(DF2(xi0))
show(DF2(xi) >= IDF[2].lower())

DF3(xi)=integral(exp(xi*u)*((Phi3+1)(u)^2-(Phi1+Phi2+1)(u)^2)/2,u\
, -1 ,B[1])
IDF[3]=RIF(DF3(xi0))
show(DF3(xi) >= IDF[3].lower())

DF4(xi)=integral(exp(xi*u)*((1)^2-(Phi3+Phi2+Phi1+1)(u)^2)/2,u, -1 ,B\
[1])
IDF[4]=RIF(DF4(xi0))
show(DF4(xi) >= IDF[4].lower())

if all([DF > 0 for DF in IDF.values()]):
    print("Surface is stable!")
else:
    if any([DF <= 0 for DF in IDF.values()]):
        print("Surface is not stable!")

    # print upper bound for destabilising DF value
    if IDF[1] <= 0: show(DF1(xi) <= IDF[1].upper())
    if IDF[2] <= 0: show(DF2(xi) <= IDF[2].upper())
    if IDF[3] <= 0: show(DF3(xi) <= IDF[3].upper())
    if IDF[4] <= 0: show(DF4(xi) <= IDF[4].upper())
    else:
        print("Cannot determine stability")
        # Note, that "not a > 0" does not imply "a <= 0" for \
intervals

```

Stability test for test configurations:

$$\begin{aligned}
& -\frac{(2\xi-1)e^\xi}{4\xi^3} + \frac{(2\xi-1)e^{(3\xi)} + 2\xi}{4\xi^3} \geq 0.1686591 \\
& \frac{((2\xi-3)e^{(2\xi)} + 4\xi + 4)e^{(-\xi)}}{4\xi^3} - \frac{(4\xi-3)e^{(3\xi)} + 4\xi + 4}{4\xi^3} \geq 0.5809738
\end{aligned}$$

---


$$\frac{2(4\xi - 3)e^{(3\xi)} - 3(\xi - 2)e^\xi + 6\xi + 4}{8\xi^3} + \frac{3\xi e^\xi - 2\xi - 4}{8\xi^3} \geq 0.1915944$$

$$\frac{((3\xi - 4)e^{(2\xi)} - 2(\xi + 2)e^\xi + 8\xi + 8)e^{(-\xi)}}{8\xi^3} + \frac{2(2\xi - 1)e^{(3\xi)} - 3(\xi - 2)e^\xi + 2\xi - 4}{8\xi^3} \geq 0.9412277$$

Surface is stable!

---

No. 31: Degree 5 / Singularity type  $A_2$ .

The combinatorial data is given by  $\square = [-1, 2]$  and  $\Phi_0(u) = \min\{0, u\}$ ,  $\Phi_\infty(u) = \min\{0, u\}$ ,  $\Phi_1(u) = \min\{0, \frac{-u-1}{2}\}$

```
# We are working with interval arithmetic with precision of 26 bit
# this fixes the precision e.g. for evaluations of exponential \
  functions
```

```
RIF=RealIntervalField(26)
```

```
# The base polytope/interval
B=[-1,3]
```

```
# 3 PL functions on the interval
Phi1(u)=min_symbolic(0,u)
Phi2(u)=min_symbolic(0,-u)
Phi3(u)=min_symbolic(0,1/2*u-1/2)
```

```
# the degree of \bar Phi
degPhi=Phi1+Phi2+Phi3+2
```

```
print "The combinatorial data"
show(B)
show(Phi1)
show(Phi2)
show(Phi3)
```

The combinatorial data

$$[-1, 3]$$

$$u \mapsto \min(0, u)$$

$$u \mapsto \min(0, -u)$$

$$u \mapsto \min\left(0, \frac{1}{2}u - \frac{1}{2}\right)$$

Step (i) obtain a closed form for  $F_{X,\xi}(1)$

For this we have to analytically solve the integral  $\int_{\square} u \deg \bar{\Phi}(u) e^{\xi u} du$ .

```
# The integral can be solved symbolically:
```

```
F(xi)=integral(degPhi(u)*u*exp(xi*u),u,-1,B[1])
show(F(xi))
```

$$-\frac{((\xi - 2)e^{(2\xi)} + 3\xi - 4e^\xi + 6)e^{(-\xi)}}{2\xi^3} - \frac{(3\xi^2 - 4\xi + 2)e^{(3\xi)} - 2}{\xi^3}$$

---

Step (ii) find an estimate for the soliton candidate vector field  $\xi$

```
# Solve numerically
sol=find_root(F,-10,10)
print "Numerical solution:",sol

# Choose upper and lower bound and
# hope that the exact solution lies in between
xi_1=sol-0.000001
xi_2=xi_1+0.000002

#define a real value xi0 between xi_1 and xi_2
# representing the exact solution
xi0=RIF(xi_1,xi_2)

# Check whether Intermediate value theorem guarantees a zero between
# xi_1 and xi_2, i.e evaluate F at xi_1 and xi_2 using interval \
  arithmetic
if RIF(F(xi_1)) > 0 and RIF(F(xi_2)) < 0:
    print "Interval containing solution:", xi0.str(style='\
brackets')

Numerical solution: -0.242677720874
Interval containing solution: [-0.242678725 .. -0.242676720]
```

Step (iii) & (iv) obtain closed forms for  $DF_\xi(X_{y,0,1})$  and plug in the estimate for  $\xi$

For every choice of  $y \in \mathbb{P}^1$  we have to symbolically solve the integrals  $\int_{\square} e^{u\xi} \cdot ((1 + \Phi_y(u))^2 - (1 + \sum_{z \neq y} \Phi_z(u)))$  which up to scaling with a positive constant coincide with  $DF_\xi(\mathcal{X}_{y,0,1})$ . Then we plug in the estimate for  $\xi$  into the resulting expression.

```
#check for positivity of the DF invariant for our vector field xi
print("Stability test for test configurations:")

#storage for DF values (as intervals)
IDF={}

DF1(xi)=integral(exp(xi*u)*((Phi1+1)(u)^2-(Phi3+Phi2+1)(u)^2)/2,u\
,-1,B[1])
IDF[1]=RIF(DF1(xi0)) # evaluate DF1 at xi0 using interval arithmetic
show(DF1(xi) >= IDF[1].lower())

DF2(xi)=integral(exp(xi*u)*((Phi2+1)(u)^2-(Phi1+Phi3+1)(u)^2)/2,u\
,-1,B[1])
IDF[2]=RIF(DF2(xi0))
show(DF2(xi) >= IDF[2].lower())

DF3(xi)=integral(exp(xi*u)*((Phi3+1)(u)^2-(Phi1+Phi2+1)(u)^2)/2,u\
,-1,B[1])
```



---

```

IDF[3]=RIF(DF3(xi0))
show(DF3(xi) >= IDF[3].lower())

DF4(xi)=integral(exp(xi*u)*((1)^2-(Phi3+Phi2+Phi1+1)(u)^2)/2,u,-1,B\
[1])
IDF[4]=RIF(DF4(xi0))
show(DF4(xi) >= IDF[4].lower())

if all([DF > 0 for DF in IDF.values()]):
    print("Surface is stable!")
else:
    if any([DF <= 0 for DF in IDF.values()]):
        print("Surface is not stable!")

    # print upper bound for destabilising DF value
    if IDF[1] <= 0: show(DF1(xi) <= IDF[1].upper())
    if IDF[2] <= 0: show(DF2(xi) <= IDF[2].upper())
    if IDF[3] <= 0: show(DF3(xi) <= IDF[3].upper())
    if IDF[4] <= 0: show(DF4(xi) <= IDF[4].upper())
    else:
        print("Cannot determine stability")
        # Note, that "not a > 0" does not imply "a <= 0" for \
intervals

```

Stability test for test configurations:

$$\begin{aligned}
& \frac{(3\xi e^{(2\xi)} - 2(5\xi - 2)e^\xi - 6)e^{(-\xi)}}{8\xi^3} - \frac{4(3\xi^2 - 4\xi + 2)e^{(3\xi)} + 3(\xi - 2)e^\xi - 6\xi - 4}{8\xi^3} \geq 0.4280779 \\
& \frac{((5\xi - 4)e^{(2\xi)} + 6(\xi - 2)e^\xi + 12\xi + 18)e^{(-\xi)}}{8\xi^3} + \frac{4(3\xi^2 - 4\xi + 2)e^{(3\xi)} - (\xi - 2)e^\xi - 10\xi - 12}{8\xi^3} \geq \\
& 0.4278612 \\
& - \frac{((2\xi - 1)e^{(2\xi)} - 4(\xi - 1)e^\xi - 3)e^{(-\xi)}}{4\xi^3} - \frac{(3\xi^2 - 4\xi + 2)e^{(3\xi)} - 2\xi - 2}{2\xi^3} \geq (-0.1469232) \\
& \frac{((2\xi - 1)e^{(2\xi)} + 2(\xi - 4)e^\xi + 6\xi + 9)e^{(-\xi)}}{4\xi^3} - \frac{(3\xi^2 - 4\xi + 2)e^{(3\xi)} + (\xi - 2)e^\xi - \xi}{2\xi^3} \geq 0.7109140 \\
& \text{Surface is not stable!} \\
& - \frac{((2\xi - 1)e^{(2\xi)} - 4(\xi - 1)e^\xi - 3)e^{(-\xi)}}{4\xi^3} - \frac{(3\xi^2 - 4\xi + 2)e^{(3\xi)} - 2\xi - 2}{2\xi^3} \leq (-0.1458051)
\end{aligned}$$


---

No. 32: Degree 5 / Singularity type  $A_1$ .

The combinatorial data is given by  $\square = [-1, 1]$  and  $\Phi_0(u) = \min\{0, u\}$ ,  $\Phi_\infty(u) = \min\{0, u\}$ ,  $\Phi_1(u) = \min\{-u, 0\}$

```

# We are working with interval arithmetic with precision of 26 bit
# this fixes the precision e.g. for evaluations of exponential \
functions
RIF=RealIntervalField(26)

```

---

```

# The base polytope/interval
B=[-1,3]

# 3 PL functions on the interval
Phi1(u)=min_symbolic(0,u)
Phi2(u)=min_symbolic(0,u)
Phi3(u)=min_symbolic(-u,0)

# the degree of \bar Phi
degPhi=Phi1+Phi2+Phi3+2

print "The combinatorial data"
show(B)
show(Phi1)
show(Phi2)
show(Phi3)

```

The combinatorial data

```

[-1, 3]
u ↦ min(0, u)
u ↦ min(0, u)
u ↦ min(-u, 0)

```

Step (i) obtain a closed form for  $F_{X,\xi}(1)$

For this we have to analytically solve the integral  $\int_{\square} u \deg \bar{\Phi}(u) e^{\xi u} du$ .

```

# The integral can be solved symbolically:
F(xi)=integral(degPhi(u)*u*exp(xi*u),u,-1,B[1])
show(F(xi))

```

$$-\frac{2(\xi - 2e^{\xi} + 2)e^{(-\xi)}}{\xi^3} - \frac{(3\xi^2 - 4\xi + 2)e^{(3\xi)} - 2}{\xi^3}$$

Step (ii) find an estimate for the soliton candidate vector field  $\xi$

```

# Solve numerically
sol=find_root(F,-10,10)
print "Numerical solution:",sol

# Choose upper and lower bound and
# hope that the exact solution lies in between
xi_2=sol-0.0000001
xi_1=xi_2+0.0000002

#define a real value xi0 between xi_1 and xi_2
# representing the exact solution
xi0=RIF(xi_1,xi_2)

# Check whether Intermediate value theorem guarantees a zero between
# xi_1 and xi_2, i.e evaluate F at xi_1 and xi_2 using interval \

```

---

```

    arithmetic
if RIF(F(xi_1)) < 0 and RIF(F(xi_2)) > 0:
    print "Interval containing solution:", xi0.str(style='\
brackets')

```

Numerical solution: -0.276432541617

Interval containing solution: [-0.276432649 .. -0.276432439]

Step (iii) & (iv) obtain closed forms for  $DF_\xi(X_{y,0,1})$  and plug in the estimate for  $\xi$

For every choice of  $y \in \mathbb{P}^1$  we have to symbolically solve the integrals  $\int_{\square} e^{u\xi} \cdot ((1 + \Phi_y(u))^2 - (1 + \sum_{z \neq y} \Phi_z(u)))$  which up to scaling with a positive constant coincide with  $DF_\xi(\mathcal{X}_{y,0,1})$ . Then we plug in the estimate for  $\xi$  into the resulting expression.

```

#check for positivity of the DF invariant for our vector field xi
print("Stability test for test configurations:")

#storage for DF values (as intervals)
IDF={}

DF1(xi)=integral(exp(xi*u)*((Phi1+1)(u)^2-(Phi3+Phi2+1)(u)^2)/2,u\
, -1,B[1])
IDF[1]=RIF(DF1(xi0)) # evaluate DF1 at xi0 using interval arithmetic
show(DF1(xi) >= IDF[1].lower())

DF2(xi)=integral(exp(xi*u)*((Phi2+1)(u)^2-(Phi1+Phi3+1)(u)^2)/2,u\
, -1,B[1])
IDF[2]=RIF(DF2(xi0))
show(DF2(xi) >= IDF[2].lower())

DF3(xi)=integral(exp(xi*u)*((Phi3+1)(u)^2-(Phi1+Phi2+1)(u)^2)/2,u\
, -1,B[1])
IDF[3]=RIF(DF3(xi0))
show(DF3(xi) >= IDF[3].lower())

DF4(xi)=integral(exp(xi*u)*((1)^2-(Phi3+Phi2+Phi1+1)(u)^2)/2,u, -1,B\
[1])
IDF[4]=RIF(DF4(xi0))
show(DF4(xi) >= IDF[4].lower())

if all([DF > 0 for DF in IDF.values()]):
    print("Surface is stable!")
else:
    if any([DF <= 0 for DF in IDF.values()]):
        print("Surface is not stable!")

# print upper bound for destabilising DF value
if IDF[1] <= 0: show(DF1(xi) <= IDF[1].upper())
if IDF[2] <= 0: show(DF2(xi) <= IDF[2].upper())

```

---

```

    if IDF[3] <= 0: show(DF3(xi) <= IDF[3].upper())
    if IDF[4] <= 0: show(DF4(xi) <= IDF[4].upper())
else:
    print("Cannot determine stability")
    # Note, that "not a > 0" does not imply "a <= 0" for \
intervals

```

Stability test for test configurations:

$$\begin{aligned}
& -\frac{(3\xi^2 - 4\xi + 2)e^{(3\xi)} - 2\xi - 2}{2\xi^3} \geq 0.1917138 \\
& -\frac{(3\xi^2 - 4\xi + 2)e^{(3\xi)} - 2\xi - 2}{2\xi^3} \geq 0.1917138 \\
& \frac{2((\xi - 2)e^\xi + \xi + 2)e^{(-\xi)}}{\xi^3} + \frac{(3\xi^2 - 4\xi + 2)e^{(3\xi)} - 2\xi - 2}{2\xi^3} \geq 0.1916600 \\
& \frac{2((\xi - 2)e^\xi + \xi + 2)e^{(-\xi)}}{\xi^3} - \frac{(3\xi^2 - 4\xi + 2)e^{(3\xi)} - 2\xi - 2}{2\xi^3} \geq 0.5751334
\end{aligned}$$

Surface is stable!

---

No. 33: Degree 6 / Singularity type  $A_2$ .

The combinatorial data is given by  $\square = [-1, 3]$  and  $\Phi_0(u) = \min\{0, u\}$ ,  $\Phi_\infty(u) = \min\{0, u\}$ ,  $\Phi_1(u) = \frac{-u-1}{2}$

```

# We are working with interval arithmetic with precision of 26 bit
# this fixes the precision e.g. for evaluations of exponential \
functions

```

```
RIF=RealIntervalField(26)
```

```

# The base polytope/interval
B=[-1,3]

```

```
# 3 PL functions on the interval
```

```
Phi1(u)=min_symbolic(0,u)
```

```
Phi2(u)=min_symbolic(0,u)
```

```
Phi3(u)=-1/2*u-1/2
```

```
# the degree of \bar Phi
```

```
degPhi=Phi1+Phi2+Phi3+2
```

```
print "The combinatorial data"
```

```
show(B)
```

```
show(Phi1)
```

```
show(Phi2)
```

```
show(Phi3)
```

The combinatorial data

$[-1, 3]$

$u \mapsto \min(0, u)$

$$u \mapsto \min(0, u)$$

$$u \mapsto -\frac{1}{2}u - \frac{1}{2}$$

Step (i) obtain a closed form for  $F_{X,\xi}(1)$

For this we have to analytically solve the integral  $\int_{\square} u \deg \bar{\Phi}(u) e^{\xi u} du$ .

```
# The integral can be solved symbolically:
F(xi)=integral(degPhi(u)*u*exp(xi*u),u,-1,B[1])
show(F(xi))
```

$$\frac{(3\xi - 2)e^{(3\xi)}}{2\xi^3} - \frac{(3\xi - 8e^{\xi} + 6)e^{(-\xi)}}{2\xi^3}$$

Step (ii) find an estimate for the soliton candidate vector field  $\xi$

```
# Solve numerically
sol=find_root(F,-10,10)
print "Numerical solution:",sol

# Choose upper and lower bound and
# hope that the exact solution lies in between
xi_1=sol-0.0000001
xi_2=xi_1+0.0000002

#define a real value xi0 between xi_1 and xi_2
# representing the exact solution
xi0=RIF(xi_1,xi_2)

# Check whether Intermediate value theorem guarantees a zero between
# xi_1 and xi_2, i.e evaluate F at xi_1 and xi_2 using interval \
  arithmetic
if RIF(F(xi_1)) < 0 and RIF(F(xi_2)) > 0:
    print "Interval containing solution:", xi0.str(style='\
brackets')
```

Numerical solution: -1.24607304295

Interval containing solution: [-1.24607316 .. -1.24607291]

Step (iii) & (iv) obtain closed forms for  $DF_{\xi}(X_{y,0,1})$  and plug in the estimate for  $\xi$

For every choice of  $y \in \mathbb{P}^1$  we have to symbolically solve the integrals  $\int_{\square} e^{u\xi} \cdot ((1 + \Phi_y(u))^2 - (1 + \sum_{z \neq y} \Phi_z(u)))$ , which up to scaling with a positive constant coincide with  $DF_{\xi}(\mathcal{X}_{y,0,1})$ . Then we plug in the estimate for  $\xi$  into the resulting expression.

```
#check for positivity of the DF invariant for our vector field xi
print("Stability test for test configurations:")

#storage for DF values (as intervals)
IDF={}
```

---

```

DF1(xi)=integral(exp(xi*u)*((Phi1+1)(u)^2-(Phi3+Phi2+1)(u)^2)/2,u\
, -1,B[1])
IDF[1]=RIF(DF1(xi0)) # evaluate DF1 at xi0 using interval arithmetic
show(DF1(xi) >= IDF[1].lower())

DF2(xi)=integral(exp(xi*u)*((Phi2+1)(u)^2-(Phi1+Phi3+1)(u)^2)/2,u\
, -1,B[1])
IDF[2]=RIF(DF2(xi0))
show(DF2(xi) >= IDF[2].lower())

DF3(xi)=integral(exp(xi*u)*((Phi3+1)(u)^2-(Phi1+Phi2+1)(u)^2)/2,u\
, -1,B[1])
IDF[3]=RIF(DF3(xi0))
show(DF3(xi) >= IDF[3].lower())

DF4(xi)=integral(exp(xi*u)*((1)^2-(Phi3+Phi2+Phi1+1)(u)^2)/2,u,-1,B\
[1])
IDF[4]=RIF(DF4(xi0))
show(DF4(xi) >= IDF[4].lower())

if all([DF > 0 for DF in IDF.values()]):
    print("Surface is stable!")
else:
    if any([DF <= 0 for DF in IDF.values()]):
        print("Surface is not stable!")

        # print upper bound for destabilising DF value
        if IDF[1] <= 0: show(DF1(xi) <= IDF[1].upper())
        if IDF[2] <= 0: show(DF2(xi) <= IDF[2].upper())
        if IDF[3] <= 0: show(DF3(xi) <= IDF[3].upper())
        if IDF[4] <= 0: show(DF4(xi) <= IDF[4].upper())
    else:
        print("Cannot determine stability")
        # Note, that "not a > 0" does not imply "a <= 0" for \
intervals

```

Stability test for test configurations:

$$\begin{aligned}
& \frac{(2\xi-1)e^{(3\xi)}}{4\xi^3} - \frac{(2(\xi-2)e^\xi+3)e^{(-\xi)}}{4\xi^3} \geq 0.5195618 \\
& \frac{(2\xi-1)e^{(3\xi)}}{4\xi^3} - \frac{(2(\xi-2)e^\xi+3)e^{(-\xi)}}{4\xi^3} \geq 0.5195618 \\
& -\frac{(2\xi-1)e^{(3\xi)}}{4\xi^3} + \frac{(8(\xi-2)e^\xi+6\xi+15)e^{(-\xi)}}{4\xi^3} \geq (-0.03507074) \\
& \frac{(2\xi-1)e^{(3\xi)}}{4\xi^3} + \frac{(4(\xi-2)e^\xi+6\xi+9)e^{(-\xi)}}{4\xi^3} \geq 1.004053
\end{aligned}$$

Surface is not stable!

$$-\frac{(2\xi-1)e^{(3\xi)}}{4\xi^3} + \frac{(8(\xi-2)e^\xi+6\xi+15)e^{(-\xi)}}{4\xi^3} \leq (-0.03506876)$$

---

No. 34: Degree 6 / Singularity type  $A_1$ .

The combinatorial data is given by  $\square = [-1, 2]$  and  $\Phi_0(u) = \min\{-u, 0\}$ ,  $\Phi_\infty(u) = \min\{0, u\}$ ,  $\Phi_1(u) = \min\{0, u\}$

```
# We are working with interval arithmetic with precision of 26 bit
# this fixes the precision e.g. for evaluations of exponential \
  functions
```

```
RIF=RealIntervalField(26)
```

```
# The base polytope/interval
```

```
B=[-1,2]
```

```
# 3 PL functions on the interval
```

```
Phi1(u)=min_symbolic(-u,0)
```

```
Phi2(u)=min_symbolic(0,u)
```

```
Phi3(u)=min_symbolic(0,u)
```

```
# the degree of \bar Phi
```

```
degPhi=Phi1+Phi2+Phi3+2
```

```
print "The combinatorial data"
```

```
show(B)
```

```
show(Phi1)
```

```
show(Phi2)
```

```
show(Phi3)
```

The combinatorial data

$[-1, 2]$

$u \mapsto \min(-u, 0)$

$u \mapsto \min(0, u)$

$u \mapsto \min(0, u)$

Step (i) obtain a closed form for  $F_{X,\xi}(1)$

For this we have to analytically solve the integral  $\int_{\square} u \deg \bar{\Phi}(u) e^{\xi u} du$ .

```
# The integral can be solved symbolically:
```

```
F(xi)=integral(degPhi(u)*u*exp(xi*u),u,-1,B[1])
```

```
show(F(xi))
```

$$-\frac{2(\xi - 2e^{\xi} + 2)e^{(-\xi)}}{\xi^3} + \frac{2((\xi - 1)e^{(2\xi)} + 1)}{\xi^3}$$

Step (ii) find an estimate for the soliton candidate vector field  $\xi$

```
# Solve numerically
```

```
sol=find_root(F,-10,10)
```

```
print "Numerical solution:",sol
```

---

```

# Choose upper and lower bound and
# hope that the exact solution lies in between
xi_1=sol-0.0000001
xi_2=xi_1+0.0000002

#define a real value xi0 between xi_1 and xi_2
# representing the exact solution
xi0=RIF(xi_1,xi_2)

# Check whether Intermediate value theorem guarantees a zero between
# xi_1 and xi_2, i.e evaluate F at xi_1 and xi_2 using interval \
  arithmetic
if RIF(F(xi_1)) < 0 and RIF(F(xi_2)) > 0:
    print "Interval containing solution:", xi0.str(style='\
brackets')

```

Numerical solution: -0.97052220918

Interval containing solution: [-0.970522315 .. -0.970522105]

Step (iii) & (iv) obtain closed forms for  $DF_\xi(X_{y,0,1})$  and plug in the estimate for  $\xi$

For every choice of  $y \in \mathbb{P}^1$  we have to symbolically solve the integrals  $\int_{\square} e^{u\xi} \cdot \left( (1 + \Phi_y(u))^2 - (1 + \sum_{z \neq y} \Phi_z(u)) \right)$  which up to scaling with a positive constant coincide with  $DF_\xi(\mathcal{X}_{y,0,1})$ . Then we plug in the estimate for  $\xi$  into the resulting expression.

```

#check for positivity of the DF invariant for our vector field xi
print("Stability test for test configurations:")

#storage for DF values (as intervals)
IDF={}

DF1(xi)=integral(exp(xi*u)*((Phi1+1)(u)^2-(Phi3+Phi2+1)(u)^2)/2,u\
, -1,B[1])
IDF[1]=RIF(DF1(xi0)) # evaluate DF1 at xi0 using interval arithmetic
show(DF1(xi) >= IDF[1].lower())

DF2(xi)=integral(exp(xi*u)*((Phi2+1)(u)^2-(Phi1+Phi3+1)(u)^2)/2,u\
, -1,B[1])
IDF[2]=RIF(DF2(xi0))
show(DF2(xi) >= IDF[2].lower())

DF3(xi)=integral(exp(xi*u)*((Phi3+1)(u)^2-(Phi1+Phi2+1)(u)^2)/2,u\
, -1,B[1])
IDF[3]=RIF(DF3(xi0))
show(DF3(xi) >= IDF[3].lower())

DF4(xi)=integral(exp(xi*u)*((1)^2-(Phi3+Phi2+Phi1+1)(u)^2)/2,u, -1,B\
[1])
IDF[4]=RIF(DF4(xi0))

```



---

```

show(DF4(xi) >= IDF[4].lower())

if all([DF > 0 for DF in IDF.values()]):
    print("Surface is stable!")
else:
    if any([DF <= 0 for DF in IDF.values()]):
        print("Surface is not stable!")

        # print upper bound for destabilising DF value
        if IDF[1] <= 0: show(DF1(xi) <= IDF[1].upper())
        if IDF[2] <= 0: show(DF2(xi) <= IDF[2].upper())
        if IDF[3] <= 0: show(DF3(xi) <= IDF[3].upper())
        if IDF[4] <= 0: show(DF4(xi) <= IDF[4].upper())
    else:
        print("Cannot determine stability")
        # Note, that "not a > 0" does not imply "a <= 0" for \
        intervals

```

Stability test for test configurations:

$$\frac{2((\xi - 2)e^\xi + \xi + 2)e^{(-\xi)}}{\xi^3} - \frac{(\xi - 1)e^{(2\xi)} + \xi + 1}{\xi^3} \geq 0.2771940$$

$$\frac{(\xi - 1)e^{(2\xi)} + \xi + 1}{\xi^3} \geq 0.2771960$$

$$\frac{(\xi - 1)e^{(2\xi)} + \xi + 1}{\xi^3} \geq 0.2771960$$

$$\frac{2((\xi - 2)e^\xi + \xi + 2)e^{(-\xi)}}{\xi^3} + \frac{(\xi - 1)e^{(2\xi)} + \xi + 1}{\xi^3} \geq 0.8315867$$

Surface is stable!
