# Supplementary material for: On the classification of Kahler-Ricci solitons on Gorenstein del Pezzo surfaces
Source: arXiv:1705.02920 ancillary file (2018-03-10)
Supplement: Supplementary file 2 [file threefolds.pdf]

# threefolds

Hendrik Suess

05.05.2017

## 0.0.1 Smooth Fano Threefolds with 2-Torus Action

1. Q
2. 2.24
3. 2.29
4. 2.30
5. 2.31
6. 2.32
7. 3.8
8. 3.10
9. 3.18
10. 3.19
11. 3.20
12. 3.21
13. 3.22
14. 3.23
15. 3.24
16. 4.4
17. 4.5
18. 4.7
19. 4.8

---

```

# Helper functions

# The function degenerations:
# Returns the list of degeneration polytopes of given combinatorial \
  data of a T-variety.
# Takes inputs L and B, where L is a list of matrices and B is the \
  base polytope.
# Each matrix in L represents a piecewise affine function on B in \
  the following way:

# Suppose $v_j$ are the columns of $M$ in the list $L$. We then form \
  the piecewise affine function
# $\phi_M(x_1, \dots, x_n) := \min_j \{ (1, x_1, x_2, \dots, x_n) \cdot v_j \}$.

def degenerations(L,B):
    dim = L[0].nrows()
    genericfunction = matrix(QQ, dim, 1, lambda i, j: 0)
    L = L + [genericfunction]
    def shift(A,r):
        shift = matrix(QQ, A.transpose().nrows(), 1, lambda i, j: \
r);
        zeroes = matrix(QQ, A.transpose().nrows(), A.nrows() -1, \
lambda i, j: 0);
        return A + shift.augment(zeroes).transpose()
    def minsum(L):
        msCurrent = L[0]
        def minsum_step(A1,A2):
            C = matrix(QQ,A2.nrows(),1,lambda i, j: 0)
            for c in A1.columns():
                for d in A2.columns():
                    C = C.augment(d+c);
            return C.delete_columns([0])
        for l in L[1:]:
            msCurrent = minsum_step(msCurrent,l)
        return msCurrent
    def degenerations_step(L,k,B):
        up = shift(L[k],1)
        base = matrix(QQ, B.inequalities_list()[0]);
        low = L[0]; low.pop(k);
        low = minsum(low).transpose();
        up = up.transpose()
        base = base.augment(matrix(QQ, base.nrows(), 1, lambda i, \
j: 0)).transpose()
        up = up.augment(matrix(QQ, up.nrows(), 1, lambda i, j: -1)).\
transpose()
        low = low.augment(matrix(QQ, low.nrows(), 1, lambda i, j: 1))\

```

---

```

).transpose()
    low = shift(low,1)
    P = Polyhedron(ieqs = [list(v) for v in up.augment(low.\
augment(base)).columns()])
    return P;
Polyhedra = [];
for k in range(len(L)):
    Polyhedra = Polyhedra + [degenerations_step(L,k,B)];
return Polyhedra

def projection(P,F):
    A = F.as_polyhedron().equations()[0].A()
    b = F.as_polyhedron().equations()[0].b()
    A = list(A)
    B=vector(QQ,A)
    B=denominator(B)*B
    A = list(B)
    B = matrix(ZZ,B)
    K = B.right_kernel()
    if P.dimension() == 1:
        K= matrix(ZZ,[0])
    else:
        K = matrix(ZZ,K.basis())
    return [K,A]

def acoeff(F,c):
    v_0 = F.vertices()[0].vector(); v_0
    return exp(c.dot_product(v_0))

def bcoeff(F,v):
    u_0 = F.vertices()[0].vector()
    return v.dot_product(u_0)

def relvolume(P):
    if P.dimension() == 0:
        return 1
    else:
        return P.volume()

# The function intexp:
# Calculates the integral of exp(c*x) dx over the polyhedron P \
# recursively using the Barvinok method. Input is a polyhedron P,
# a sufficiently general vector L (not orthogonal, after projection,\
# to c or any face of P at any stage of the recursion),
# and a vector c for the integrand. To optimize performance values \

```

---

```

    obtained at faces are cached along the way.
def intexp(P,L,c,face=None, cache=None):
    if face is None: face = tuple(range(P.n_vertices()))
    if cache is None:
        cache = {}
    if cache.has_key(frozenset(face)):
        return cache[frozenset(face)]
    I = 0
    if c.is_zero():
        cache[face]= relvolume(P)
        return relvolume(P)
    else:
        for F in P.faces(P.dimension()-1):
            ProjMatrix,A = projection(P,F)
            n_F = -F.ambient_Hrepresentation()[0].A()
            n_F = n_F/gcd(n_F)
            coeff = acoeff(F,c)*(1/L.dot_product(c))*(L.dot_product(\
n_F))
            c_F = ProjMatrix*c
            L_F = ProjMatrix.insert_row(0,vector(ZZ,A)).transpose().\
solve_right(L)[1:]
            v_0 = F.vertices()[0].vector(); v_0
            Vert = [ProjMatrix.transpose().solve_right(v.vector() - \
v_0) for v in F.vertices()]
            face_F = tuple([face[i] for i in F.\
_ambient_Vrepresentation_indices])
            P_F = Polyhedron(vertices = Vert, backend="cdd")
            I = I + coeff*intexp(P_F,L_F,c_F,face_F,cache)
        cache[frozenset(face)]=I
    return I

# The function intexp:
# Calculates the integral of <x,v>*exp(<x,c>) dx over the polyhedron\
P recursively using the Barvinok method. Input is a polyhedron P\
,
# a sufficiently general vector L (not orthogonal, after projection,\
to c or any face of P at any stage of the recursion),
# and vectors c and v for the integrand. To optimize performance \
values obtained at faces are cached along the way.
def intexp(P,L,c,v,face=None,cache=None,cache2=None):
    if face is None: face = tuple(range(P.n_vertices()))
    if cache2 is None:
        cache2 = {}
    if cache is None:
        cache = {}
    if cache.has_key(frozenset(face)):
        return cache[frozenset(face)]

```

---

```

I = 0
if c.is_zero():
    if v.is_zero(): return 0
    for T in list(P.triangulate()):
        T = [P.Vrepresentation()[ZZ(t)].vector() for t in T]
        bary = sum(T)/len(T)
        T = Polyhedron(vertices = T)
        I = I + T.volume()*bary.dot_product(v)
else:
    for F in P.faces(P.dimension() -1):
        ProjMatrix = projection(P,F)
        L_F = ProjMatrix[0].insert_row(0,vector(ZZ,\
ProjMatrix[1])).transpose().solve_right(L)[1:]
        c_F = ProjMatrix[0]*c
        v_F = ProjMatrix[0]*v
        v_0 = F.vertices()[0].vector(); v_0
        Vert = [ProjMatrix[0].transpose().solve_right(w.\
vector() - v_0) for w in F.vertices()]
        face_F = tuple([face[i] for i in F.\
_ambient_Vrepresentation_indices])
        P_F = Polyhedron(vertices = Vert, backend="cdd")
        n_F = -F.ambient_Hrepresentation()[0].A()
        n_F = n_F/gcd(n_F)
        I = I + (L.dot_product(n_F)/L.dot_product(c))*acoeff\
(F,c)*(intexp(P_F,L_F,c_F,v_F,face_F,cache,cache2) + bcoeff(F,v)\
*intexp(P_F,L_F,c_F,face_F,cache2)) - L.dot_product(n_F)*(v.\
dot_product(L)/(L.dot_product(c)^2))*acoeff(F,c)*intexp(P_F,L_F,\
c_F,face_F,cache2)
        cache[frozenset(face)]=I
return I

```

---

No. 2.30

The combinatorial data is given by  $\square = \text{conv}((-3,0), (-2,1), (2,1), (3,0), (0,-3))$  and  $\Phi_0(x,y) = \min\{0, -x\}$ ,  $\Phi_1(x,y) = \min\{0, y\}$ ,  $\Phi_\infty(x,y) = \frac{x-y-1}{2}$ .

```

# We are working with interval arithmetic with precision of 16 bit
# this fixes the precision e.g. for evaluations of exponential \
  functions
RIF=RealIntervalField(16)

# The base polytope
B=Polyhedron(vertices = [[-3,0],[-2,1],[2,1],[3,0],[0,-3]])

# 3 PL functions on B. If phi is the minimum of affine functions of \
  the form F(x,y) = a + b*x + c*y we represent phi as
# the transpose of the matrix with rows [a,b,c].

```

---

```

Phi1 = matrix(QQ,[[0,0,0],[0,-1,0]].transpose()
Phi2 = matrix(QQ,[[0,0,0],[0,0,1]].transpose()
Phi3 = matrix(QQ,[[ -1/2,1/2,-1/2]].transpose()

PLfunctions = [Phi1,Phi2,Phi3]

# Form list of degeneration polyhedra
Polyhedra = degenerations(PLfunctions,B)

print "The combinatorial data"

graphic = B.plot().show(figsize=[3,3],title='Base Polytope B')

x,y = var('x,y')
r = vector([1,x,y])

for Phi in PLfunctions:
    if Phi.transpose().nrows() > 1:
        f(x,y) = min_symbolic(*list(r*Phi))
    else:
        f(x,y) = list(r*Phi)[0]
    print ' '
    show(f)

```

The combinatorial data

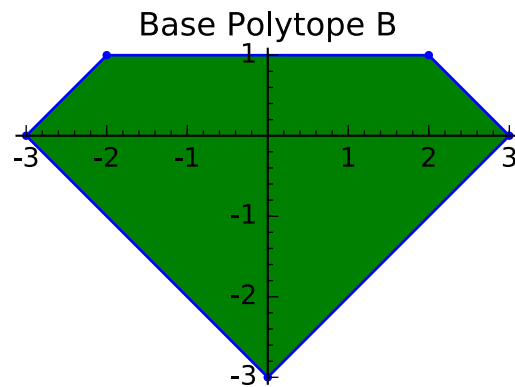

$$(x, y) \mapsto \min(0, -x)$$

$$(x, y) \mapsto \min(0, y)$$

$$(x, y) \mapsto \frac{1}{2}x - \frac{1}{2}y - \frac{1}{2}$$

Step (i) obtain a closed form for  $F_{X,\xi}$

For this note, that  $\begin{pmatrix} -1 & 0 \\ 0 & 1 \end{pmatrix}$  is a symmetry of the combinatorial data. Hence, we have  $\xi = (0, \xi_2)$ . We have to analytically solve the integral

$$\int_{\square} \langle u, v \rangle \deg \bar{\Phi}(u) e^{\langle u, (0, \xi_2) \rangle} du = \int_{\Delta_0} \langle u', (v, 0) \rangle \cdot e^{\langle u', (0, \xi_2, 0) \rangle} du'$$

for  $v$  varying over a basis of  $N_{\mathbb{R}}$ .

```
#Choose a sufficiently general value for lambda
```

```
Lambda = vector([1,3,13])
```

```
# Analytic solution of the integral
```

```
F1(xi_2) = intxexp(Polyhedra[0], Lambda, vector([0, xi_2, 0]), vector\
([1, 0, 0])).simplify_full()
```

```
F2(xi_2) = intxexp(Polyhedra[0], Lambda, vector([0, xi_2, 0]), vector\
([0, 1, 0])).simplify_full()
```

```
show(vector([F1, F2]))
```

$$\xi_2 \mapsto \left( 0, \frac{((2\xi_2^3 - 3\xi_2 - 3)e^{(4\xi_2)} + 12\xi_2 e^{(3\xi_2)} + 3\xi_2 + 3)e^{(-3\xi_2)}}{\xi_2^4} \right)$$

Step (ii) find an estimate for the soliton candidate vector field  $\xi$ .

```
# Choose upper and lower bound and
```

```
# hope that the exact solution lies in between
```

```
lower = 0.514
```

```
upper = 0.515
```

```
#define a real value xi_RIF between xi_1 and xi_2
```

```
# representing the exact solution.
```

```
xi_RIF = RIF(lower, upper)
```

```
# Check whether Intermediate value theorem guarantees a zero between
```

```
# lower and upper, i.e evaluate F2 at lower and upper using interval\
arithmetic.
```

```
if RIF(F2(lower)) < 0 and RIF(F2(upper)) > 0:
```

```
    print "Interval containing solution:", xi_RIF.str(style='\
brackets')
```

```
Interval containing solution: [0.513992 .. 0.515015]
```

Step (iii) & (iv) obtain closed forms for  $DF_{\xi}(X_{y,0,1})$  and plug in the estimate for  $\xi$

For this we first have to symbolically solve the integrals

$$h_y(\xi) := \text{vol}(\Delta_y) \cdot DF_{\xi}(X_{y,0,1}) = \int_{\Delta_y} \langle u, (0, 0, 1) \rangle e^{\langle u, (\xi, 0) \rangle} du$$

for every (admissible) choice of  $y \in \mathbb{P}^1$  and then plug in the estimate for  $\xi$  into the resulting expression.

---

```

#storage for the functions h_y
H=[]
#storage for values h_y(xi) (as intervals)
Ih=[]

#Symbollically solving integrals using Barvinok method
for P in Polyhedra:
    h(xi_2) = intxexp(P,Lambda,vector([0,xi_2,0]),vector([0,0,1])).\
    simplify_full()
    DF=RIF(h(xi_RIF))
    H.append(h); Ih.append(DF)
    show(h(xi_2) >= DF.lower())

if all([h > 0 for h in Ih]):
    print("Threefold is stable!")
else:
    if any([h <= 0 for h in Ih]):
        print("Threefold is not stable!")

        # print upper bound for destabilising DF value
        if Ih[0] <= 0: show(H[0](xi_2) <= Ih[0].upper())
        if Ih[1] <= 0: show(H[1](xi_2) <= Ih[1].upper())
        if Ih[2] <= 0: show(H[2](xi_2) <= Ih[2].upper())
        if Ih[3] <= 0: show(H[3](xi_2) <= Ih[3].upper())
    else:
        print("Cannot determine stability")
        # Note, that "not a > 0" does not imply "a <= 0" for \
        intervals
        
$$\frac{((2\xi_2^3 - 3\xi_2 - 3)e^{(4\xi_2)} + 3(3\xi_2^2 + 2)e^{(3\xi_2)} - 3\xi_2 - 3)e^{(-3\xi_2)}}{3\xi_2^4} \geq 1.088$$


$$\frac{((8\xi_2^3 + 6\xi_2^2 - 3)e^{(4\xi_2)} - 12(3\xi_2^2 - 3\xi_2 + 1)e^{(3\xi_2)} + 12\xi_2 + 15)e^{(-3\xi_2)}}{6\xi_2^4} \geq 2.178$$


$$-\frac{(2(2\xi_2^3 - 3\xi_2 - 3)e^{(4\xi_2)} - 3(3\xi_2^2 - 12\xi_2 + 2)e^{(3\xi_2)} + 12\xi_2 + 12)e^{(-3\xi_2)}}{6\xi_2^4} \geq 0.4465$$


$$\frac{((8\xi_2^3 + 6\xi_2^2 - 3)e^{(4\xi_2)} - 3(3\xi_2^2 - 2)e^{(3\xi_2)} - 6\xi_2 - 3)e^{(-3\xi_2)}}{6\xi_2^4} \geq 4.151$$


```

Threefold is stable!

---

No. 2.31

The combinatorial data is given by  $\square = \text{conv}((-3, 0), (-1, 2), (0, 2), (2, 0), (2, -1), (0, -3))$  and  $\Phi_0(x, y) = \min\{0, -x\}$ ,  $\Phi_1(x, y) = \min\{0, y\}$ ,  $\Phi_\infty(x, y) = \min\{-y, \frac{x-y-1}{2}\}$ .

```

# We are working with interval arithmetic with precision of 60 bit
# this fixes the precision e.g. for evaluations of exponential \
    functions
RIF=RealIntervalField(60)

```

---

```

# The base polytope
B=Polyhedron(vertices = [[-3,0],[-1,2],[0,2],[2,0],[2,-1],[0,-3]])

# 3 PL functions on B. If phi is the minimum of affine functions of \
  the form F(x,y) = a + b*x + c*y we represent phi as
# the transpose of the matrix with rows [a,b,c].

Phi1 = matrix(QQ,[[0,0,0],[0,-1,0]].transpose()
Phi2 = matrix(QQ,[[0,0,0],[0,0,1]].transpose()
Phi3 = matrix(QQ,[-1/2,1/2,-1/2],[0,0,-1]].transpose()

PLfunctions = [Phi1,Phi2,Phi3]

# Form list of degeneration polyhedra
Polyhedra = degenerations(PLfunctions,B)

print "The combinatorial data"

graphic = B.plot().show(figsize=[3,3],title='Base Polytope B')

x,y = var('x,y')
r = vector([1,x,y])

for Phi in PLfunctions:
    if Phi.transpose().nrows() > 1:
        f(x,y) = min_symbolic(*list(r*Phi))
    else:
        f(x,y) = list(r*Phi)[0]
    print ' '
    show(f)

```

The combinatorial data

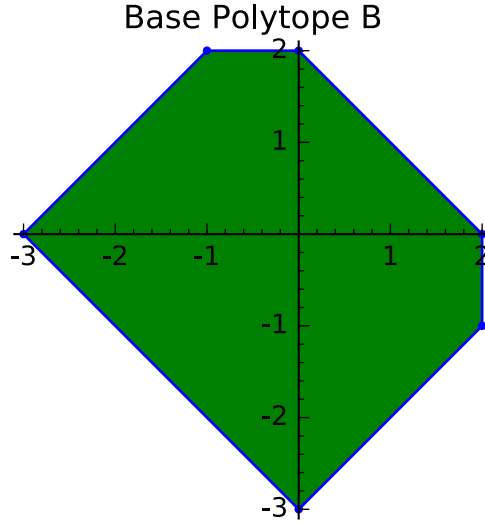

$$(x, y) \mapsto \min(0, -x)$$

$$(x, y) \mapsto \min(0, y)$$

$$(x, y) \mapsto \min\left(\frac{1}{2}x - \frac{1}{2}y - \frac{1}{2}, -y\right)$$

Step (i) obtain a closed form for  $F_{X,\xi}$

For this note, that  $\begin{pmatrix} 0 & 1 \\ 1 & 0 \end{pmatrix}$  is a symmetry of the combinatorial data. Hence, we have  $\xi = (\xi_1, \xi_1)$ . We have to analytically solve the integral

$$\int_{\square} \langle u, v \rangle \deg \bar{\Phi}(u) e^{\langle u, \xi \rangle} du = \int_{\Delta_0} \langle u', (v, 0) \rangle \cdot e^{\langle u', (\xi, 0) \rangle} du'$$

for  $v$  varying over a basis of  $N_{\mathbb{R}}$ .

#Choose a sufficiently general value for lambda

Lambda = vector([1,3,13])

# Analytic solution of the integral

F1(xi\_1) = intxexp(Polyhedra[0], Lambda, vector([xi\_1, xi\_1, 0]), vector([1, -1, 0])).simplify\_full()

F2(xi\_1) = intxexp(Polyhedra[0], Lambda, vector([xi\_1, xi\_1, 0]), vector([1, 1, 0])).simplify\_full()

show(vector([F1, F2]))

$$\xi_1 \mapsto \left(0, -\frac{(9\xi_1^2 - 8(\xi_1^2 - \xi_1))e^{5\xi_1} + (3\xi_1^2 - 5\xi_1 - 3)e^{4\xi_1} + 9\xi_1 + 3)e^{(-3\xi_1)}}{2\xi_1^4}\right)$$

Step (ii) find an estimate for the soliton candidate vector field  $\xi$ .

# Choose upper and lower bound and

---

```
# hope that the exact solution lies in between
lower = 0.285497
upper = 0.285507
```

```
#define a real value xi_RIF between xi_1 and xi_2
# representing the exact solution.
xi_RIF = RIF(lower , upper)
```

```
# Check whether Intermediate value theorem guarantees a zero between
# lower and upper, i.e evaluate F2 at lower and upper using interval\
arithmetic.
if RIF(F2(lower)) < 0 and RIF(F2(upper)) > 0:
    print "Interval containing solution:", xi_RIF.str(style='\
brackets')
```

```
Interval containing solution: [0.28549700000000000077 .. 0.285507000000000001078]
```

Step (iii) & (iv) obtain closed forms for  $DF_\xi(X_{y,0,1})$  and plug in the estimate for  $\xi$   
For this we first have to symbolically solve the integrals

$$h_y(\xi) := \text{vol}(\Delta_y) \cdot DF_\xi(\mathcal{X}_{y,0,1}) = \int_{\Delta_y} \langle u, (0, 0, 1) \rangle e^{\langle u, (\xi, 0) \rangle} du$$

for every (admissible) choice of  $y \in \mathbb{P}^1$  and then plug in the estimate for  $\xi$  into the resulting expression.

```
#storage for the functions h_y
H=[]
#storage for values h_y(xi) (as intervals)
Ih=[]

#Symbollically solving integrals using Barvinok method
for P in Polyhedra:
    h(xi_2) = intxexp(P,Lambda,vector([xi_2,xi_2,0]),vector([0,0,1])\
).simplify_full()
    DF=RIF(h(xi_RIF))
    H.append(h); Ih.append(DF)
    show(h(xi_2) >= DF.lower())

if all([h > 0 for h in Ih]):
    print("Threefold is stable!")
else:
    if any([h <= 0 for h in Ih]):
        print("Threefold is not stable!")

    # print upper bound for destabilising DF value
    if Ih[0] <= 0: show(H[0](xi_2) <= Ih[0].upper())
    if Ih[1] <= 0: show(H[1](xi_2) <= Ih[1].upper())
    if Ih[2] <= 0: show(H[2](xi_2) <= Ih[2].upper())
```

---

```

    if Ih[3] <= 0: show(H[3](xi_2) <= Ih[3].upper())
    else:
        print("Cannot determine stability")
        # Note, that "not a > 0" does not imply "a <= 0" for \
intervals

$$\frac{(12\xi_2^2 + (4\xi_2^2 + 2\xi_2 - 3)e^{(4\xi_2)} + 10\xi_2 + 3)e^{(-3\xi_2)}}{8\xi_2^4} \geq 1.9509141924719434162$$


$$- \frac{(6\xi_2^2 - 16(\xi_2^2 - \xi_2)e^{(5\xi_2)} + (2\xi_2^2 - 12\xi_2 - 3)e^{(4\xi_2)} + 8\xi_2 + 3)e^{(-3\xi_2)}}{8\xi_2^4} \geq 1.9410579647693620622$$


$$\frac{(3\xi_2^2 - (3\xi_2^2 + 4\xi_2 + 2)e^{(4\xi_2)} + 4\xi_2 + 4e^{(5\xi_2)} - 4e^{(3\xi_2)} + 2)e^{(-3\xi_2)}}{4\xi_2^4} \geq 0.46321187855599924134$$


$$\frac{(6\xi_2^2 + 4(2\xi_2^2 - 2\xi_2 + 1)e^{(5\xi_2)} - (2\xi_2^2 - 3\xi_2 + 2)e^{(4\xi_2)} + 5\xi_2 - 4e^{(3\xi_2)} + 2)e^{(-3\xi_2)}}{4\xi_2^4} \geq 4.370374945004598$$


```

Threefold is stable!

---

No. 3.8\*

The combinatorial data is given by  $\square = \text{conv}((-2, -1), (-2, 1), (1, 1), (3, -1), (3, -2), (-1, -2))$   
and  $\Phi_0(x, y) = \min\{0, \frac{-x-1}{2}\}$ ,  $\Phi_1(x, y) = \min\{0, \frac{-y-1}{2}\}$ ,  $\Phi_\infty(x, y) = \min\{0, \frac{x+y-1}{2}\}$ .

```

# We are working with interval arithmetic with precision of 60 bit
# this fixes the precision e.g. for evaluations of exponential \
functions
RIF=RealIntervalField(60)

# The base polytope
B=Polyhedron(vertices = \
    [[-2, -1], [-2, 1], [1, 1], [3, -1], [3, -2], [-1, -2]])

# 3 PL functions on B. If phi is the minimum of affine functions of \
the form F(x,y) = a + b*x + c*y we represent phi as
# the transpose of the matrix with rows [a,b,c].

Phi1 = matrix(QQ, [[0, 0, 0], [-1/2, -1/2, 0]]) . transpose()
Phi2 = matrix(QQ, [[0, 0, 0], [-1/2, 0, -1/2]]) . transpose()
Phi3 = matrix(QQ, [[0, 0, 0], [-1/2, 1/2, 1/2]]) . transpose();

PLfunctions = [Phi1, Phi2, Phi3]

# Form list of degeneration polyhedra
Polyhedra = degenerations(PLfunctions, B)

print "The combinatorial data"

```

---

```

graphic = B.plot().show(figsize=[3,3],title='Base Polytope B')

x,y = var('x,y')
r = vector([1,x,y])

for Phi in PLfunctions:
    if Phi.transpose().nrows() > 1:
        f(x,y) = min_symbolic(*list(r*Phi))
    else:
        f(x,y) = list(r*Phi)[0]
    print ' '
    show(f)

```

The combinatorial data

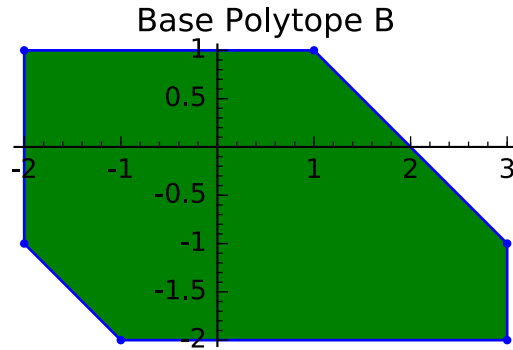

$$(x, y) \mapsto \min \left( 0, -\frac{1}{2}x - \frac{1}{2} \right)$$

$$(x, y) \mapsto \min \left( 0, -\frac{1}{2}y - \frac{1}{2} \right)$$

$$(x, y) \mapsto \min \left( 0, \frac{1}{2}x + \frac{1}{2}y - \frac{1}{2} \right)$$

Step (i) obtain a closed form for  $F_{X,\xi}$

For this note, that  $\begin{pmatrix} -1 & -1 \\ 0 & 1 \end{pmatrix}$  is a symmetry of the combinatorial data. Hence, we have  $\xi = (0, \xi_2)$ . We have to analytically solve the integral

$$\int_{\square} \langle u, v \rangle \deg \bar{\Phi}(u) e^{\langle u, \xi \rangle} du = \int_{\Delta_0} \langle u', (v, 0) \rangle \cdot e^{\langle u', (\xi, 0) \rangle} du'$$

for  $v$  varying over a basis of  $N_{\mathbb{R}}$ .

```

#Choose a sufficiently general value for lambda
Lambda = vector([1,5,13])

```

```

# Analytic solution of the integral
F1(xi_2) = intxexp(Polyhedra[0], Lambda, vector([0, xi_2, 0]), vector\
([1, 0, 0])).simplify_full()

```

---

```
F2(xi_2) = intxexp(Polyhedra[0], Lambda, vector([0, xi_2, 0]), vector\
([0, 1, 0])).simplify_full()
```

```
show(vector([F1, F2]))
```

$$\xi_2 \mapsto \left( -\frac{((2\xi_2^2 - \xi_2 - 2)e^{(3\xi_2)} + 5(\xi_2 + 2)e^{\xi_2} - 8\xi_2 - 8)e^{(-2\xi_2)}}{4\xi_2^3}, \frac{((2\xi_2^2 - \xi_2 - 2)e^{(3\xi_2)} + 5(\xi_2 + 2)e^{\xi_2} - 8\xi_2 - 8)e^{(-2\xi_2)}}{2\xi_2^3} \right)$$

Step (ii) find an estimate for the soliton candidate vector field  $\xi$ .

```
# Choose upper and lower bound and
# hope that the exact solution lies in between
find_root(F2, -10, 10)
```

```
lower = 0.799716
upper = 0.799717
```

```
#define a real value xi_RIF between xi_1 and xi_2
# representing the exact solution.
xi_RIF = RIF(lower, upper)
```

```
# Check whether Intermediate value theorem guarantees a zero between
# lower and upper, i.e evaluate F2 at lower and upper using interval\
arithmetic.
if RIF(F2(lower)) < 0 and RIF(F2(upper)) > 0:
    print "Interval containing solution:", xi_RIF.str(style='\
brackets')
```

```
0.7997160277154249
```

```
Interval containing solution: [0.7997159999999998242 .. 0.79971700000000001119]
```

Step (iii) & (iv) obtain closed forms for  $DF_\xi(X_{y,0,1})$  and plug in the estimate for  $\xi$   
For this we first have to symbolically solve the integrals

$$h_y(\xi) := \text{vol}(\Delta_y) \cdot DF_\xi(\mathcal{X}_{y,0,1}) = \int_{\Delta_y} \langle u, (0, 0, 1) \rangle e^{\langle u, (\xi, 0) \rangle} du$$

for every choice of  $y \in \mathbb{P}^1$  and then plug in the estimate for  $\xi$  into the resulting expression.

```
#storage for the functions h_y
```

```
H=[]
```

```
#storage for values h_y(xi) (as intervals)
```

```
Ih=[]
```

```
#Symbollically solving integrals using Barvinok method
```

```
for P in Polyhedra:
```

```
    h(xi_2) = intxexp(P, Lambda, vector([0, xi_2, 0]), vector([0, 0, 1])).\
    simplify_full()
```

```
    DF=RIF(h(xi_RIF))
```

```
    H.append(h); Ih.append(DF)
```

---

```

show(h(xi_2) >= DF.lower())

if all([h > 0 for h in Ih]):
    print("Threefold is stable!")
else:
    if any([h <= 0 for h in Ih]):
        print("Threefold is not stable!")

    # print upper bound for destabilising DF value
    if Ih[0] <= 0: show(H[0](xi_2) <= Ih[0].upper())
    if Ih[1] <= 0: show(H[1](xi_2) <= Ih[1].upper())
    if Ih[2] <= 0: show(H[2](xi_2) <= Ih[2].upper())
    if Ih[3] <= 0: show(H[3](xi_2) <= Ih[3].upper())
    else:
        print("Cannot determine stability")
        # Note, that "not a > 0" does not imply "a <= 0" for \
intervals


$$\frac{((2\xi_2^2 - 1)e^{(2\xi_2)} + 2\xi_2 + 1)e^{(-\xi_2)}}{4\xi_2^3} \geq 0.87460114755231644$$


$$\frac{(48\xi_2^2 - (5\xi_2^3 - 9\xi_2^2 - 12\xi_2)e^{(3\xi_2)} - 6(10\xi_2^2 + 5\xi_2 + 1)e^{\xi_2} + 24\xi_2 + 6)e^{(-2\xi_2)}}{24\xi_2^4} \geq 0.92008662275004536$$


$$\frac{((2\xi_2^2 - 1)e^{(2\xi_2)} + 2\xi_2 + 1)e^{(-\xi_2)}}{4\xi_2^3} \geq 0.87460114755231644$$


$$\frac{(48\xi_2^2 + (19\xi_2^3 + 9\xi_2^2)e^{(3\xi_2)} - 6(6\xi_2^2 + 3\xi_2 + 1)e^{\xi_2} + 24\xi_2 + 6)e^{(-2\xi_2)}}{24\xi_2^4} \geq 2.6692906048111306$$


Threefold is stable!

```

---

No. 3.18

The combinatorial data is given by  $\square = \text{conv}((-3, 0), (-2, 1), (2, 1), (3, 0), (1, -2), (-1, -2))$  and  $\Phi_0(x, y) = \min\{0, \frac{-x-1}{2}, -x\}$ ,  $\Phi_1(x, y) = \min\{0, y\}$ ,  $\Phi_\infty(x, y) = \frac{x-y-1}{2}$ .

```

# We are working with interval arithmetic with precision of 60 bit
# this fixes the precision e.g. for evaluations of exponential \
functions
RIF=RealIntervalField(16)

# The base polytope
B=Polyhedron(vertices = [[-3, 0], [-2, 1], [2, 1], [3, 0], [1, -2], [-1, -2]])

# 3 PL functions on B. If phi is the minimum of affine functions of \
the form F(x,y) = a + b*x + c*y we represent phi as
# the transpose of the matrix with rows [a,b,c].

Phi1 = matrix(QQ, [[0, 0, 0], [-1/2, -1/2, 0], [0, -1, 0]]).transpose()
Phi2 = matrix(QQ, [[0, 0, 0], [0, 0, 1]]).transpose()
Phi3 = matrix(QQ, [[-1/2, 1/2, -1/2]]).transpose();

```

---

```

PLfunctions = [Phi1,Phi2,Phi3]

# Form list of degeneration polyhedra
Polyhedra = degenerations(PLfunctions,B)

print "The combinatorial data"

graphic = B.plot().show(figsize=[3,3],title='Base Polytope B')

x,y = var('x,y')
r = vector([1,x,y])

for Phi in PLfunctions:
    if Phi.transpose().nrows() > 1:
        f(x,y) = min_symbolic(*list(r*Phi))
    else:
        f(x,y) = list(r*Phi)[0]
    print ' '
    show(f)

```

The combinatorial data

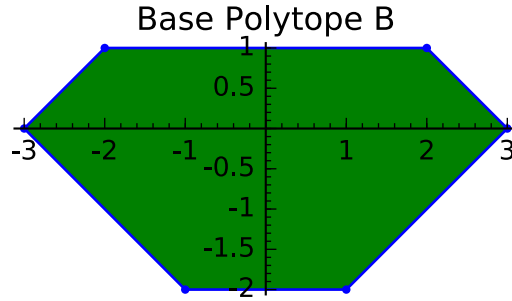

$$(x, y) \mapsto \min\left(0, -\frac{1}{2}x - \frac{1}{2}, -x\right)$$

$$(x, y) \mapsto \min(0, y)$$

$$(x, y) \mapsto \frac{1}{2}x - \frac{1}{2}y - \frac{1}{2}$$

Step (i) obtain a closed form for  $F_{X,\xi}$

For this note, that  $\begin{pmatrix} -1 & 0 \\ 0 & 1 \end{pmatrix}$  is a symmetry of the combinatorial data. Hence, we have  $\xi = (0, \xi_2)$ . We have to analytically solve the integral

$$\int_{\square} \langle u, v \rangle \deg \bar{\Phi}(u) e^{\langle u, \xi \rangle} du = \int_{\Delta_0} \langle u', (v, 0) \rangle \cdot e^{\langle u', (\xi, 0) \rangle} du'$$

for  $v$  varying over a basis of  $N_{\mathbb{R}}$ .

```
#Choose a sufficiently general value for lambda
Lambda = vector([1,3,13])

# Analytic solution of the integral
F1(xi_2) = intxexp(Polyhedra[0], Lambda, vector([0, xi_2, 0]), vector\
([1, 0, 0])).simplify_full()
F2(xi_2) = intxexp(Polyhedra[0], Lambda, vector([0, xi_2, 0]), vector\
([0, 1, 0])).simplify_full()

show(vector([F1, F2]))
```

$$\xi_2 \mapsto \left( 0, -\frac{(4\xi_2^2 - (3\xi_2^3 + \xi_2^2 - 6\xi_2 - 6)e^{(3\xi_2)} - 24\xi_2e^{(2\xi_2)} - 6)e^{(-2\xi_2)}}{2\xi_2^4} \right)$$

Step (ii) find an estimate for the soliton candidate vector field  $\xi$ .

```
# Choose upper and lower bound and
# hope that the exact solution lies in between
lower = 0.3796905
upper = 0.3797005

#define a real value xi_RIF between xi_1 and xi_2
# representing the exact solution.
xi_RIF = RIF(lower, upper)

# Check whether Intermediate value theorem guarantees a zero between
# lower and upper, i.e evaluate F2 at lower and upper using interval\
arithmetic.
if RIF(F2(lower)) < 0 and RIF(F2(upper)) > 0:
    print "Interval containing solution:", xi_RIF.str(style='\
brackets')
```

Interval containing solution: [0.379684 .. 0.379708]

Step (iii) & (iv) obtain closed forms for  $DF_{\xi}(X_{y,0,1})$  and plug in the estimate for  $\xi$   
For this we first have to symbolically solve the integrals

$$h_y(\xi) := \text{vol}(\Delta_y) \cdot DF_{\xi}(X_{y,0,1}) = \int_{\Delta_y} \langle u, (0, 0, 1) \rangle e^{\langle u, (\xi, 0) \rangle} du$$

for every (admissible) choice of  $y \in \mathbb{P}^1$  and then plug in the estimate for  $\xi$  into the resulting expression.

```
#storage for the functions h_y
H=[]
#storage for values h_y(xi) (as intervals)
Ih=[]
```

---

```

#Symbollically solving integrals using Barvinok method
for P in Polyhedra:
    h(xi_2) = intxexp(P,Lambda,vector([0,xi_2,0]),vector([0,0,1])).\
simplify_full()
    DF=RIF(h(xi_RIF))
    H.append(h); Ih.append(DF)
    show(h(xi_2) >= DF.lower())

if all([h > 0 for h in Ih]):
    print("Threefold is stable!")
else:
    if any([h <= 0 for h in Ih]):
        print("Threefold is not stable!")

        # print upper bound for destabilising DF value
        if Ih[0] <= 0: show(H[0](xi_2) <= Ih[0].upper())
        if Ih[1] <= 0: show(H[1](xi_2) <= Ih[1].upper())
        if Ih[2] <= 0: show(H[2](xi_2) <= Ih[2].upper())
        if Ih[3] <= 0: show(H[3](xi_2) <= Ih[3].upper())
    else:
        print("Cannot determine stability")
        # Note, that "not a > 0" does not imply "a <= 0" for \
intervals


$$\frac{(3\xi_2^2 + 2(\xi_2^3 - 3\xi_2 - 3)e^{(3\xi_2)} + 6(3\xi_2^2 + 2)e^{(2\xi_2)} - 6)e^{(-2\xi_2)}}{6\xi_2^4} \geq 0.3694$$


$$\frac{(12\xi_2^2 - (14\xi_2^3 + 15\xi_2^2 - 6)e^{(3\xi_2)} + 24(3\xi_2^2 - 3\xi_2 + 1)e^{(2\xi_2)} + 6\xi_2 - 30)e^{(-2\xi_2)}}{12\xi_2^4} \geq 2.516$$


$$\frac{(9\xi_2^2 - 2(\xi_2^3 - 3\xi_2 - 3)e^{(3\xi_2)} + 6(\xi_2^2 - 6\xi_2 + 1)e^{(2\xi_2)} - 12)e^{(-2\xi_2)}}{6\xi_2^4} \geq 1.013$$


$$\frac{(12\xi_2^2 + (14\xi_2^3 + 15\xi_2^2 - 6)e^{(3\xi_2)} - 12(2\xi_2^2 - 1)e^{(2\xi_2)} - 6\xi_2 - 6)e^{(-2\xi_2)}}{12\xi_2^4} \geq 3.946$$


```

Threefold is stable!

---

No. 3.21

The combinatorial data is given by  $\square = \text{conv}((-2, 1), (-3, 3), (-1, 3), (1, -2), (3, -3), (3, -1))$  and  $\Phi_0(x, y) = \min\{0, \frac{-x-1}{2}\}$ ,  $\Phi_1(x, y) = \min\{0, \frac{-y-1}{2}\}$ ,  $\Phi_\infty(x, y) = \min\{0, x + y\}$ .

```

# We are working with interval arithmetic with precision of 60 bit
# this fixes the precision e.g. for evaluations of exponential \
functions
RIF=RealIntervalField(16)

```

```

# The base polytope

```

```

B=Polyhedron(vertices = [[-2,1],[-3,3],[-1,3],[1,-2],[3,-3],[3,-1]])

```

```

# 3 PL functions on B. If phi is the minimum of affine functions of \

```

---

```

    the form  $F(x,y) = a + b*x + c*y$  we represent phi as
# the transpose of the matrix with rows [a,b,c].

Phi1 = matrix(QQ,[[0,0,0],[-1/2,-1/2,0]].transpose()
Phi2 = matrix(QQ,[[0,0,0],[-1/2,0,-1/2]].transpose()
Phi3 = matrix(QQ,[[0,0,0],[0,1,1]].transpose()

PLfunctions = [Phi1,Phi2,Phi3]

# Form list of degeneration polyhedra
Polyhedra = degenerations(PLfunctions,B)

print "The combinatorial data"

graphic = B.plot().show(figsize=[3,3],title='Base Polytope B')

x,y = var('x,y')
r = vector([1,x,y])

for Phi in PLfunctions:
    if Phi.transpose().nrows() > 1:
        f(x,y) = min_symbolic(*list(r*Phi))
    else:
        f(x,y) = list(r*Phi)[0]
    print ' '
    show(f)

```

The combinatorial data

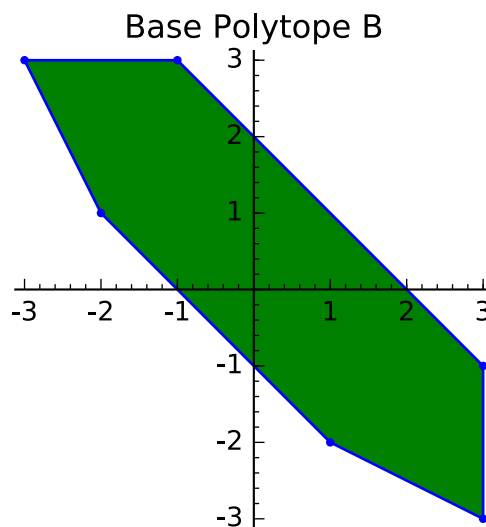

$$(x, y) \mapsto \min \left( 0, -\frac{1}{2}x - \frac{1}{2} \right)$$

$$(x, y) \mapsto \min \left( 0, -\frac{1}{2}y - \frac{1}{2} \right)$$

$$(x, y) \mapsto \min(0, x + y)$$

Step (i) obtain a closed form for  $F_{X,\xi}$

For this note, that  $\begin{pmatrix} 0 & 1 \\ 1 & 0 \end{pmatrix}$  is a symmetry of the combinatorial data. Hence we have  $\xi = (\xi_1, \xi_1)$ . We have to analytically solve the integral

$$\int_{\square} \langle u, v \rangle \deg \bar{\Phi}(u) e^{\langle u, \xi \rangle} du = \int_{\Delta_0} \langle u', (v, 0) \rangle \cdot e^{\langle u', (\xi, 0) \rangle} du'$$

for  $v$  varying over a basis of  $N_{\mathbb{R}}$ .

#Choose a sufficiently general value for Lambda

Lambda = vector([1,3,13])

# Analytic solution of the integral

F1(xi\_1) = intxexp(Polyhedra[0], Lambda, vector([xi\_1, xi\_1, 0]), vector([1, -1, 0])).simplify\_full()

F2(xi\_1) = intxexp(Polyhedra[0], Lambda, vector([xi\_1, xi\_1, 0]), vector([1, 1, 0])).simplify\_full()

show(vector([F1, F2]))

$$\xi_1 \mapsto \left( 0, \frac{(\xi_1^3 - \xi_1^2 + 4(\xi_1^2 - \xi_1)e^{(3\xi_1)} + 6(2\xi_1 - 1)e^{\xi_1} - 2\xi_1 + 6)e^{(-\xi_1)}}{\xi_1^4} \right)$$

Step (ii) find an estimate for the soliton candidate vector field  $\xi$ .

# Choose upper and lower bound and

# hope that the exact solution lies in between

find\_root(F2, -10, 10)

lower = -0.69631193

upper = -0.69621193

#define a real value xi\_RIF between xi\_1 and xi\_2

# representing the exact solution.

xi\_RIF = RIF(lower, upper)

# Check whether Intermediate value theorem guarantees a zero between

# lower and upper, i.e evaluate F2 at lower and upper using interval arithmetic.

if RIF(F2(lower)) < 0 and RIF(F2(upper)) > 0:

    print "Interval containing solution:", xi\_RIF.str(style='brackets')

-0.6962119314891655

Interval containing solution: [-0.696320 .. -0.696197]

---

Step (iii) & (iv) obtain closed forms for  $DF_\xi(X_{y,0,1})$  and plug in the estimate for  $\xi$   
 For this we first have to symbolically solve the integrals

$$h_y(\xi) := \text{vol}(\Delta_y) \cdot DF_\xi(\mathcal{X}_{y,0,1}) = \int_{\Delta_y} \langle u, (0, 0, 1) \rangle e^{\langle u, (\xi, 0) \rangle} du$$

for every choice of  $y \in \mathbb{P}^1$  and then plug in the estimate for  $\xi$  into the resulting expression.

```
#storage for the functions h_y
H=[]
#storage for values h_y(xi) (as intervals)
Ih=[]

#Symbollically solving integrals using Barvinok method
for P in Polyhedra:
    h(xi_2) = intxexp(P,Lambda,vector([xi_2,xi_2,0]),vector([0,0,1])\
    ).simplify_full()
    DF=RIF(h(xi_RIF))
    H.append(h); Ih.append(DF)
    show(h(xi_2) >= DF.lower())

if all([h > 0 for h in Ih]):
    print("Threefold is stable!")
else:
    if any([h <= 0 for h in Ih]):
        print("Threefold is not stable!")

    # print upper bound for destabilising DF value
    if Ih[0] <= 0: show(H[0](xi_2) <= Ih[0].upper())
    if Ih[1] <= 0: show(H[1](xi_2) <= Ih[1].upper())
    if Ih[2] <= 0: show(H[2](xi_2) <= Ih[2].upper())
    if Ih[3] <= 0: show(H[3](xi_2) <= Ih[3].upper())
    else:
        print("Cannot determine stability")
        # Note, that "not a > 0" does not imply "a <= 0" for \
intervals
```

$$\begin{aligned} & - \frac{(\xi_2^3 - \xi_2^2 - 2(2\xi_2^2 - 4\xi_2 + 3)e^{\xi_2} - 2\xi_2 + 6)e^{(-\xi_2)}}{2\xi_2^4} \geq 0.6910 \\ & - \frac{(\xi_2^3 - \xi_2^2 - 2(2\xi_2^2 - 4\xi_2 + 3)e^{\xi_2} - 2\xi_2 + 6)e^{(-\xi_2)}}{2\xi_2^4} \geq 0.6910 \\ & \frac{(5\xi_2^3 + 9\xi_2^2 + 6(8\xi_2^2 - 4\xi_2 + 1)e^{(3\xi_2)} - 24(6\xi_2^2 - 8\xi_2 + 5)e^{\xi_2} - 66\xi_2 + 114)e^{(-\xi_2)}}{24\xi_2^4} \geq 2.500 \\ & - \frac{(19\xi_2^3 - 33\xi_2^2 - 6(8\xi_2^2 - 4\xi_2 + 1)e^{(3\xi_2)} + 24(2\xi_2^2 - 1)e^{\xi_2} + 18\xi_2 + 30)e^{(-\xi_2)}}{24\xi_2^4} \geq 3.907 \end{aligned}$$

Threefold is stable!

---

The combinatorial data is given by  $\square = \text{conv}((-3, -1), (-3, 0), (-1, 1), (1, 1), (3, 0), (3, -1))$  and  $\Phi_0(x, y) = \min\{0, -x\}$ ,  $\Phi_1(x, y) = \min\{0, -y\}$ ,  $\Phi_\infty(x, y) = \frac{x-1}{2}$ .

```
# We are working with interval arithmetic with precision of 60 bit
# this fixes the precision e.g. for evaluations of exponential \
  functions
RIF=RealIntervalField(16)

# The base polytope
B=Polyhedron(vertices = [[-3, -1], [-3, 0], [-1, 1], [1, 1], [3, 0], [3, -1]])

# 3 PL functions on B. If phi is the minimum of affine functions of \
  the form F(x,y) = a + b*x + c*y we represent phi as
# the transpose of the matrix with rows [a,b,c].

Phi1 = matrix(QQ, [[0, 0, 0], [0, -1, 0]]).transpose()
Phi2 = matrix(QQ, [[0, 0, 0], [0, 0, -1]]).transpose()
Phi3 = matrix(QQ, [[-1/2, 1/2, 0]]).transpose()

PLfunctions = [Phi1, Phi2, Phi3]

# Form list of degeneration polyhedra
Polyhedra = degenerations(PLfunctions, B)

print "The combinatorial data"

graphic = B.plot().show(figsize=[3,3], title='Base Polytope B')

x,y = var('x,y')
r = vector([1,x,y])

for Phi in PLfunctions:
    if Phi.transpose().nrows() > 1:
        f(x,y) = min_symbolic(*list(r*Phi))
    else:
        f(x,y) = list(r*Phi)[0]
    print ' '
    show(f)
```

The combinatorial data

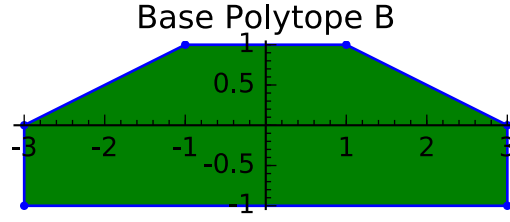

$$(x, y) \mapsto \min(0, -x)$$

$$(x, y) \mapsto \min(0, -y)$$

$$(x, y) \mapsto \frac{1}{2}x - \frac{1}{2}$$

Step (i) obtain a closed form for  $F_{X,\xi}$

For this note, that  $\begin{pmatrix} -1 & 0 \\ 0 & 1 \end{pmatrix}$  is a symmetry of the combinatorial data. Hence, we have  $\xi = (0, \xi_2)$ . We have to analytically solve the integral

$$\int_{\square} \langle u, v \rangle \deg \bar{\Phi}(u) e^{\langle u, \xi \rangle} du = \int_{\Delta_0} \langle u', (v, 0) \rangle \cdot e^{\langle u', (\xi, 0) \rangle} du'$$

for  $v$  varying over a basis of  $N_{\mathbb{R}}$ .

#Choose a sufficiently general value for lambda

Lambda = vector([1,5,13])

# Analytic solution of the integral

F1(xi\_2) = intxexp(Polyhedra[0], Lambda, vector([0, xi\_2, 0]), vector([1, 0, 0])).simplify\_full()

F2(xi\_2) = intxexp(Polyhedra[0], Lambda, vector([0, xi\_2, 0]), vector([0, 1, 0])).simplify\_full()

show(vector([F1, F2]))

$$\xi_2 \mapsto \left( 0, \frac{(9\xi_2^3 + 9\xi_2^2 + (\xi_2^3 + 3\xi_2^2 - 24)e^{(2\xi_2)} + 24(\xi_2 + 1)e^{\xi_2})e^{(-\xi_2)})}{2\xi_2^4} \right)$$

Step (ii) find an estimate for the soliton candidate vector field  $\xi$ .

# Choose upper and lower bound and

# hope that the exact solution lies in between

find\_root(F2, -10, 10)

lower = 0.9147877

upper = 0.9147977

#define a real value xi\_RIF between xi\_1 and xi\_2

# representing the exact solution.

xi\_RIF = RIF(lower, upper)

---

```
# Check whether Intermediate value theorem guarantees a zero between
# lower and upper, i.e evaluate F2 at lower and upper using interval\
arithmetic.
if RIF(F2(lower)) < 0 and RIF(F2(upper)) > 0:
    print "Interval containing solution:", xi_RIF.str(style='\
brackets')
```

0.9147877132620504

Interval containing solution: [0.914779 .. 0.914811]

Step (iii) & (iv) obtain closed forms for  $DF_\xi(X_{y,0,1})$  and plug in the estimate for  $\xi$

For this we first have to symbolically solve the integrals

$$h_y(\xi) := \text{vol}(\Delta_y) \cdot DF_\xi(\mathcal{X}_{y,0,1}) = \int_{\Delta_y} \langle u, (0, 0, 1) \rangle e^{\langle u, (\xi, 0) \rangle} du$$

for every choice of  $y \in \mathbb{P}^1$  and then plug in the estimate for  $\xi$  into the resulting expression.

```
#storage for the functions h_y
H=[]
#storage for values h_y(xi) (as intervals)
Ih=[]

#Symbollically solving integrals using Barvinok method
for P in Polyhedra:
    h(xi_2) = intxexp(P,Lambda,vector([0,xi_2,0]),vector([0,0,1])).\
simplify_full()
    DF=RIF(h(xi_RIF))
    H.append(h); Ih.append(DF)
    show(h(xi_2) >= DF.lower())

if all([h > 0 for h in Ih]):
    print("Threefold is stable!")
else:
    if any([h <= 0 for h in Ih]):
        print("Threefold is not stable!")

        # print upper bound for destabilising DF value
        if Ih[0] <= 0: show(H[0](xi_2) <= Ih[0].upper())
        if Ih[1] <= 0: show(H[1](xi_2) <= Ih[1].upper())
        if Ih[2] <= 0: show(H[2](xi_2) <= Ih[2].upper())
        if Ih[3] <= 0: show(H[3](xi_2) <= Ih[3].upper())
    else:
        print("Cannot determine stability")
        # Note, that "not a > 0" does not imply "a <= 0" for \
intervals
```

$$\frac{9\xi_2^2 + (\xi_2^3 + 3\xi_2^2 - 24)e^{\xi_2} + 24\xi_2 + 24}{3\xi_2^4} \geq 0.8323$$

---


$$\frac{(27\xi_2^3 + (\xi_2^3 - 24\xi_2 - 96)e^{(2\xi_2)} + 24(3\xi_2^2 + 5\xi_2 + 4)e^{\xi_2})e^{(-\xi_2)}}{12\xi_2^4} \geq 2.164$$

$$\frac{9\xi_2^2 + (\xi_2^3 + 3\xi_2^2 - 24)e^{\xi_2} + 24\xi_2 + 24}{6\xi_2^4} \geq 0.4161$$

$$\frac{(27\xi_2^3 - (5\xi_2^3 + 18\xi_2^2 + 24\xi_2 - 48)e^{(2\xi_2)} + 6(3\xi_2^2 - 4\xi_2 - 8)e^{\xi_2})e^{(-\xi_2)}}{12\xi_2^4} \geq 3.419$$

Threefold is stable!

---

No. 3.23

The combinatorial data is given by  $\square = \text{conv}((-3, 0), (-2, 1), (1, 1), (2, 0), (2, -1), (0, 3))$  and  $\Phi_0(x, y) = \min\{0, -x\}$ ,  $\Phi_1(x, y) = \min\{0, y\}$ ,  $\Phi_\infty(x, y) = \min\{-y, \frac{x-y-1}{2}\}$ .

```
# We are working with interval arithmetic with precision of 40 bit
# this fixes the precision e.g. for evaluations of exponential \
  functions
```

```
RIF=RealIntervalField(40)
```

```
# The base polytope
```

```
B=Polyhedron(vertices = [[-3,0],[-2,1],[1,1],[2,0],[2,-1],[0,-3]])
```

```
# 3 PL functions on B. If phi is the minimum of affine functions of \
  the form F(x,y) = a + b*x + c*y we represent phi as
# the transpose of the matrix with rows [a,b,c].
```

```
Phi1 = matrix(QQ,[[0,0,0],[0,-1,0]].transpose()
```

```
Phi2 = matrix(QQ,[[0,0,0],[0,0,1]].transpose()
```

```
Phi3 = matrix(QQ,[-1/2,1/2,-1/2],[0,0,-1]].transpose())
```

```
PLfunctions = [Phi1,Phi2,Phi3]
```

```
# Form list of degeneration polyhedra
```

```
Polyhedra = degenerations(PLfunctions,B)
```

```
print "The combinatorial data"
```

```
graphic = B.plot().show(figsize=[3,3],title='Base Polytope B')
```

```
x,y = var('x,y')
```

```
r = vector([1,x,y])
```

```
for Phi in PLfunctions:
```

```
    if Phi.transpose().nrows() > 1:
```

```
        f(x,y) = min_symbolic(*list(r*Phi))
```

```

else :
    f(x,y) = list(r*Phi)[0]
print ' '
show(f)

```

The combinatorial data

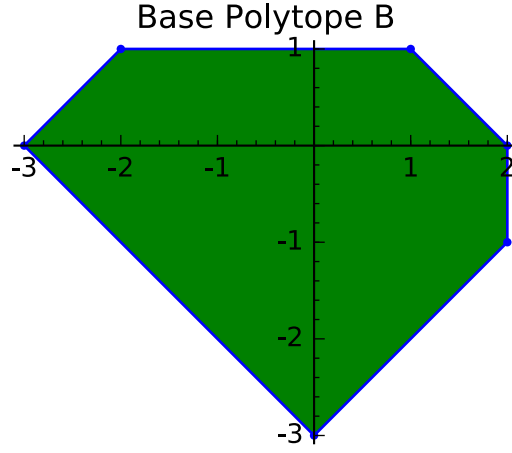

$$(x, y) \mapsto \min(0, -x)$$

$$(x, y) \mapsto \min(0, y)$$

$$(x, y) \mapsto \min\left(\frac{1}{2}x - \frac{1}{2}y - \frac{1}{2}, -y\right)$$

Step (i) obtain a closed form for  $F_{X,\xi}$

For this we have to analytically solve the integral

$$\int_{\square} \langle u, v \rangle \deg \bar{\Phi}(u) e^{\langle u, \xi \rangle} du = \int_{\Delta_0} \langle u', (v, 0) \rangle \cdot e^{\langle u', (\xi, 0) \rangle} du'$$

for  $v$  varying over a basis of  $N_{\mathbb{R}}$ .

#Choose a sufficiently general value for Lambda

Lambda = vector([3,13,19])

# The integral can be solved symbolically:

F1(xi\_1, xi\_2) = intxexp(Polyhedra[1], Lambda, vector([xi\_1, xi\_2, 0]), \vector([1, 0, 0])) . simplify\_full()

F2(xi\_1, xi\_2) = intxexp(Polyhedra[1], Lambda, vector([xi\_1, xi\_2, 0]), \vector([0, 1, 0])) . simplify\_full()

show(F1)

show(F2)

$$(\xi_1, \xi_2) \mapsto -\frac{(4\xi_1^4 e^{(3\xi_1)} - (2((\xi_1 - 2)e^{(4\xi_1)} - (\xi_1 + 1)e^{\xi_1} + 3e^{(3\xi_1)}))\xi_2^4 + 4\xi_1^4 e^{(3\xi_1)} + (2(\xi_1^2 - \xi_1)e^{(4\xi_1)} + \xi_1$$

---


$$(\xi_1, \xi_2) \mapsto - \frac{(6 \xi_1^4 \xi_2 e^{(3 \xi_1)} - 6 \xi_1^2 \xi_2^3 e^{(3 \xi_1)} + 2 \xi_1^4 e^{(3 \xi_1)} - 6 \xi_1^2 \xi_2^2 e^{(3 \xi_1)} - (\xi_2^5 (2 e^{(4 \xi_1)} - 3 e^{(3 \xi_1)} + e^{\xi_1}) - 2 \xi_1^4 \xi_2 e^{(3 \xi_1)}))}{(6 \xi_1^4 \xi_2 e^{(3 \xi_1)} - 6 \xi_1^2 \xi_2^3 e^{(3 \xi_1)} + 2 \xi_1^4 e^{(3 \xi_1)} - 6 \xi_1^2 \xi_2^2 e^{(3 \xi_1)} - (\xi_2^5 (2 e^{(4 \xi_1)} - 3 e^{(3 \xi_1)} + e^{\xi_1}) - 2 \xi_1^4 \xi_2 e^{(3 \xi_1)}))}$$

Step (ii) find an estimate for the soliton candidate vector field  $\xi$ .

We identify a small closed rectangle containing our estimate such that  $\nabla_n G > 0$  for any outer normal of this rectangle, where  $G(\xi) = \int_{\square} \langle u, v \rangle \deg \bar{\Phi}(u) e^{\langle u, \xi \rangle} du$ . This and uniqueness guarantee our candidate lies within the rectangle.

```
#numerically finding an estimate
from scipy import optimize

def FF(x):
    return [F1(x[0], x[1]), F2(x[0], x[1])]
sol=optimize.root(FF, [0.2, 0.5])
x0=sol.x

#We hope xi lies in the square with centre x0 and side length 2e, \
    where:
e = 0.00001

xi_RIF=[RIF(x0[0]-e, x0[0]+e), RIF(x0[1]-e, x0[1]+e)]

#We use interval arithmetic to check positivity of $ \nabla_n G $ on \
    the boundary of the square. We check line segments along the \
    boundary of length 2e/N.
N=2300

if all([RIF(F1(x0[0]+e, RIF(x0[1]-e+i*(2*e/N), x0[1]-e+(i+1)*(2*e/N))) \
    ) > 0
        for i in range(N)]):
    if all([RIF(-F1(x0[0]-e, RIF(x0[1]-e+i*(2*e/N), x0[1]-e+(i+1)*(2*e \
    /N)))) > 0
            for i in range(N)]):
        if all([RIF(F2(RIF(x0[0]-e+i*(2*e/N), x0[0]-e+(i+1)*(2*e/N)), \
    x0[1]+e)) > 0 for i in range(N)]):
            if all([RIF(-F2(RIF(x0[0]-e+i*(2*e/N), x0[0]-e+(i+1)*(2*e \
    /N)), x0[1]-e)) > 0 for i in range(N)]):
                print "There is a root in"
                print xi_RIF[0].str(style="brackets"), "x", xi_RIF[1]. \
    str(style="brackets")
```

There is a root in

$[0.26616785810574 \dots 0.26618785810616] \times [0.67163062513918 \dots 0.67165062513960]$

Step (iii) & (iv) obtain closed forms for  $DF_{\xi}(X_{y,0,1})$  and plug in the estimate for  $\xi$

---

For this we first have to symbolically solve the integrals

$$h_y(\xi) := \text{vol}(\Delta_y) \cdot \text{DF}_\xi(\mathcal{X}_{y,0,1}) = \int_{\Delta_y} \langle u, (0, 0, 1) \rangle e^{\langle u, (\xi, 0) \rangle} du$$

for every (admissible) choice of  $y \in \mathbb{P}^1$  and then plug in the estimate for  $\xi$  into the resulting expression.

```
#storage for the functions h_y and for the values h_y(xi) (as \
    intervals)
Ih=[]

print "lower bounds for DF invariants"
for P in Polyhedra:
    h(xi_1,xi_2) = intxexp(P,Lambda,vector([xi_1,xi_2,0]),vector\
([0,0,1])).simplify_full()
    DF = RIF(h(*xi_RIF))
    Ih.append(DF)
    print(DF.lower())

if all([h > 0 for h in Ih]):
    print("Threefold is stable!")
else:
    if any([h <= 0 for h in Ih]):
        print("Threefold is not stable!")

        print("negative upper bounds for DF invariant:")# print \
upper bound for destabilising DF value
        if Ih[0] <= 0: print(Ih[0].upper())
        if Ih[1] <= 0: print(Ih[1].upper())
        if Ih[2] <= 0: print(Ih[2].upper())
        if Ih[3] <= 0: print(Ih[3].upper())
    else:
        print("Cannot determine stability")
        # Note, that "not a > 0" does not imply "a <= 0" for \
intervals
```

lower bounds for DF invariants

1.2766364162

1.8401675971

0.10047917120

3.4443270408

Threefold is stable!

---

No. 3.24

The combinatorial data is given by  $\square = \text{conv}((-2, 0), (-2, 1), (1, 1), (2, 0), (2, -2), (0, -2))$  and  $\Phi_0(x, y) = \min\{0, x\}$ ,  $\Phi_1(x, y) = \min\{0, y\}$ ,  $\Phi_\infty(x, y) = \min\{0, -x - y\}$ .

---

```

# We are working with interval arithmetic with precision of 60 bit
# this fixes the precision e.g. for evaluations of exponential \
  functions
RIF=RealIntervalField(16)

# The base polytope
B=Polyhedron(vertices = [[-2,0],[-2,1],[1,1],[2,0],[2,-2],[0,-2]])

# 3 PL functions on B. If phi is the minimum of affine functions of \
  the form  $F(x,y) = a + b*x + c*y$  we represent phi as
# the transpose of the matrix with rows [a,b,c].

Phi1 = matrix(QQ,[[0,0,0],[0,1,0]].transpose()
Phi2 = matrix(QQ,[[0,0,0],[0,0,1]].transpose()
Phi3 = matrix(QQ,[[0,0,0],[0,-1,-1]].transpose()

PLfunctions = [Phi1,Phi2,Phi3]

# Form list of degeneration polyhedra
Polyhedra = degenerations(PLfunctions,B)

print "The combinatorial data"

graphic = B.plot().show(figsize=[3,3],title='Base Polytope B')

x,y = var('x,y')
r = vector([1,x,y])

for Phi in PLfunctions:
    if Phi.transpose().nrows() > 1:
        f(x,y) = min_symbolic(*list(r*Phi))
    else:
        f(x,y) = list(r*Phi)[0]
    print ' '
    show(f)

```

The combinatorial data

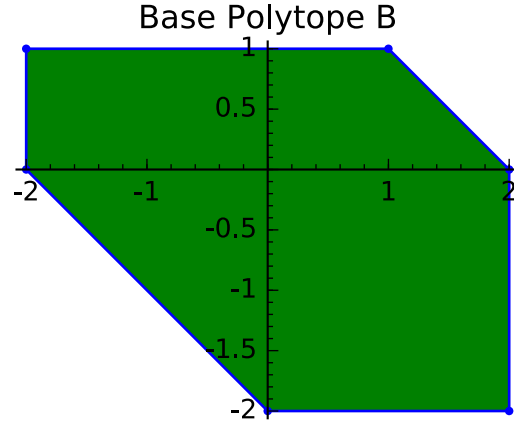

$$(x, y) \mapsto \min(0, x)$$

$$(x, y) \mapsto \min(0, y)$$

$$(x, y) \mapsto \min(0, -x - y)$$

Step (i) obtain a closed form for  $F_{X,\xi}$

For this note, that  $\begin{pmatrix} -1 & -1 \\ 1 & 0 \end{pmatrix}$  is a symmetry of the combinatorial data. Hence, we have  $\xi = (0, \xi_2)$ . We have to analytically solve the integral

$$\int_{\square} \langle u, v \rangle \deg \bar{\Phi}(u) e^{\langle u, \xi \rangle} du = \int_{\Delta_0} \langle u', (v, 0) \rangle \cdot e^{\langle u', (\xi, 0) \rangle} du'$$

for  $v$  varying over a basis of  $N_{\mathbb{R}}$ .

#Choose a sufficiently general value for lambda

Lambda = vector([1,3,13])

# Analytic solution of the integral

F1(xi\_2) = intxexp(Polyhedra[0], Lambda, vector([0, xi\_2, 0]), vector([1, 0, 0])).simplify\_full()

F2(xi\_2) = intxexp(Polyhedra[0], Lambda, vector([0, xi\_2, 0]), vector([0, 1, 0])).simplify\_full()

show(vector([F1, F2]))

$$\xi_2 \mapsto \left( -\frac{((\xi_2^2 - 2)e^{(3\xi_2)} - 2\xi_2 + 4e^{(2\xi_2)} - 2)e^{(-2\xi_2)}}{\xi_2^3}, \frac{2((\xi_2^2 - 2)e^{(3\xi_2)} - 2\xi_2 + 4e^{(2\xi_2)} - 2)e^{(-2\xi_2)}}{\xi_2^3} \right)$$

Step (ii) find an estimate for the soliton candidate vector field  $\xi$ .

# Choose upper and lower bound and

# hope that the exact solution lies in between

lower = 0.434747

upper = 0.434757

---

```

#define a real value xi_RIF between xi_1 and xi_2
# representing the exact solution.
xi_RIF = RIF(lower , upper)

# Check whether Intermediate value theorem guarantees a zero beween
# lower and upper, i.e evaluate F2 at lower and upper using interval\
arithmetic.
if RIF(F2(lower)) < 0 and RIF(F2(upper)) > 0:
    print "Interval containing solution:", xi_RIF.str(style='\
brackets')

```

Step (iii) & (iv) obtain closed forms for  $DF_\xi(X_{y,0,1})$  and plug in the estimate for  $\xi$   
For this we first have to symbolically solve the integrals

$$h_y(\xi) := \text{vol}(\Delta_y) \cdot DF_\xi(\mathcal{X}_{y,0,1}) = \int_{\Delta_y} \langle u, (0, 0, 1) \rangle e^{\langle u, (\xi, 0) \rangle} du$$

for every (admissible) choice of  $y \in \mathbb{P}^1$  and then plug in the estimate for  $\xi$  into the resulting expression.

```

#storage for the functions h_y
H=[]
#storage for values h_y(xi) (as intervals)
Ih=[]

#Symbollically solving integrals using Barvinok method
for P in Polyhedra:
    h(xi_2) = intxexp(P,Lambda,vector([0,xi_2,0]),vector([0,0,1])).\
simplify_full()
    DF=RIF(h(xi_RIF))
    H.append(h); Ih.append(DF)
    show(h(xi_2) >= DF.lower())

if all([h > 0 for h in Ih]):
    print("Threefold is stable!")
else:
    if any([h <= 0 for h in Ih]):
        print("Threefold is not stable!")

    # print upper bound for destabilising DF value
    if Ih[0] <= 0: show(H[0](xi_2) <= Ih[0].upper())
    if Ih[1] <= 0: show(H[1](xi_2) <= Ih[1].upper())
    if Ih[2] <= 0: show(H[2](xi_2) <= Ih[2].upper())
    if Ih[3] <= 0: show(H[3](xi_2) <= Ih[3].upper())
    else:
        print("Cannot determine stability")
        # Note, that "not a > 0" does not imply "a <= 0" for \
intervals

```

---


$$\frac{2((\xi_2 - 1)e^{(2\xi_2)} + \xi_2 + 1)e^{(-2\xi_2)}}{\xi_2^3} \geq 0.8784$$

$$\frac{(12\xi_2^2 - (7\xi_2^3 + 3\xi_2^2 - 6\xi_2 + 6)e^{(3\xi_2)} + 12(2\xi_2^2 - 2\xi_2 + 1)e^{(2\xi_2)} + 12\xi_2 - 6)e^{(-2\xi_2)}}{6\xi_2^4} \geq 1.288$$

$$\frac{2((\xi_2 - 1)e^{(2\xi_2)} + \xi_2 + 1)e^{(-2\xi_2)}}{\xi_2^3} \geq 0.8784$$

$$\frac{(12\xi_2^2 + (7\xi_2^3 + 3\xi_2^2 - 6\xi_2 + 6)e^{(3\xi_2)} + 12\xi_2 - 12e^{(2\xi_2)} + 6)e^{(-2\xi_2)}}{6\xi_2^4} \geq 3.049$$

Threefold is stable!

---

No. 4.5\*

The combinatorial data is given by  $\square = \text{conv}((-2, 1), (-3, 3), (-2, 3), (1, -2), (3, -3), (3, -2))$  and  $\Phi_0(x, y) = \min\{0, \frac{-x-1}{2}\}$ ,  $\Phi_1(x, y) = \min\{0, \frac{-y-1}{2}\}$ ,  $\Phi_\infty(x, y) = \min\{0, x + y\}$ .

```
# We are working with interval arithmetic with precision of 60 bit
# this fixes the precision e.g. for evaluations of exponential \
  functions
RIF=RealIntervalField(16)

# The base polytope
B=Polyhedron(vertices = [[-2, 1], [-3, 3], [-2, 3], [1, -2], [3, -3], [3, -2]])

# 3 PL functions on B. If phi is the minimum of affine functions of \
  the form F(x,y) = a + b*x + c*y we represent phi as
# the transpose of the matrix with rows [a,b,c].

Phi1 = matrix(QQ, [[0, 0, 0], [-1/2, -1/2, 0]]).transpose()
Phi2 = matrix(QQ, [[0, 0, 0], [-1/2, 0, -1/2]]).transpose()
Phi3 = matrix(QQ, [[0, 0, 0], [0, 1, 1]]).transpose()

PLfunctions = [Phi1, Phi2, Phi3]

# Form list of degeneration polyhedra
Polyhedra = degenerations(PLfunctions, B)

print "The combinatorial data"

graphic = B.plot().show(figsize=[3,3], title='Base Polytope B')

x,y = var('x,y')
r = vector([1,x,y])
```

---

```

for Phi in PLfunctions:
    if Phi.transpose().nrows() > 1:
        f(x,y) = min_symbolic(*list(r*Phi))
    else:
        f(x,y) = list(r*Phi)[0]
    print ' '
    show(f)

```

The combinatorial data

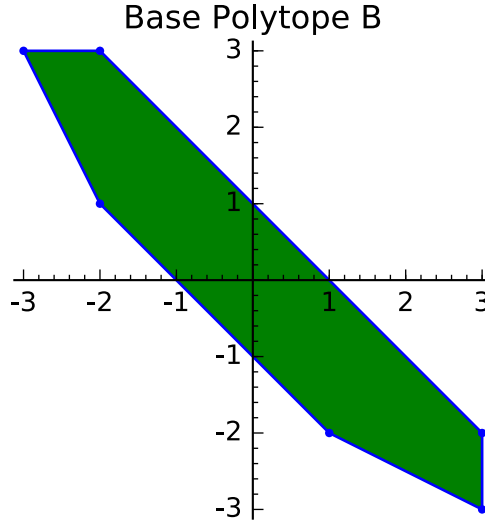

$$(x, y) \mapsto \min \left( 0, -\frac{1}{2}x - \frac{1}{2} \right)$$

$$(x, y) \mapsto \min \left( 0, -\frac{1}{2}y - \frac{1}{2} \right)$$

$$(x, y) \mapsto \min(0, x + y)$$

Step (i) obtain a closed form for  $F_{X,\xi}$

For this note, that  $\begin{pmatrix} 0 & 1 \\ 1 & 0 \end{pmatrix}$  is a symmetry of the combinatorial data. Hence, we have  $\xi = (\xi_1, \xi_1)$   
 We have to analytically solve the integral

$$\int_{\square} \langle u, v \rangle \deg \bar{\Phi}(u) e^{\langle u, \xi \rangle} du = \int_{\Delta_0} \langle u', (v, 0) \rangle \cdot e^{\langle u', (\xi, 0) \rangle} du'$$

for  $v$  varying over a basis of  $N_{\mathbb{R}}$ .

#Choose a sufficiently general value for lambda

Lambda = vector([1,3,13])

# Analytic solution of the integral

F1(xi\_1) = intxexp(Polyhedra[0], Lambda, vector([xi\_1, xi\_1, 0]), vector([1, -1, 0])).simplify\_full()

F2(xi\_1) = intxexp(Polyhedra[0], Lambda, vector([xi\_1, xi\_1, 0]), vector([1, 1, 0])).simplify\_full()

---

```
show(vector([F1,F2]))
```

$$\xi_1 \mapsto \left(0, \frac{(\xi_1^3 - \xi_1^2 + 2(\xi_1^3 - 2\xi_1)e^{(2\xi_1)} + 6(2\xi_1 - 1)e^{\xi_1} - 2\xi_1 + 6)e^{(-\xi_1)}}{\xi_1^4}\right)$$

Step (ii) find an estimate for the soliton candidate vector field  $\xi$ .

```
# Choose upper and lower bound and
# hope that the exact solution lies in between
find_root(F2,-10,10)
lower = -0.31044
upper = -0.31043

#define a real value xi_RIF between xi_1 and xi_2
# representing the exact solution.
xi_RIF = RIF(lower, upper)

# Check whether Intermediate value theorem guarantees a zero between
# lower and upper, i.e evaluate F2 at lower and upper using interval\
arithmetic.
if RIF(F2(lower)) < 0 and RIF(F2(upper)) > 0:
    print "Interval containing solution:", xi_RIF.str(style='\
brackets')
-0.31043117071394555
Interval containing solution: [-0.310441 .. -0.310424]
```

Step (iii) & (iv) obtain closed forms for  $DF_\xi(X_{y,0,1})$  and plug in the estimate for  $\xi$   
For this we first have to symbolically solve the integrals

$$h_y(\xi) := \text{vol}(\Delta_y) \cdot DF_\xi(X_{y,0,1}) = \int_{\Delta_y} \langle u, (0, 0, 1) \rangle e^{\langle u, (\xi, 0) \rangle} du$$

for every choice of  $y \in \mathbb{P}^1$  and then plug in the estimate for  $\xi$  into the resulting expression.

```
#storage for the functions h_y
H=[]
#storage for values h_y(xi) (as intervals)
Ih=[]

#Symbolically solving integrals using Barvinok method
for P in Polyhedra:
    h(xi_2) = intxexp(P,Lambda,vector([xi_2,xi_2,0]),vector([0,0,1])\
).simplify_full()
    DF=RIF(h(xi_RIF))
    H.append(h); Ih.append(DF)
    show(h(xi_2) >= DF.lower())

if all([h > 0 for h in Ih]):
    print("Threefold is stable!")
```

---

```

else:
    if any([h <= 0 for h in Ih]):
        print("Threefold is not stable!")

        # print upper bound for destabilising DF value
        if Ih[0] <= 0: show(H[0](xi_2) <= Ih[0].upper())
        if Ih[1] <= 0: show(H[1](xi_2) <= Ih[1].upper())
        if Ih[2] <= 0: show(H[2](xi_2) <= Ih[2].upper())
        if Ih[3] <= 0: show(H[3](xi_2) <= Ih[3].upper())
    else:
        print("Cannot determine stability")
        # Note, that "not a > 0" does not imply "a <= 0" for \
intervals

$$-\frac{(\xi_2^3 - \xi_2^2 - 2(2\xi_2^2 - 4\xi_2 + 3)e^{\xi_2} - 2\xi_2 + 6)e^{(-\xi_2)}}{2\xi_2^4} \geq 0.5108$$


$$-\frac{(\xi_2^3 - \xi_2^2 - 2(2\xi_2^2 - 4\xi_2 + 3)e^{\xi_2} - 2\xi_2 + 6)e^{(-\xi_2)}}{2\xi_2^4} \geq 0.5108$$


$$\frac{(5\xi_2^3 + 9\xi_2^2 + (37\xi_2^3 + 27\xi_2^2 - 18\xi_2 + 6)e^{(2\xi_2)} - 24(6\xi_2^2 - 8\xi_2 + 5)e^{\xi_2} - 66\xi_2 + 114)e^{(-\xi_2)}}{24\xi_2^4} \geq$$

2.318

$$-\frac{(19\xi_2^3 - 33\xi_2^2 - (37\xi_2^3 + 27\xi_2^2 - 18\xi_2 + 6)e^{(2\xi_2)} + 24(2\xi_2^2 - 1)e^{\xi_2} + 18\xi_2 + 30)e^{(-\xi_2)}}{24\xi_2^4} \geq 3.489$$

Threefold is stable!

```

---

No. 4.8

The combinatorial data is given by  $\square = \text{conv}((-2, 0), (-1, 1), (1, 1), (2, 0), (2, -1), (-2, -1))$  and  $\Phi_0(x, y) = \min\{0, x\}$ ,  $\Phi_1(x, y) = \min\{0, -x\}$ ,  $\Phi_\infty(x, y) = \min\{0, -y\}$ .

```

# We are working with interval arithmetic with precision of 60 bit
# this fixes the precision e.g. for evaluations of exponential \
functions
RIF=RealIntervalField(16)

# The base polytope
B=Polyhedron(vertices = [[-2, 0], [-1, 1], [1, 1], [2, 0], [2, -1], [-2, -1]])

# 3 PL functions on B. If phi is the minimum of affine functions of \
the form F(x,y) = a + b*x + c*y we represent phi as
# the transpose of the matrix with rows [a,b,c].

Phi1 = matrix(QQ, [[0, 0, 0], [0, 1, 0]]).transpose()
Phi2 = matrix(QQ, [[0, 0, 0], [0, -1, 0]]).transpose()
Phi3 = matrix(QQ, [[0, 0, 0], [0, 0, -1]]).transpose()

PLfunctions = [Phi1, Phi2, Phi3]

```

---

```

# Form list of degeneration polyhedra
Polyhedra = degenerations(PLfunctions,B)

print "The combinatorial data"

graphic = B.plot().show(figsize=[3,3],title='Base Polytope B')

x,y = var('x,y')
r = vector([1,x,y])

for Phi in PLfunctions:
    if Phi.transpose().nrows() > 1:
        f(x,y) = min_symbolic(*list(r*Phi))
    else:
        f(x,y) = list(r*Phi)[0]
    print ' '
    show(f)

```

The combinatorial data

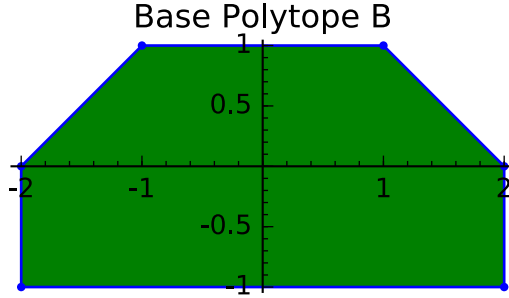

$$(x, y) \mapsto \min(0, x)$$

$$(x, y) \mapsto \min(0, -x)$$

$$(x, y) \mapsto \min(0, -y)$$

Step (i) obtain a closed form for  $F_{X,\xi}$

For this note, that  $\begin{pmatrix} -1 & 0 \\ 0 & 1 \end{pmatrix}$  is a symmetry of the combinatorial data. Hence we have  $\xi = (0, \xi_2)$ . We have to analytically solve the integral

$$\int_{\square} \langle u, v \rangle \deg \bar{\Phi}(u) e^{\langle u, \xi \rangle} du = \int_{\Delta_0} \langle u', (v, 0) \rangle \cdot e^{\langle u', (\xi, 0) \rangle} du'$$

for  $v$  varying over a basis of  $N_{\mathbb{R}}$ .

---

#Choose a sufficiently general value for lambda

---

```
Lambda = vector([1,5,13])
```

```
# Analytic solution of the integral
```

```
F1(xi_2) = intxexp(Polyhedra[0], Lambda, vector([0, xi_2, 0]), vector\
([1, 0, 0])).simplify_full()
F2(xi_2) = intxexp(Polyhedra[0], Lambda, vector([0, xi_2, 0]), vector\
([0, 1, 0])).simplify_full()
```

```
show(vector([F1, F2]))
```

$$\xi_2 \mapsto \left( 0, \frac{(4\xi_2^3 + 4\xi_2^2 + (\xi_2^3 + \xi_2^2 - 2\xi_2 - 6)e^{(2\xi_2)} + 2(4\xi_2 + 3)e^{\xi_2})e^{(-\xi_2)})}{\xi_2^4} \right)$$

Step (ii) find an estimate for the soliton candidate vector field  $\xi$ .

```
# Choose upper and lower bound and
```

```
# hope that the exact solution lies in between
```

```
lower = 0.62430
```

```
upper = 0.62431
```

```
#define a real value xi_RIF between xi_1 and xi_2
```

```
# representing the exact solution.
```

```
xi_RIF = RIF(lower, upper)
```

```
# Check whether Intermediate value theorem guarantees a zero between
# lower and upper, i.e evaluate F2 at lower and upper using interval\
arithmetic.
```

```
if RIF(F2(lower)) < 0 and RIF(F2(upper)) > 0:
```

```
    print "Interval containing solution:", xi_RIF.str(style='\
brackets')
```

```
Interval containing solution: [0.624298 .. 0.624314]
```

Step (iii) & (iv) obtain closed forms for  $DF_\xi(X_{y,0,1})$  and plug in the estimate for  $\xi$

For this we first have to symbolically solve the integrals

$$h_y(\xi) := \text{vol}(\Delta_y) \cdot DF_\xi(X_{y,0,1}) = \int_{\Delta_y} \langle u, (0, 0, 1) \rangle e^{\langle u, (\xi, 0) \rangle} du$$

for every choice of  $y \in \mathbb{P}^1$  and then plug in the estimate for  $\xi$  into the resulting expression.

```
#storage for the functions h_y
```

```
H=[]
```

```
#storage for values h_y(xi) (as intervals)
```

```
Ih=[]
```

```
#Symbollically solving integrals using Barvinok method
```

```
for P in Polyhedra:
```

---

```

    h(xi_2) = intxexp(P,Lambda,vector([0,xi_2,0]),vector([0,0,1])).\
simplify_full()
    DF=RIF(h(xi_RIF))
    H.append(h); Ih.append(DF)
    show(h(xi_2) >= DF.lower())

if all([h > 0 for h in Ih]):
    print("Threefold is stable!")
else:
    if any([h <= 0 for h in Ih]):
        print("Threefold is not stable!")

        # print upper bound for destabilising DF value
        if Ih[0] <= 0: show(H[0](xi_2) <= Ih[0].upper())
        if Ih[1] <= 0: show(H[1](xi_2) <= Ih[1].upper())
        if Ih[2] <= 0: show(H[2](xi_2) <= Ih[2].upper())
        if Ih[3] <= 0: show(H[3](xi_2) <= Ih[3].upper())
    else:
        print("Cannot determine stability")
        # Note, that "not a > 0" does not imply "a <= 0" for \
intervals

$$\frac{4\xi_2^2 + (\xi_2^3 + \xi_2^2 - 2\xi_2 - 6)e^{\xi_2} + 8\xi_2 + 6}{2\xi_2^4} \geq 0.6641$$


$$\frac{4\xi_2^2 + (\xi_2^3 + \xi_2^2 - 2\xi_2 - 6)e^{\xi_2} + 8\xi_2 + 6}{2\xi_2^4} \geq 0.6641$$


$$-\frac{(4\xi_2^3 + (\xi_2^3 - 6\xi_2 - 12)e^{(2\xi_2)} + 6(2\xi_2^2 + 3\xi_2 + 2)e^{\xi_2})e^{(-\xi_2)}}{3\xi_2^4} \geq 1.104$$


$$-\frac{(4\xi_2^3 - (2\xi_2^3 + 3\xi_2^2 - 6)e^{(2\xi_2)} - 6(\xi_2 + 1)e^{\xi_2})e^{(-\xi_2)}}{3\xi_2^4} \geq 2.442$$


```

Threefold is stable!
